# Supplementary material for: Microlensing and Variability in the Bulge of M31
Source: arXiv:1009.2115 source file (2010-09-10)
Supplement: Supplementary file 1 [file Appendix.tex]

\chapter{Appendix}
\label{appendix}
In this section are the figures showing the distributions of the variable candidate fit parameters Period and Skewness,
divided into their $16$ sub-categories, ((LT+FTN) data only or (LT+FTN+PA) data, Variable or Mixed fit, Fixed flux amplitude ratio low, medium, high or unfixed) before these groups were rationalised together. In each of the summary plots \ref{Log(P)_all_categories_low_ratio} to \ref{Skewness_all_categories_no_ratio}, the three vertical columns also first divide the data into two parts, for low (0-5 ADU/s) flux amplitudes and higher flux amplitude ratios and then in the third column show the undivided total distributions. This division is made because the most obvious differences in the plotted distributions usually occur between the two groups illustrated; it might be more accurate to say that the low amplitude variables differed from the rest, but they also dominate hugely in number/ADU.

% LOW RATIO
\begin{figure}
\vspace*{4cm}
\center{
  \begin{tabular}{ccc}
% 0-5
\vspace*{5cm}
   \leavevmode
 \includegraphics{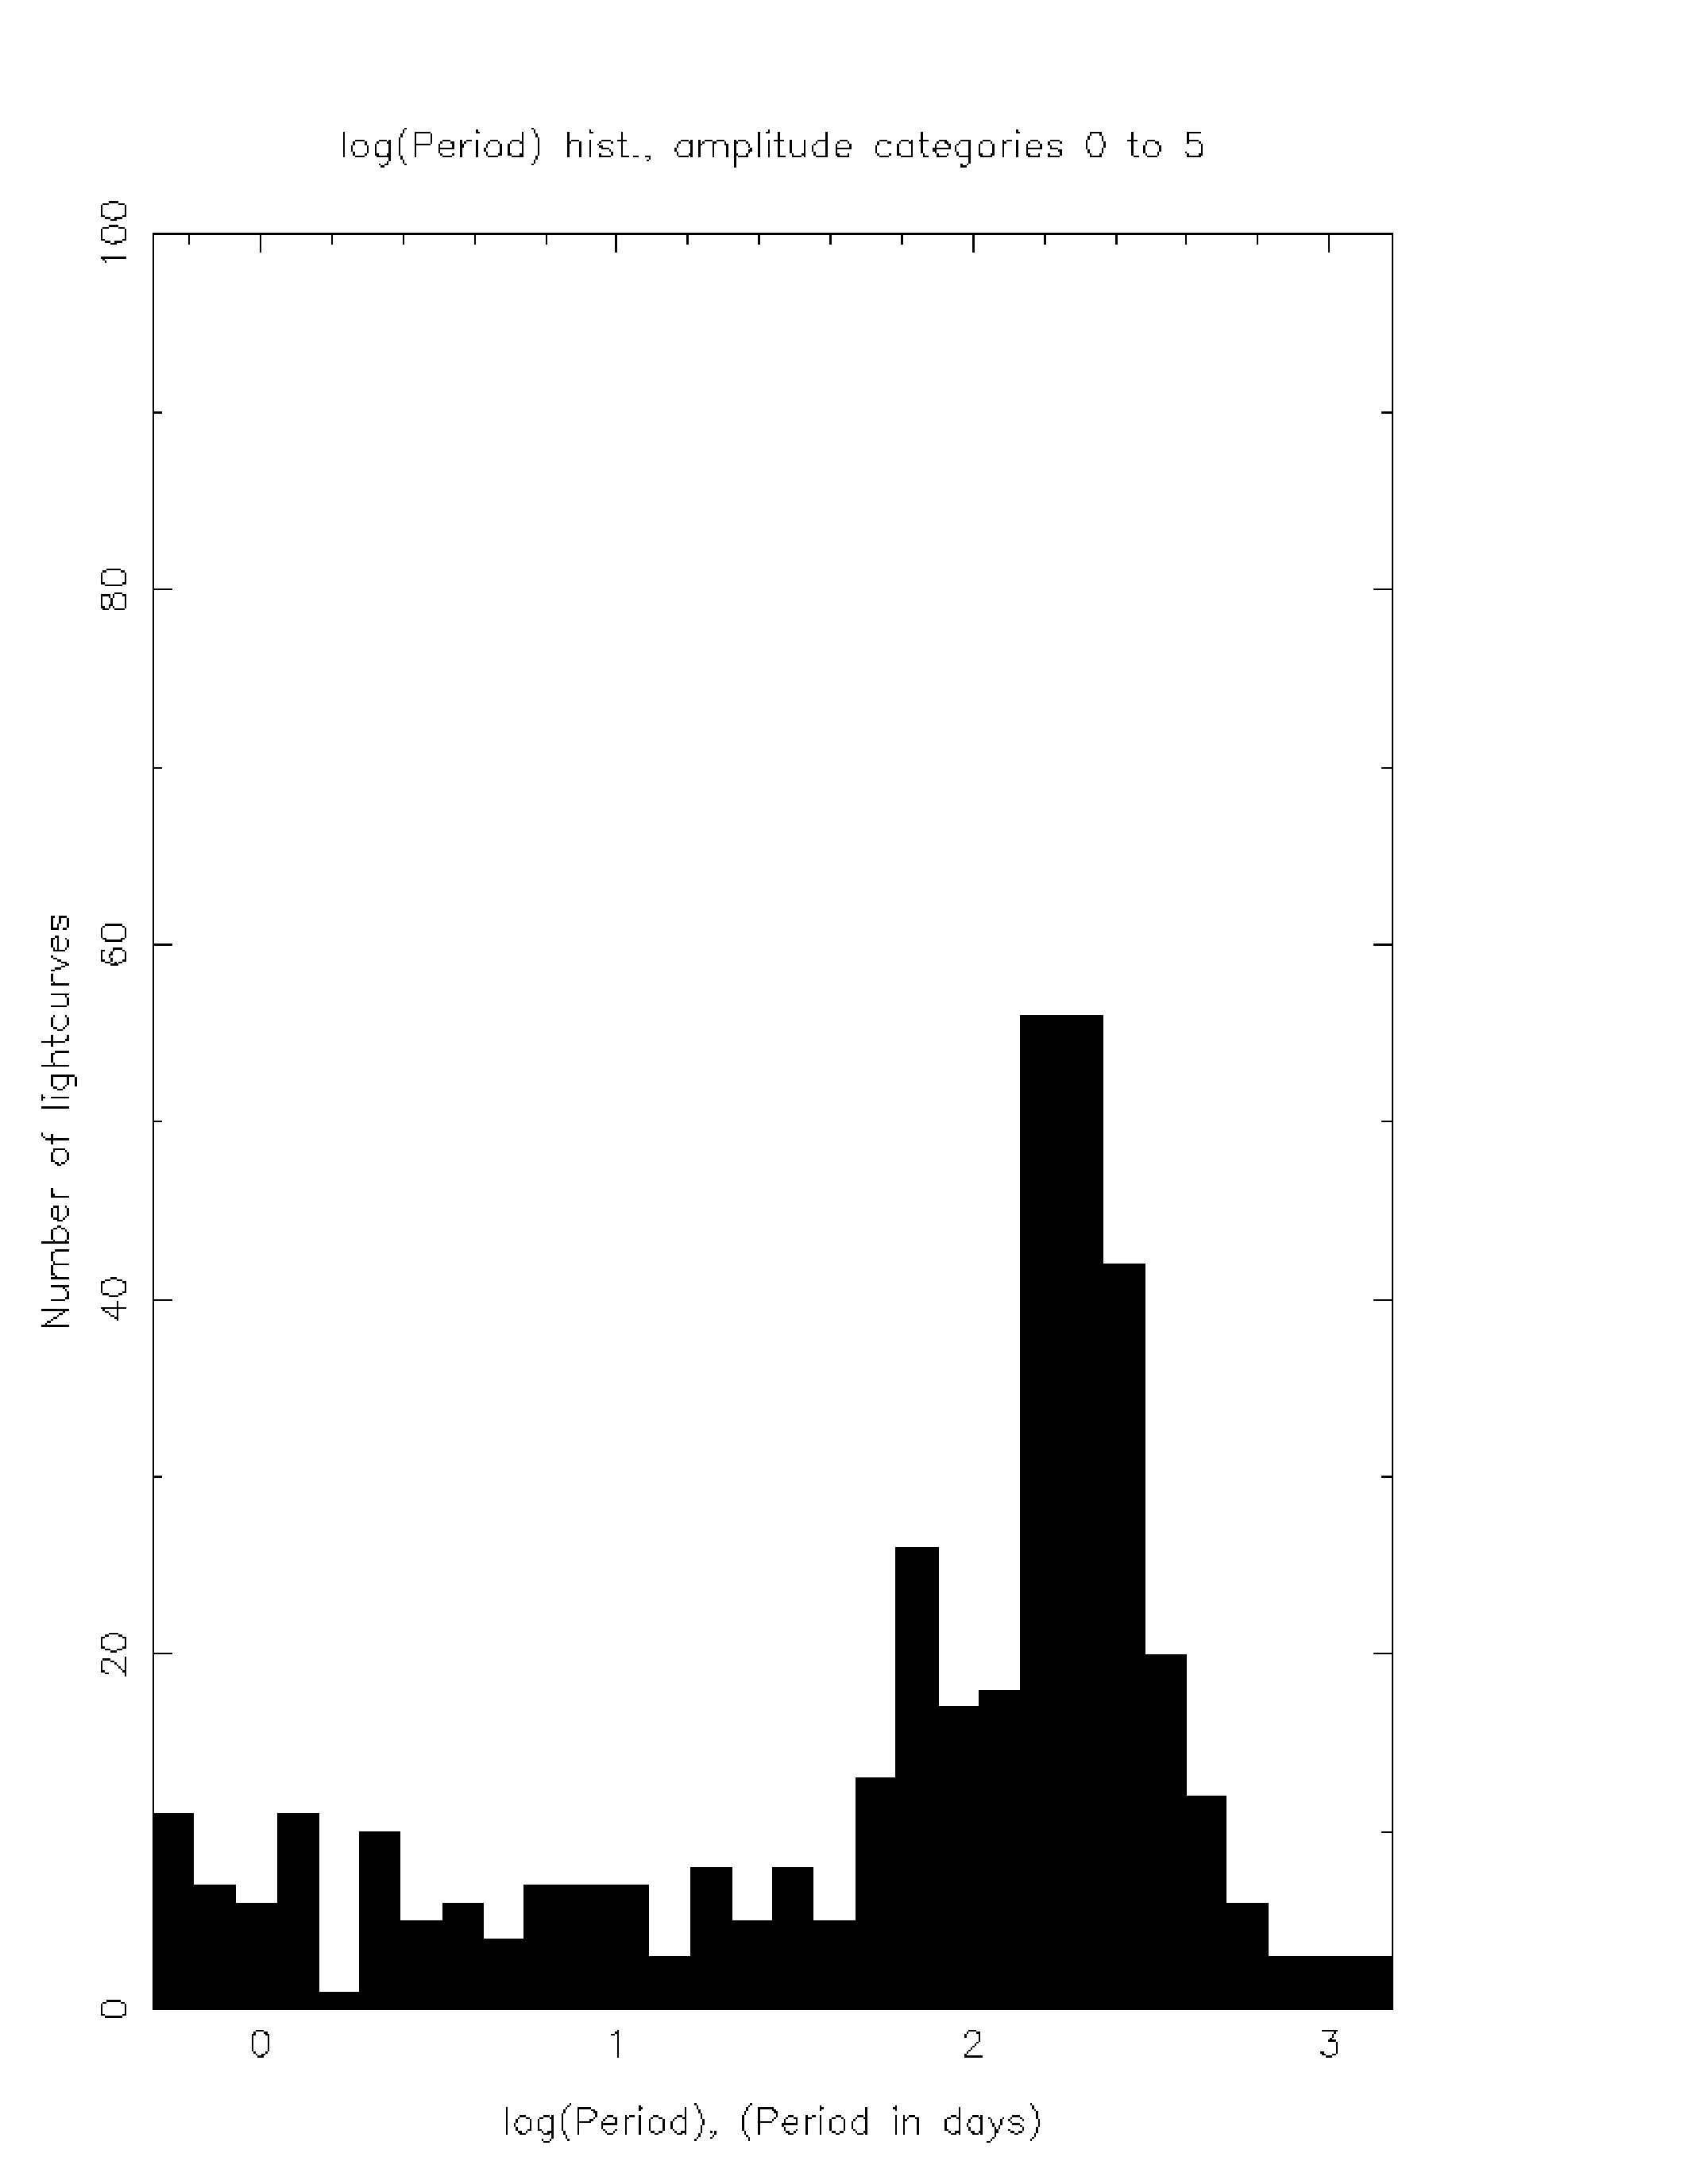} \\
\vspace*{5cm}
   \leavevmode
 \includegraphics{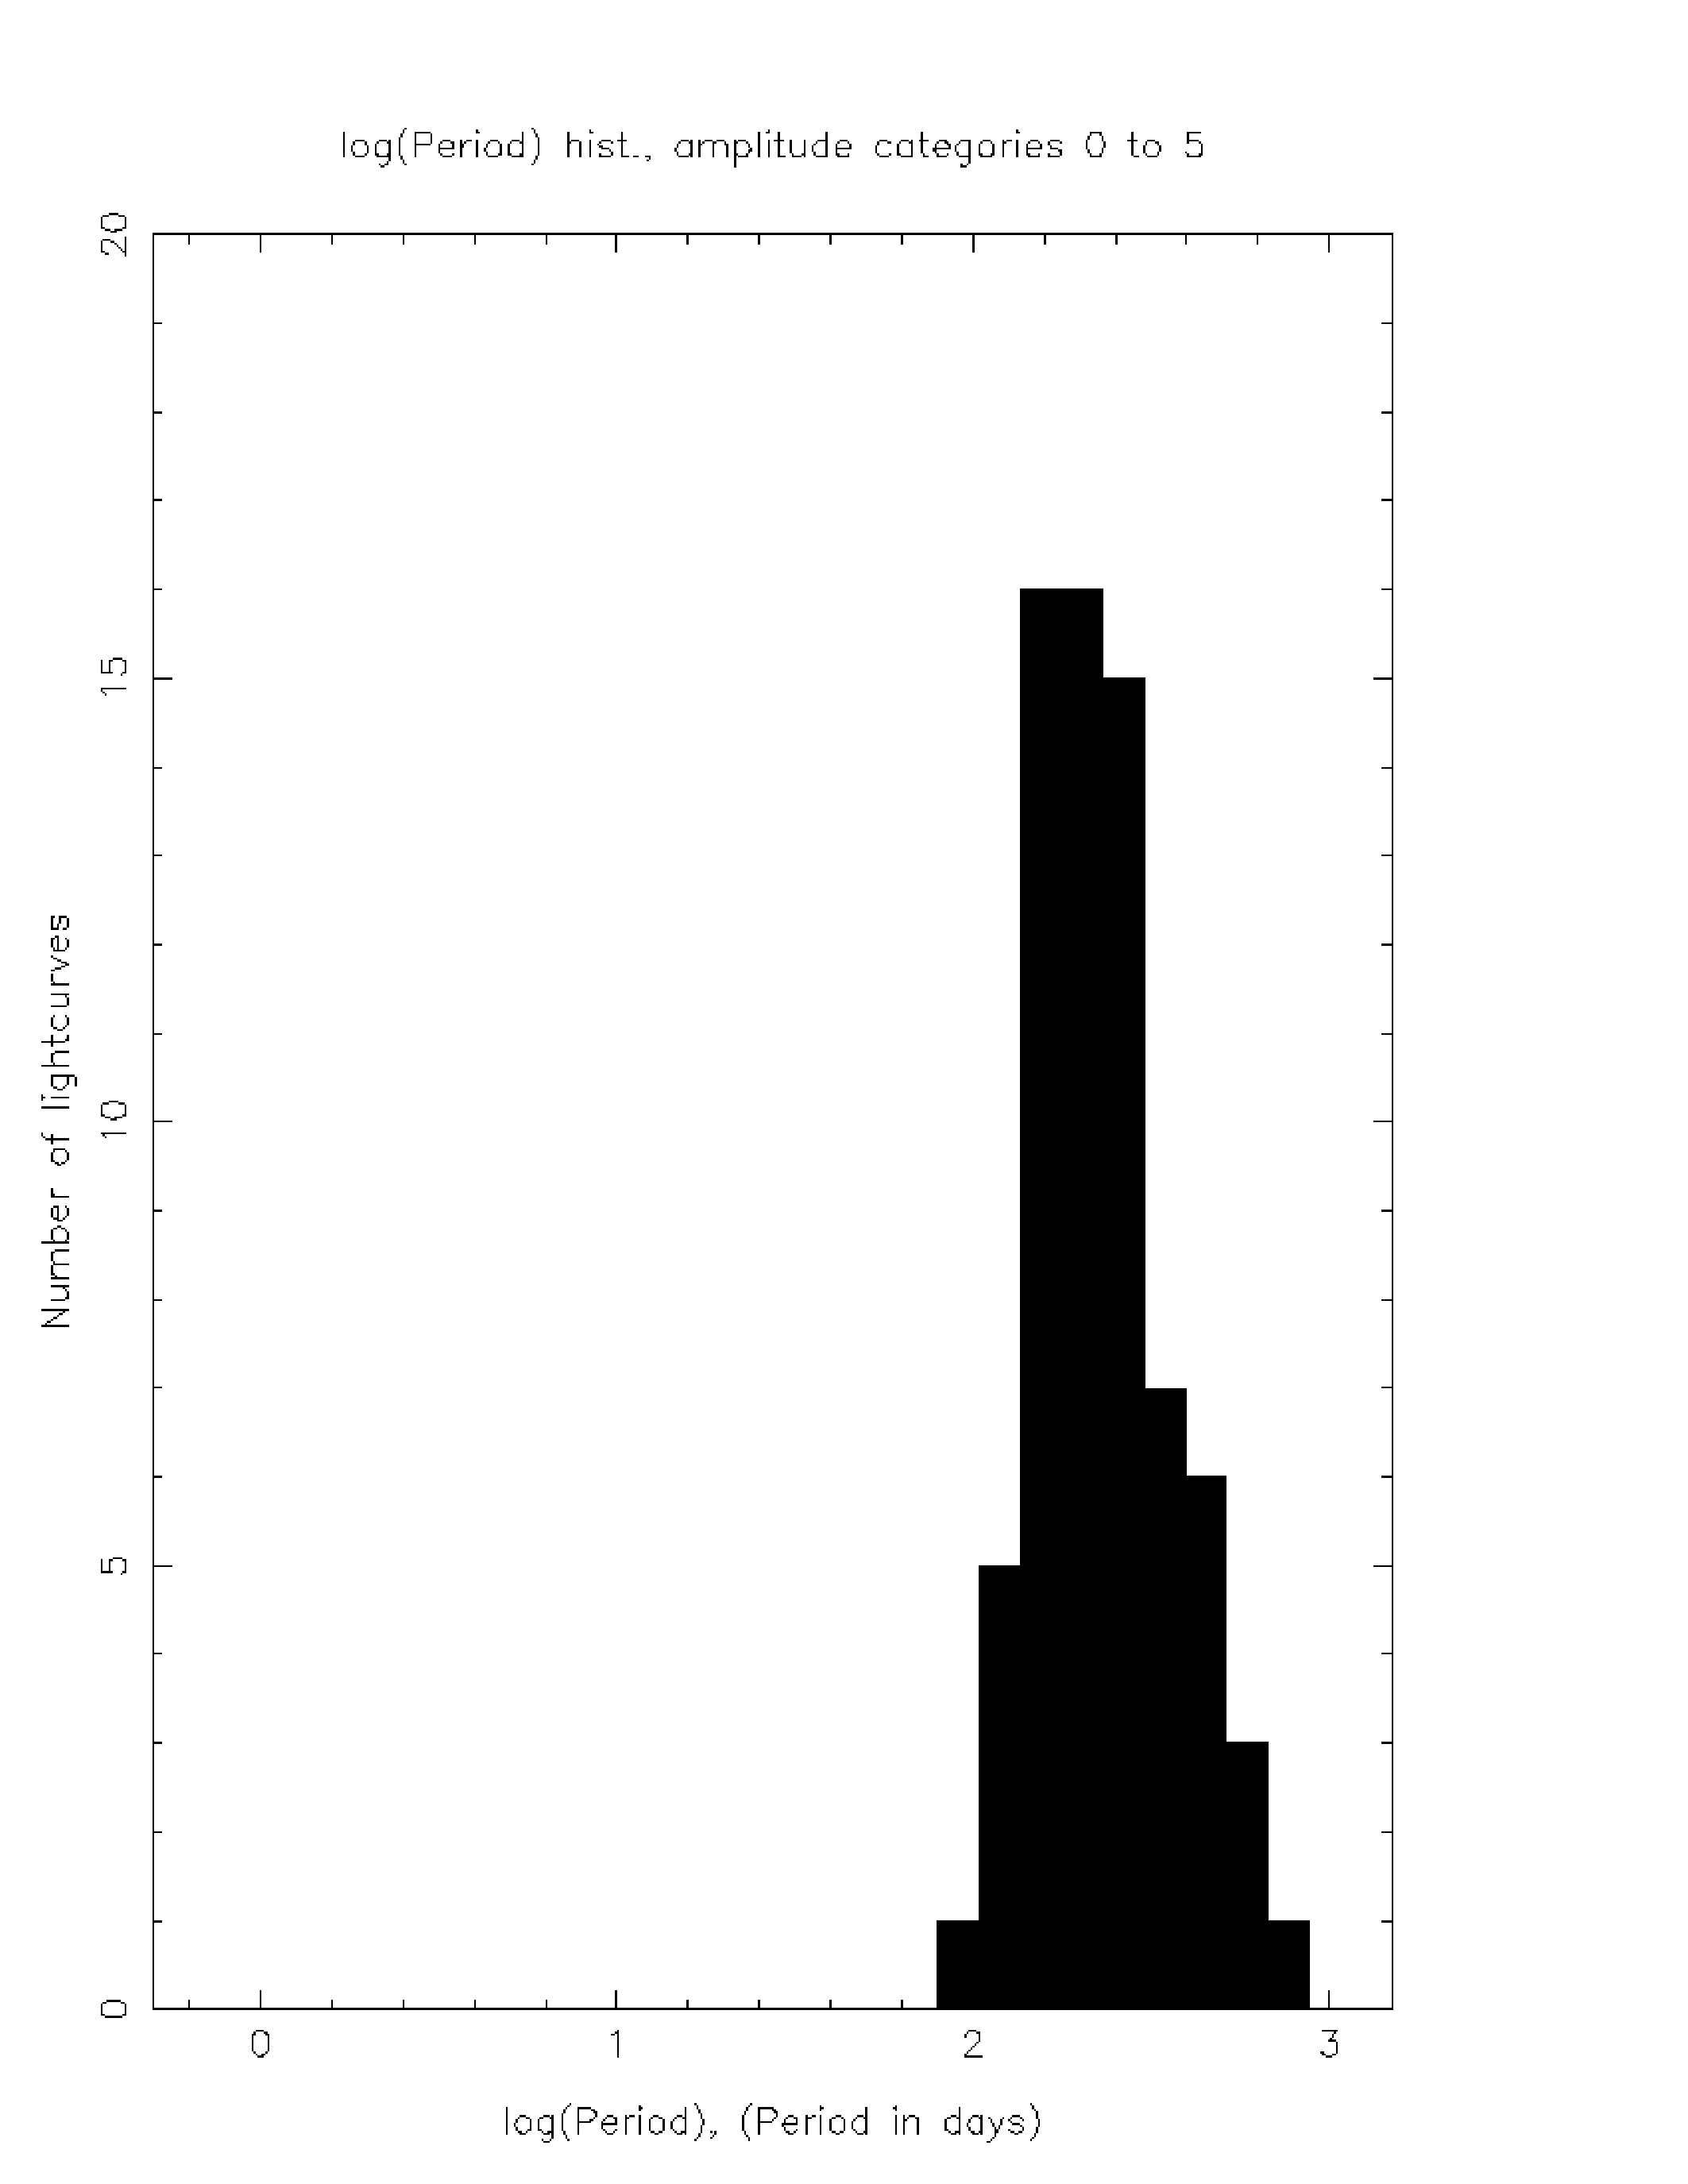} \\
\vspace*{5cm}
   \leavevmode
 \includegraphics{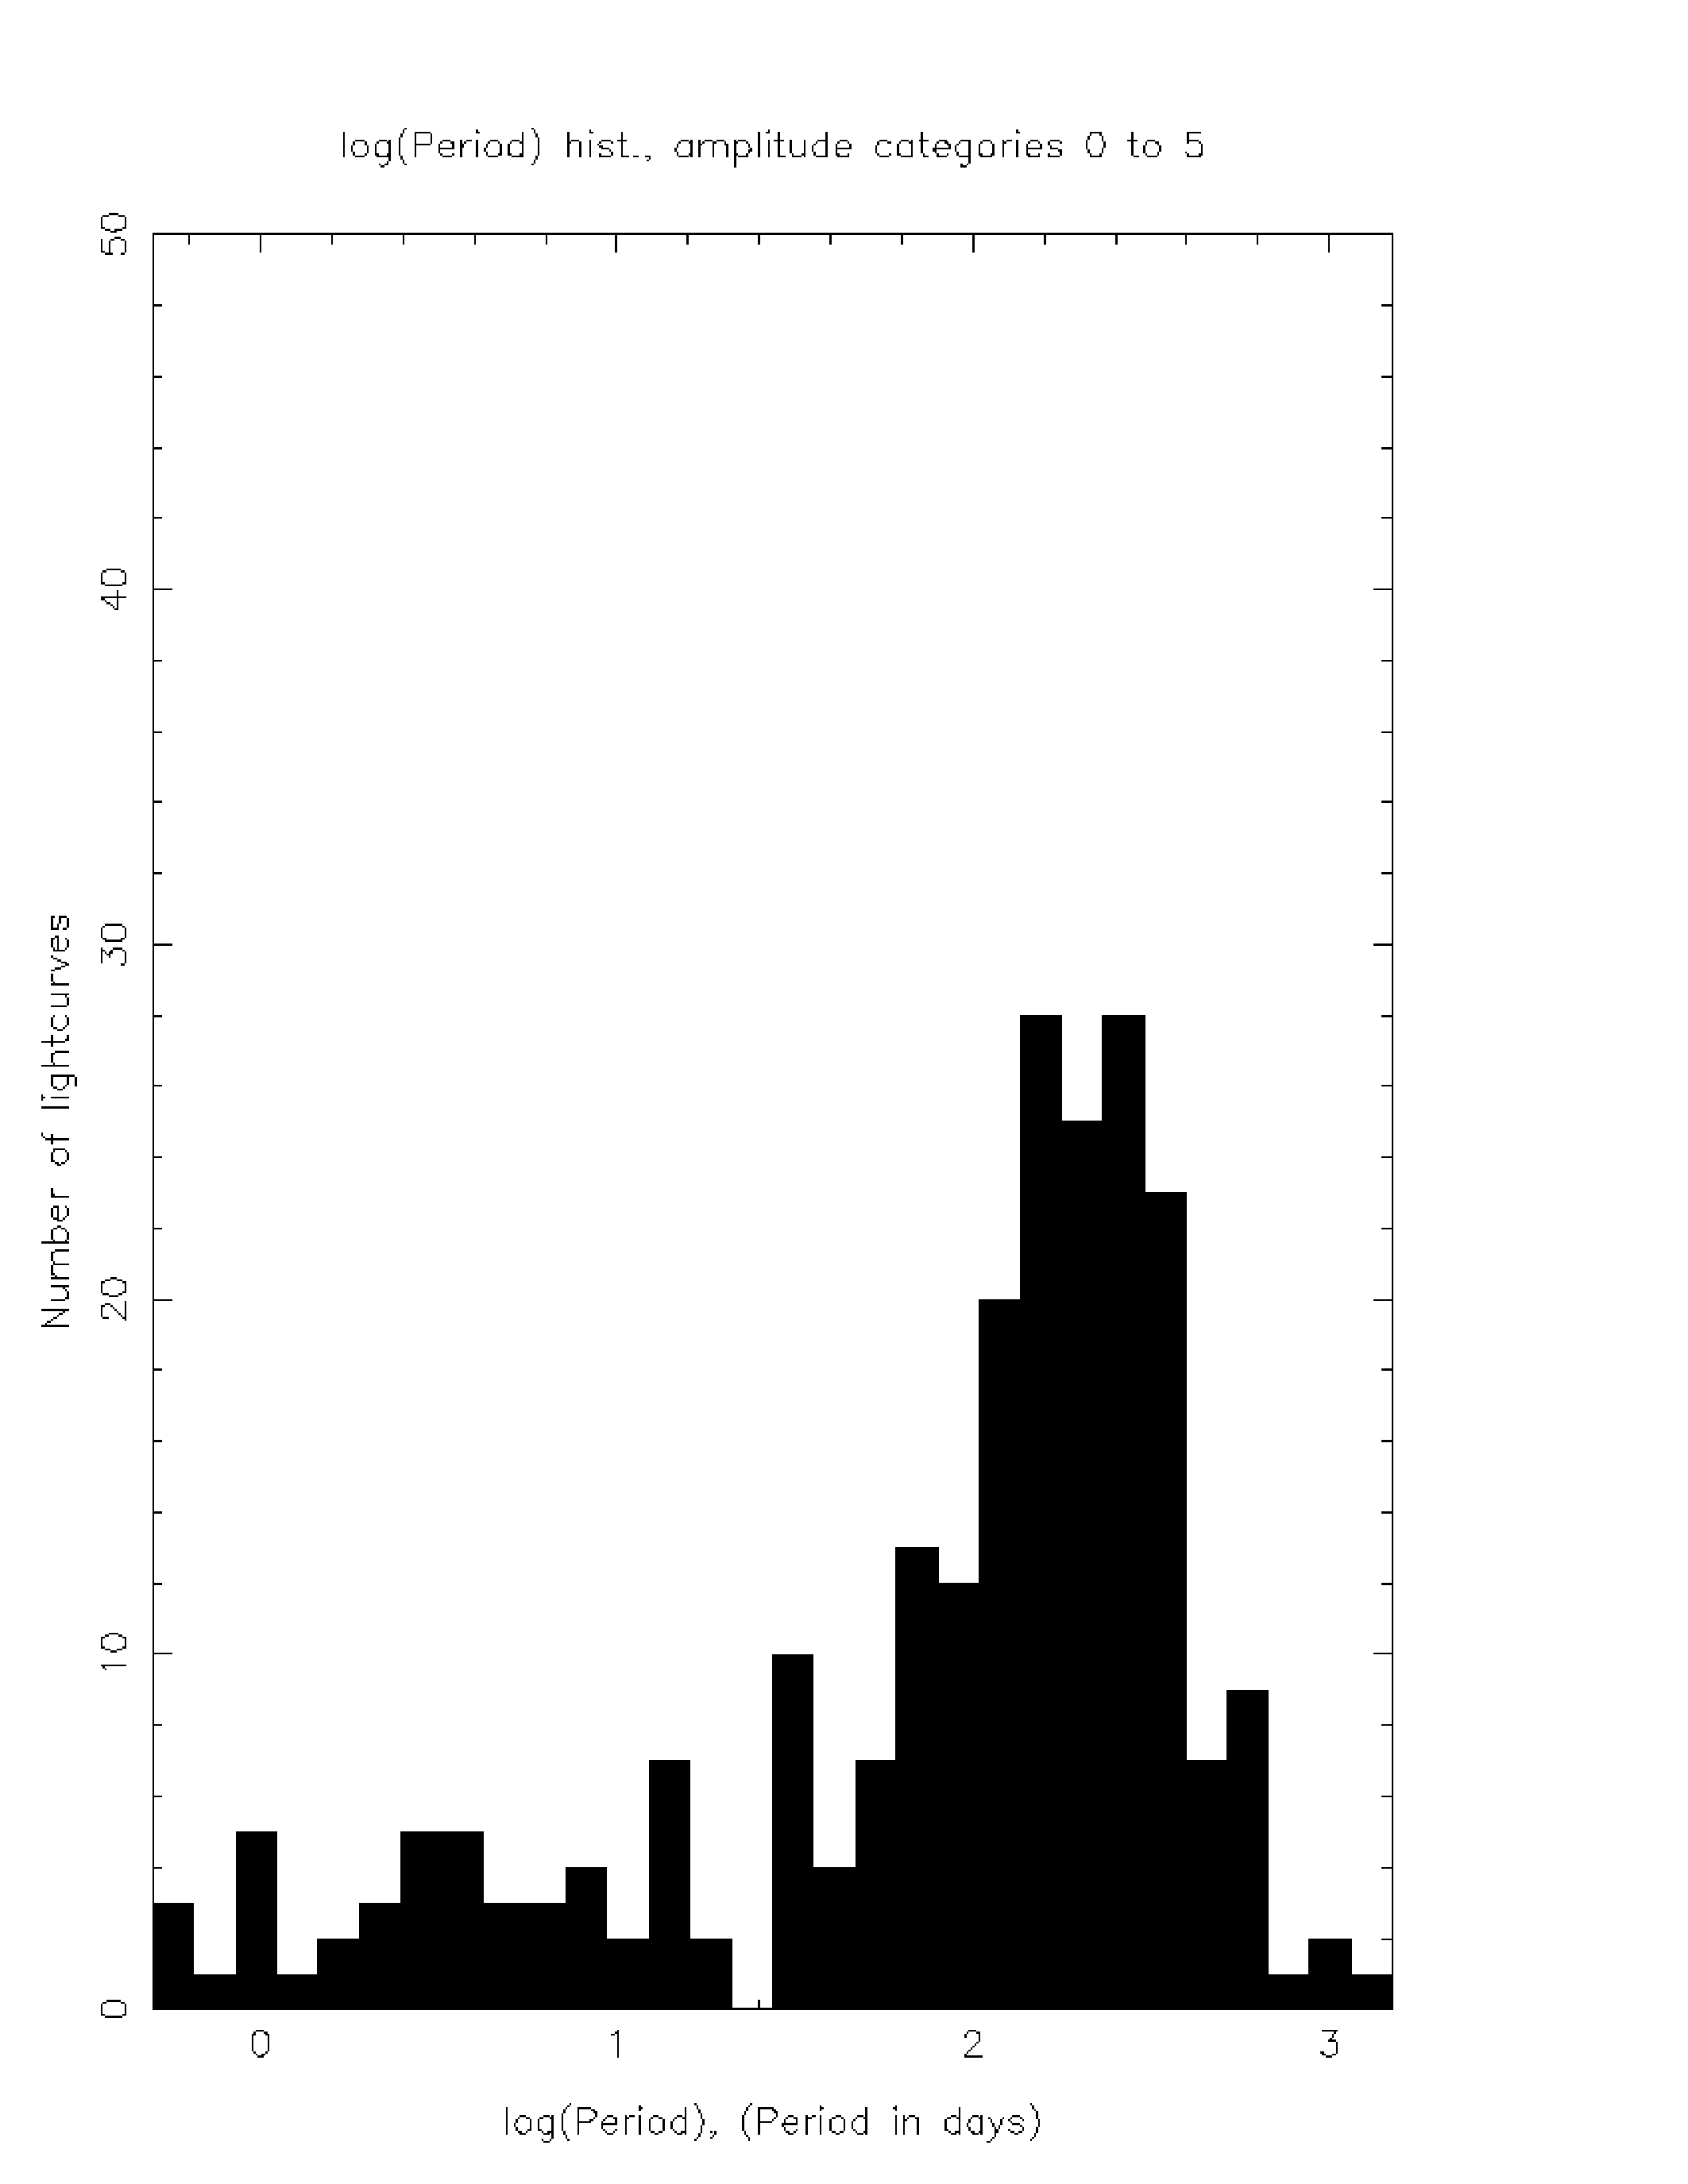} \\
\vspace*{0cm}
   \leavevmode
 \includegraphics{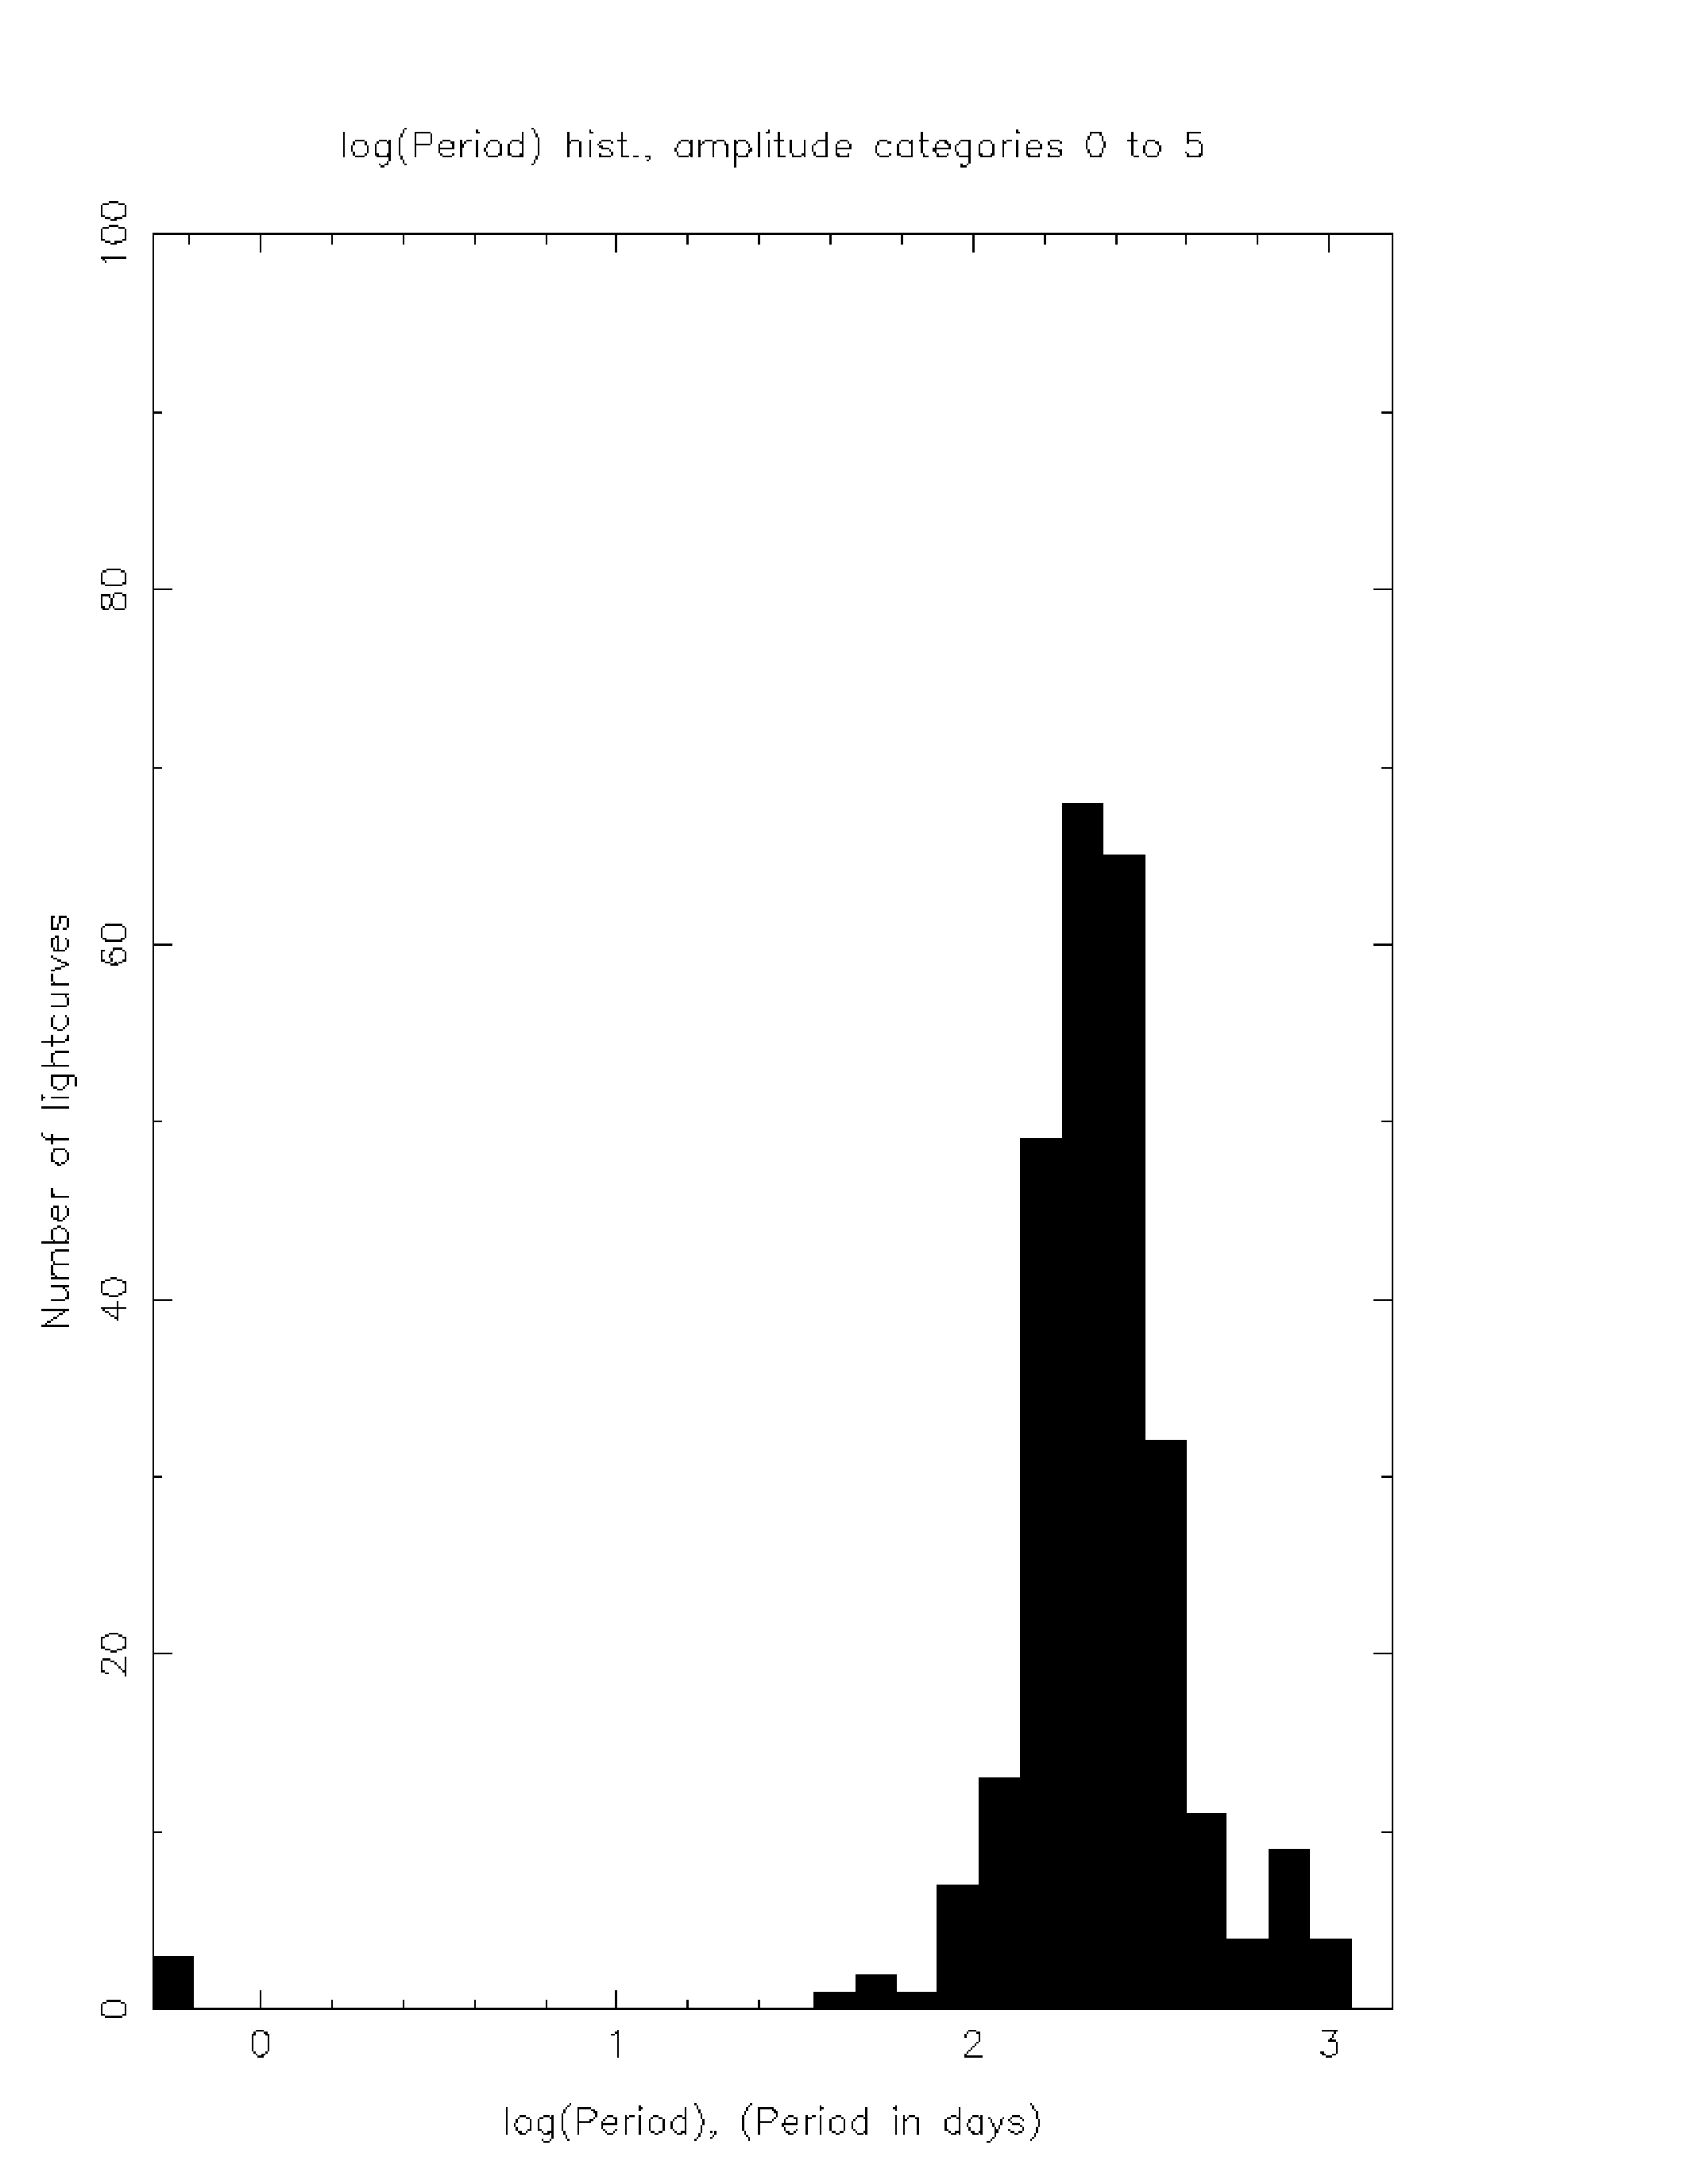} \\
  \end{tabular}
\hspace*{4cm}
  \begin{tabular}{ccc}
% 5 - whatever
\vspace*{5cm}
   \leavevmode
 \includegraphics{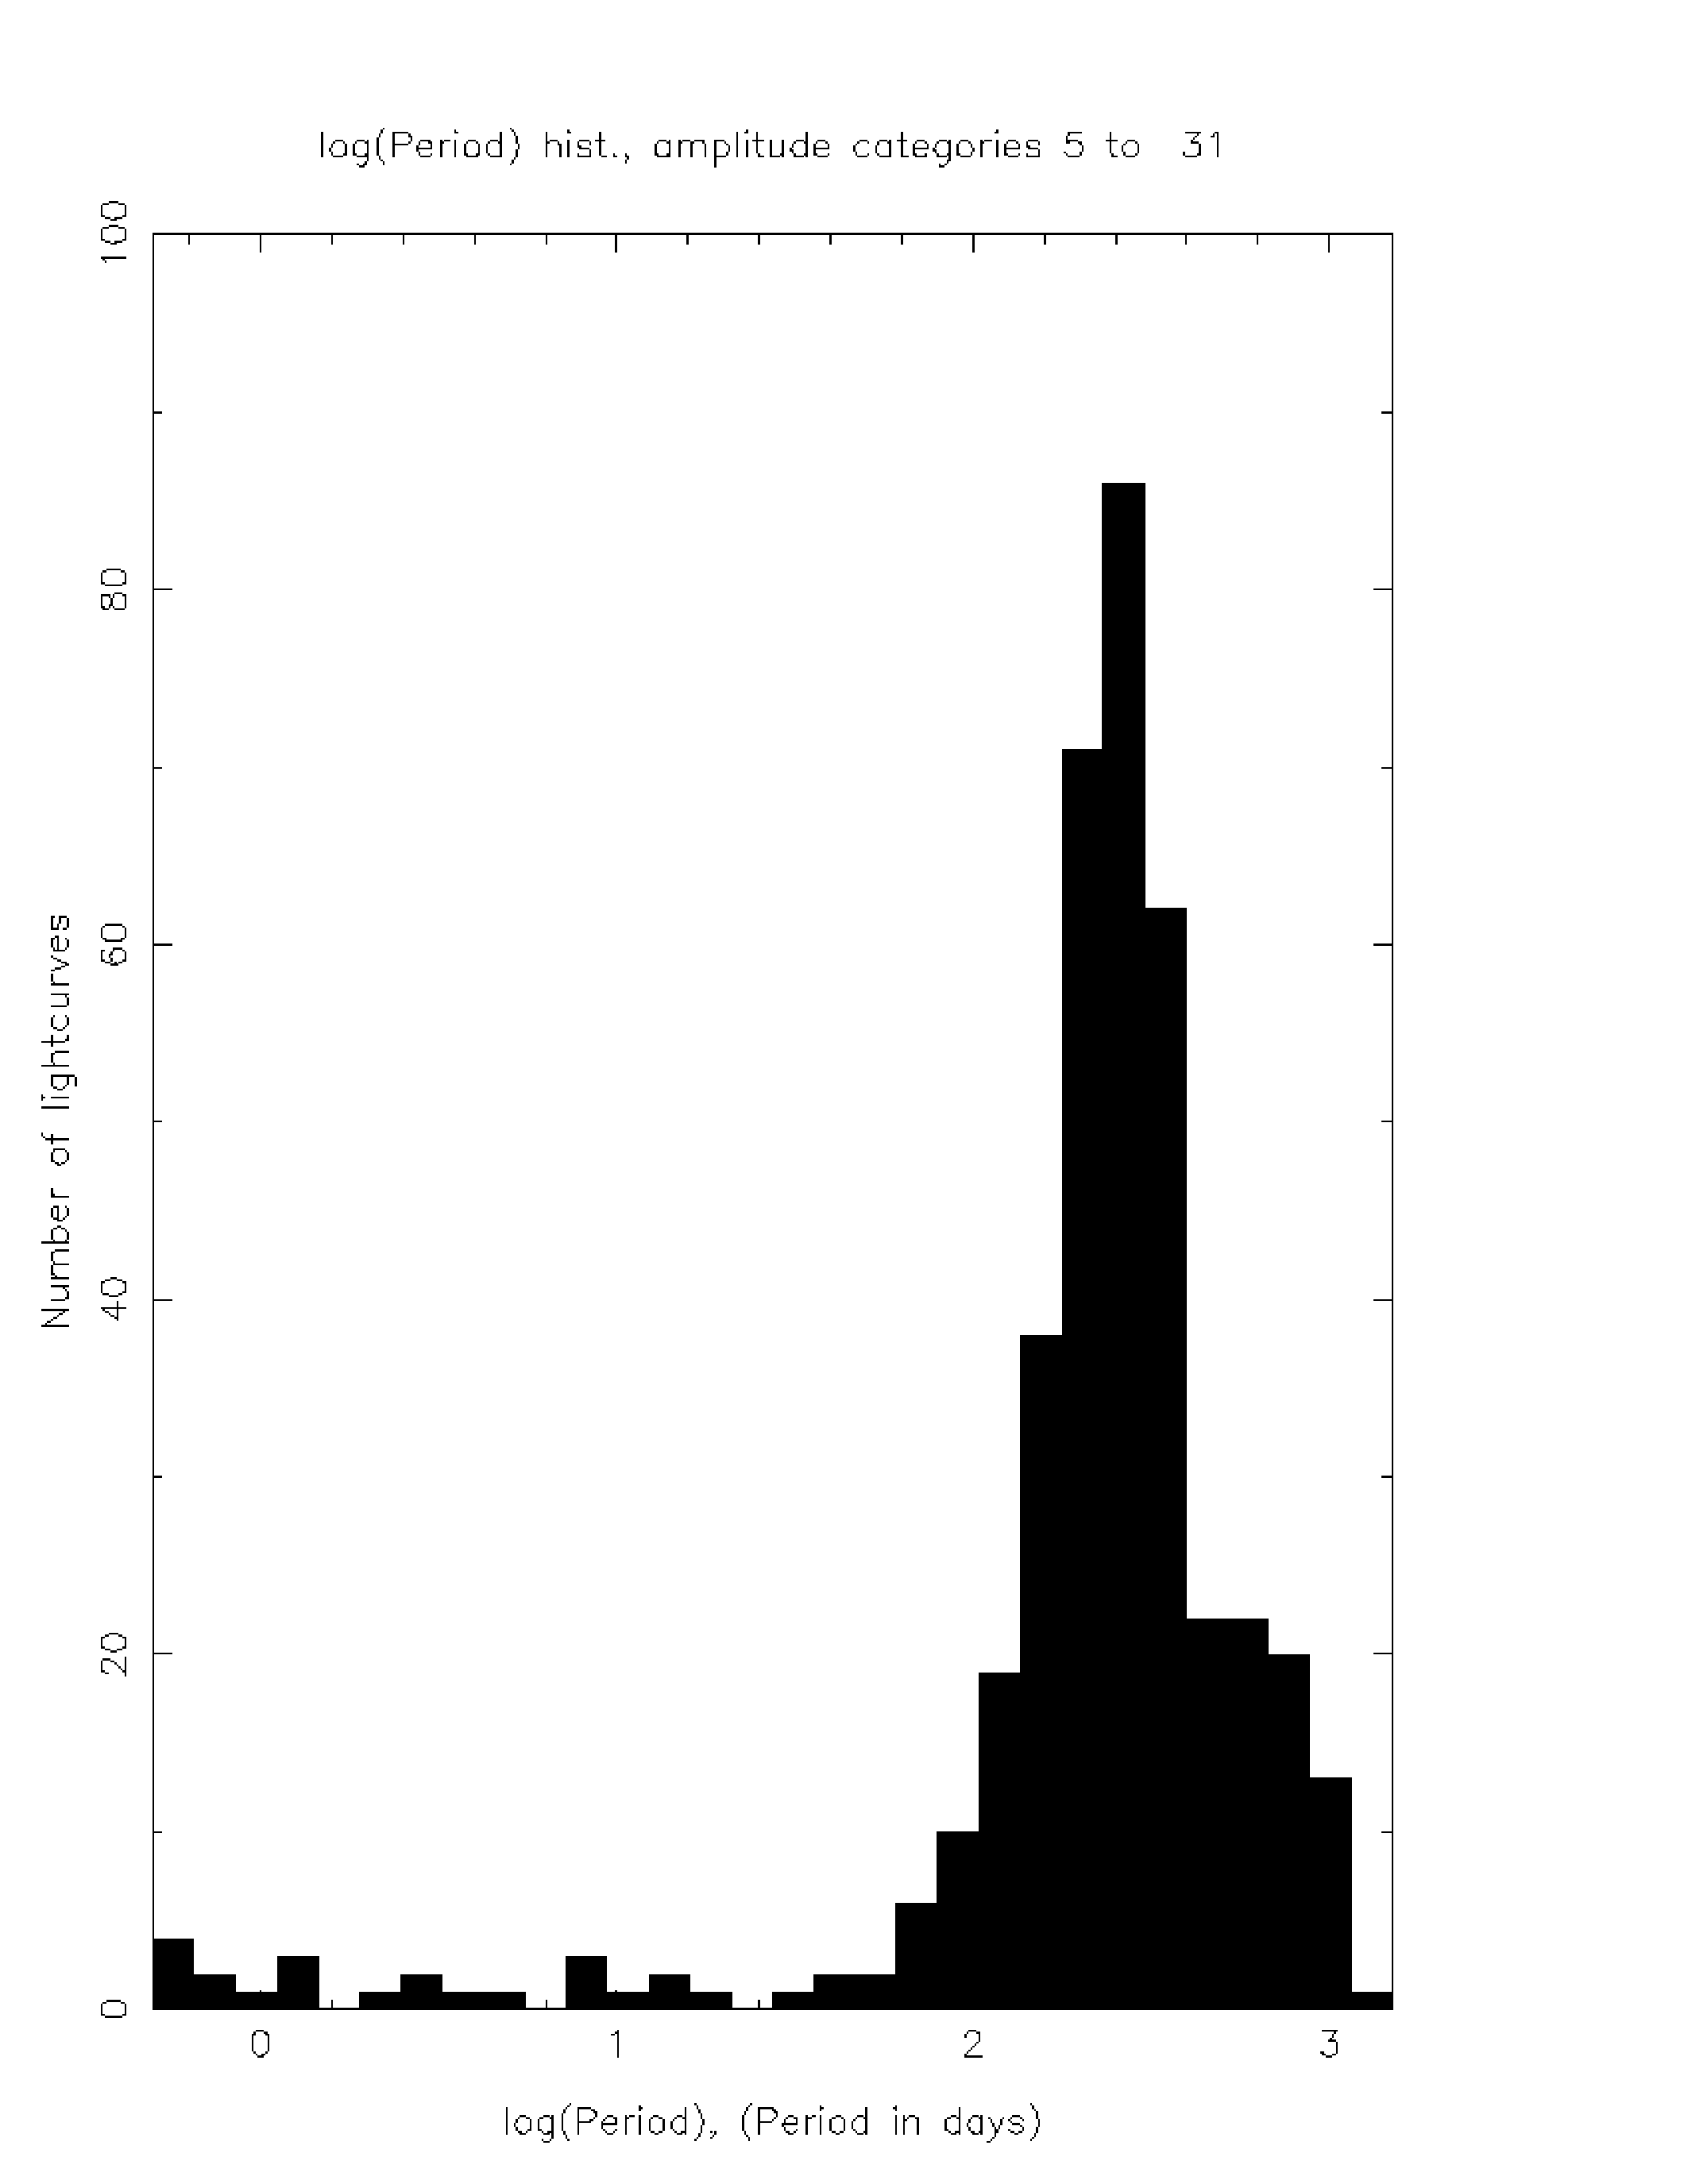} \\
 \vspace*{5cm}
   \leavevmode
\includegraphics{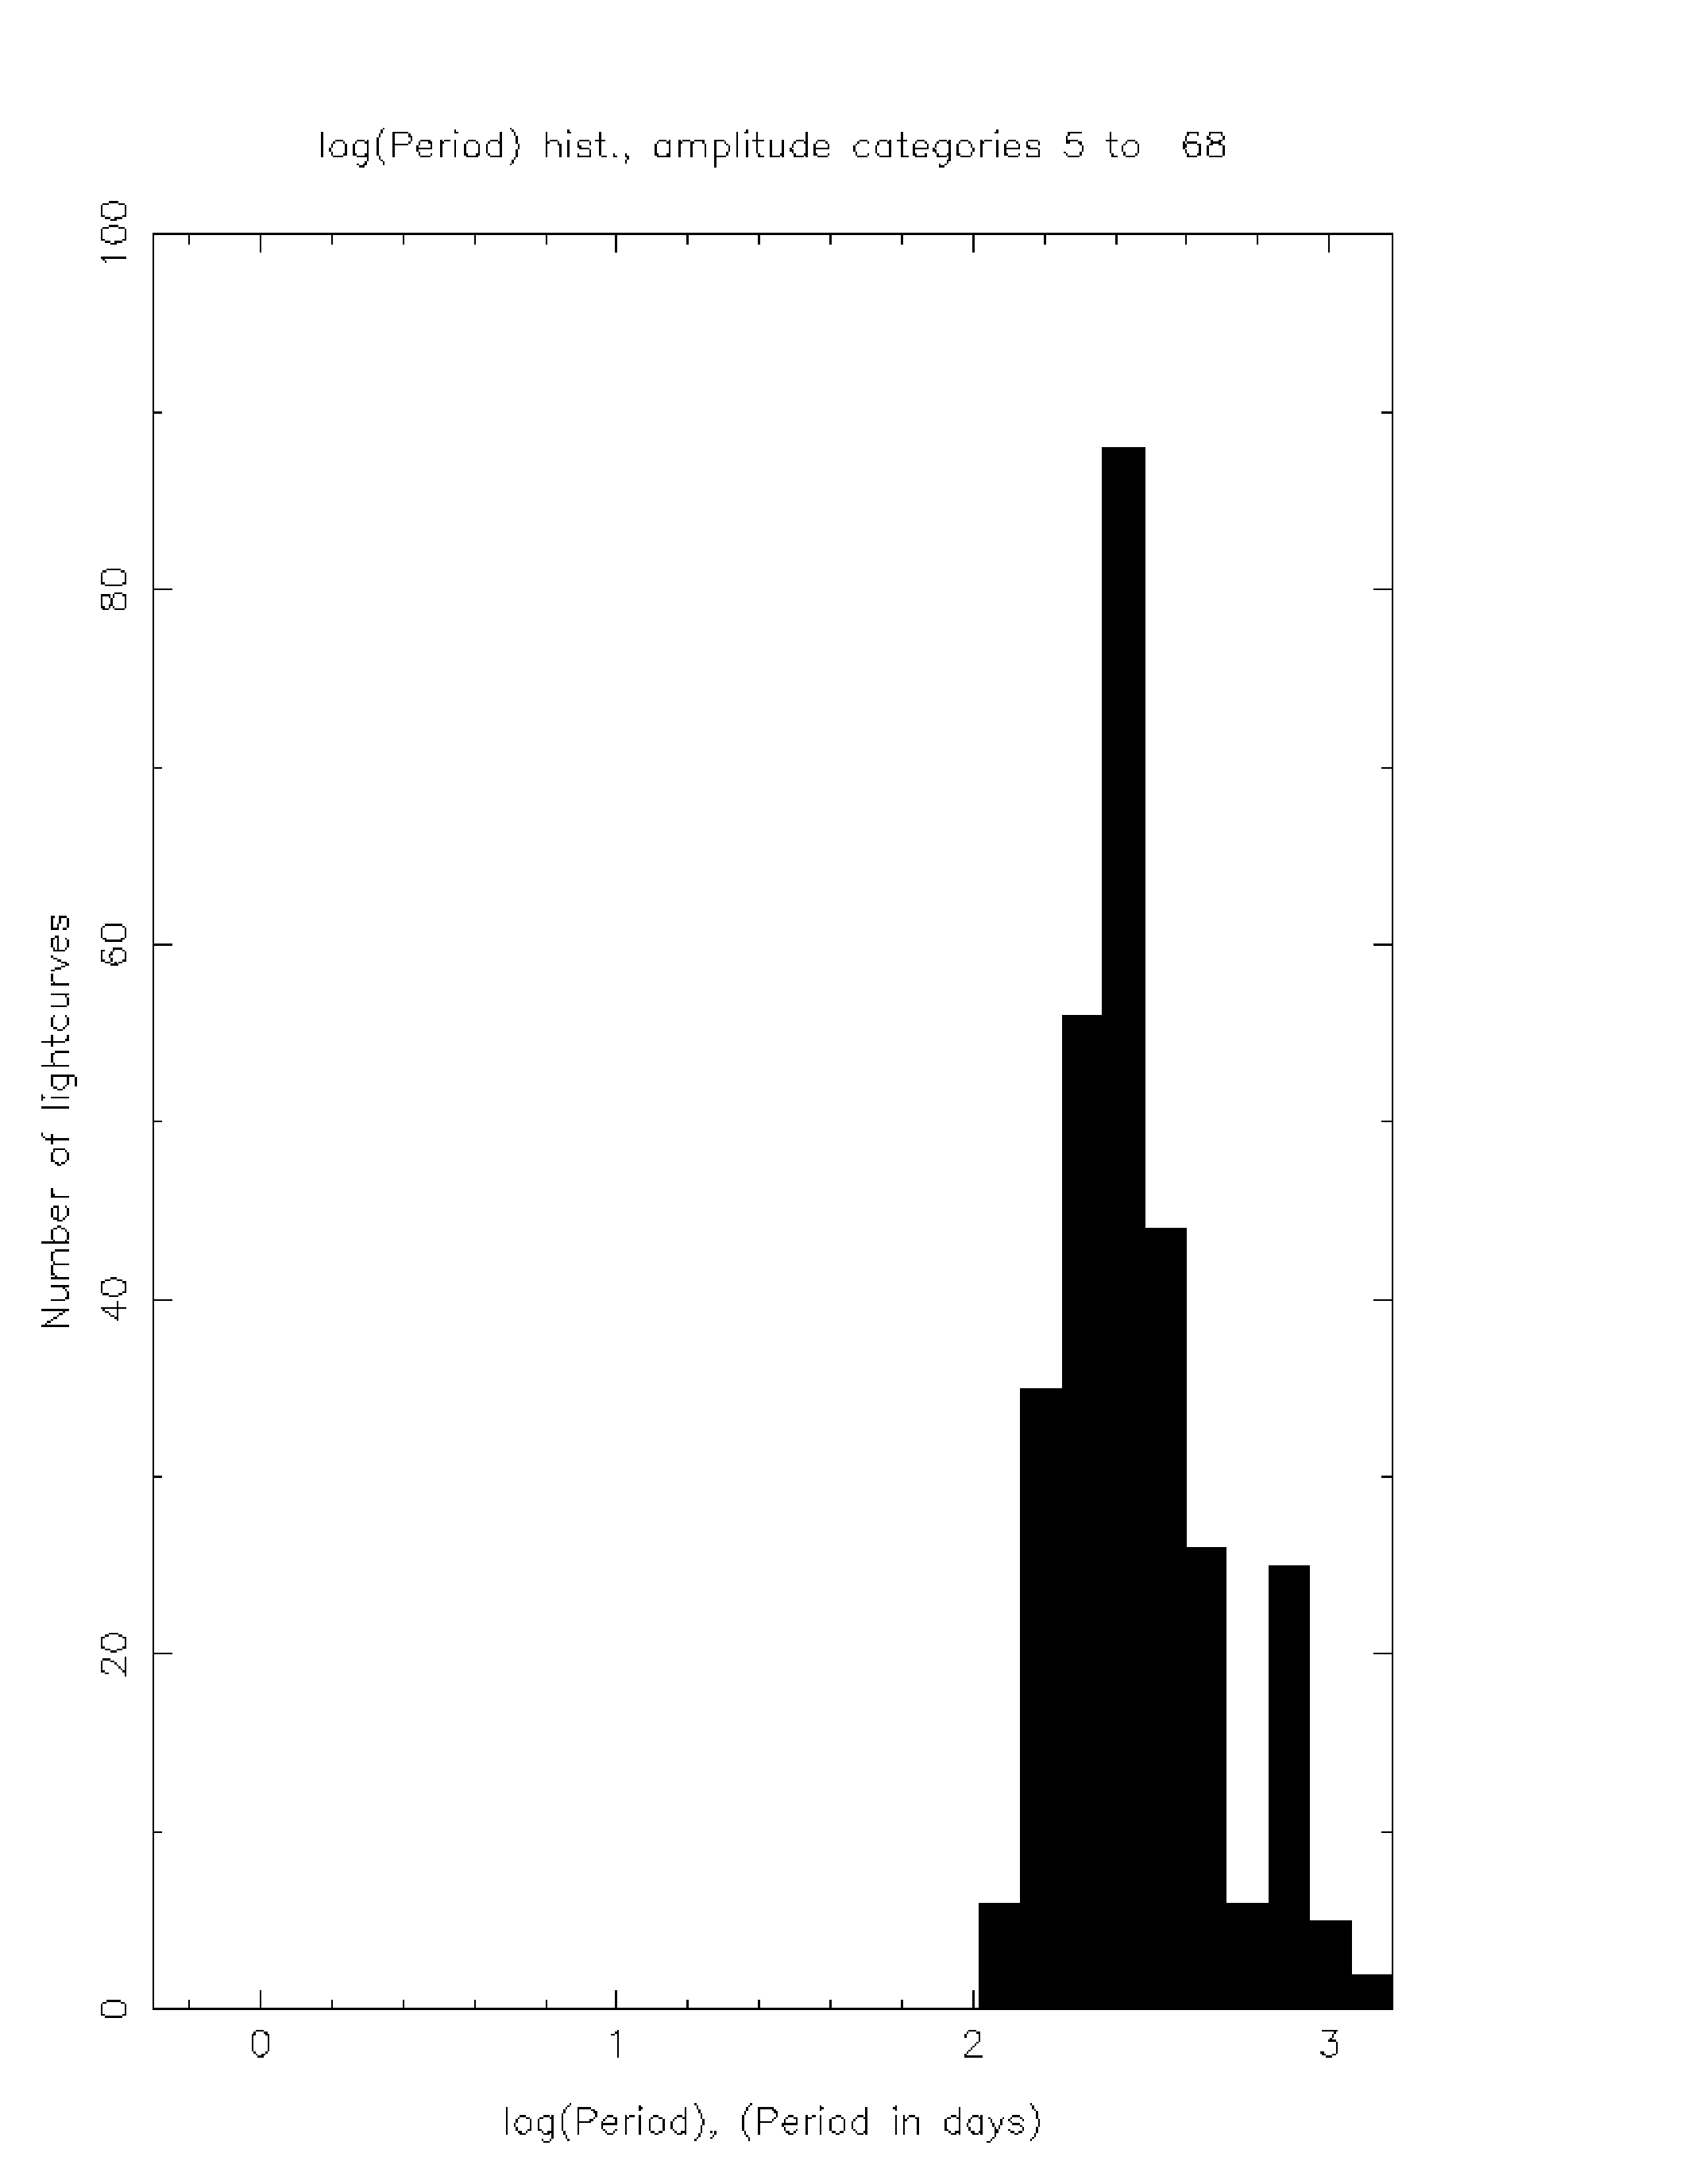} \\
\vspace*{5cm}
   \leavevmode
 \includegraphics{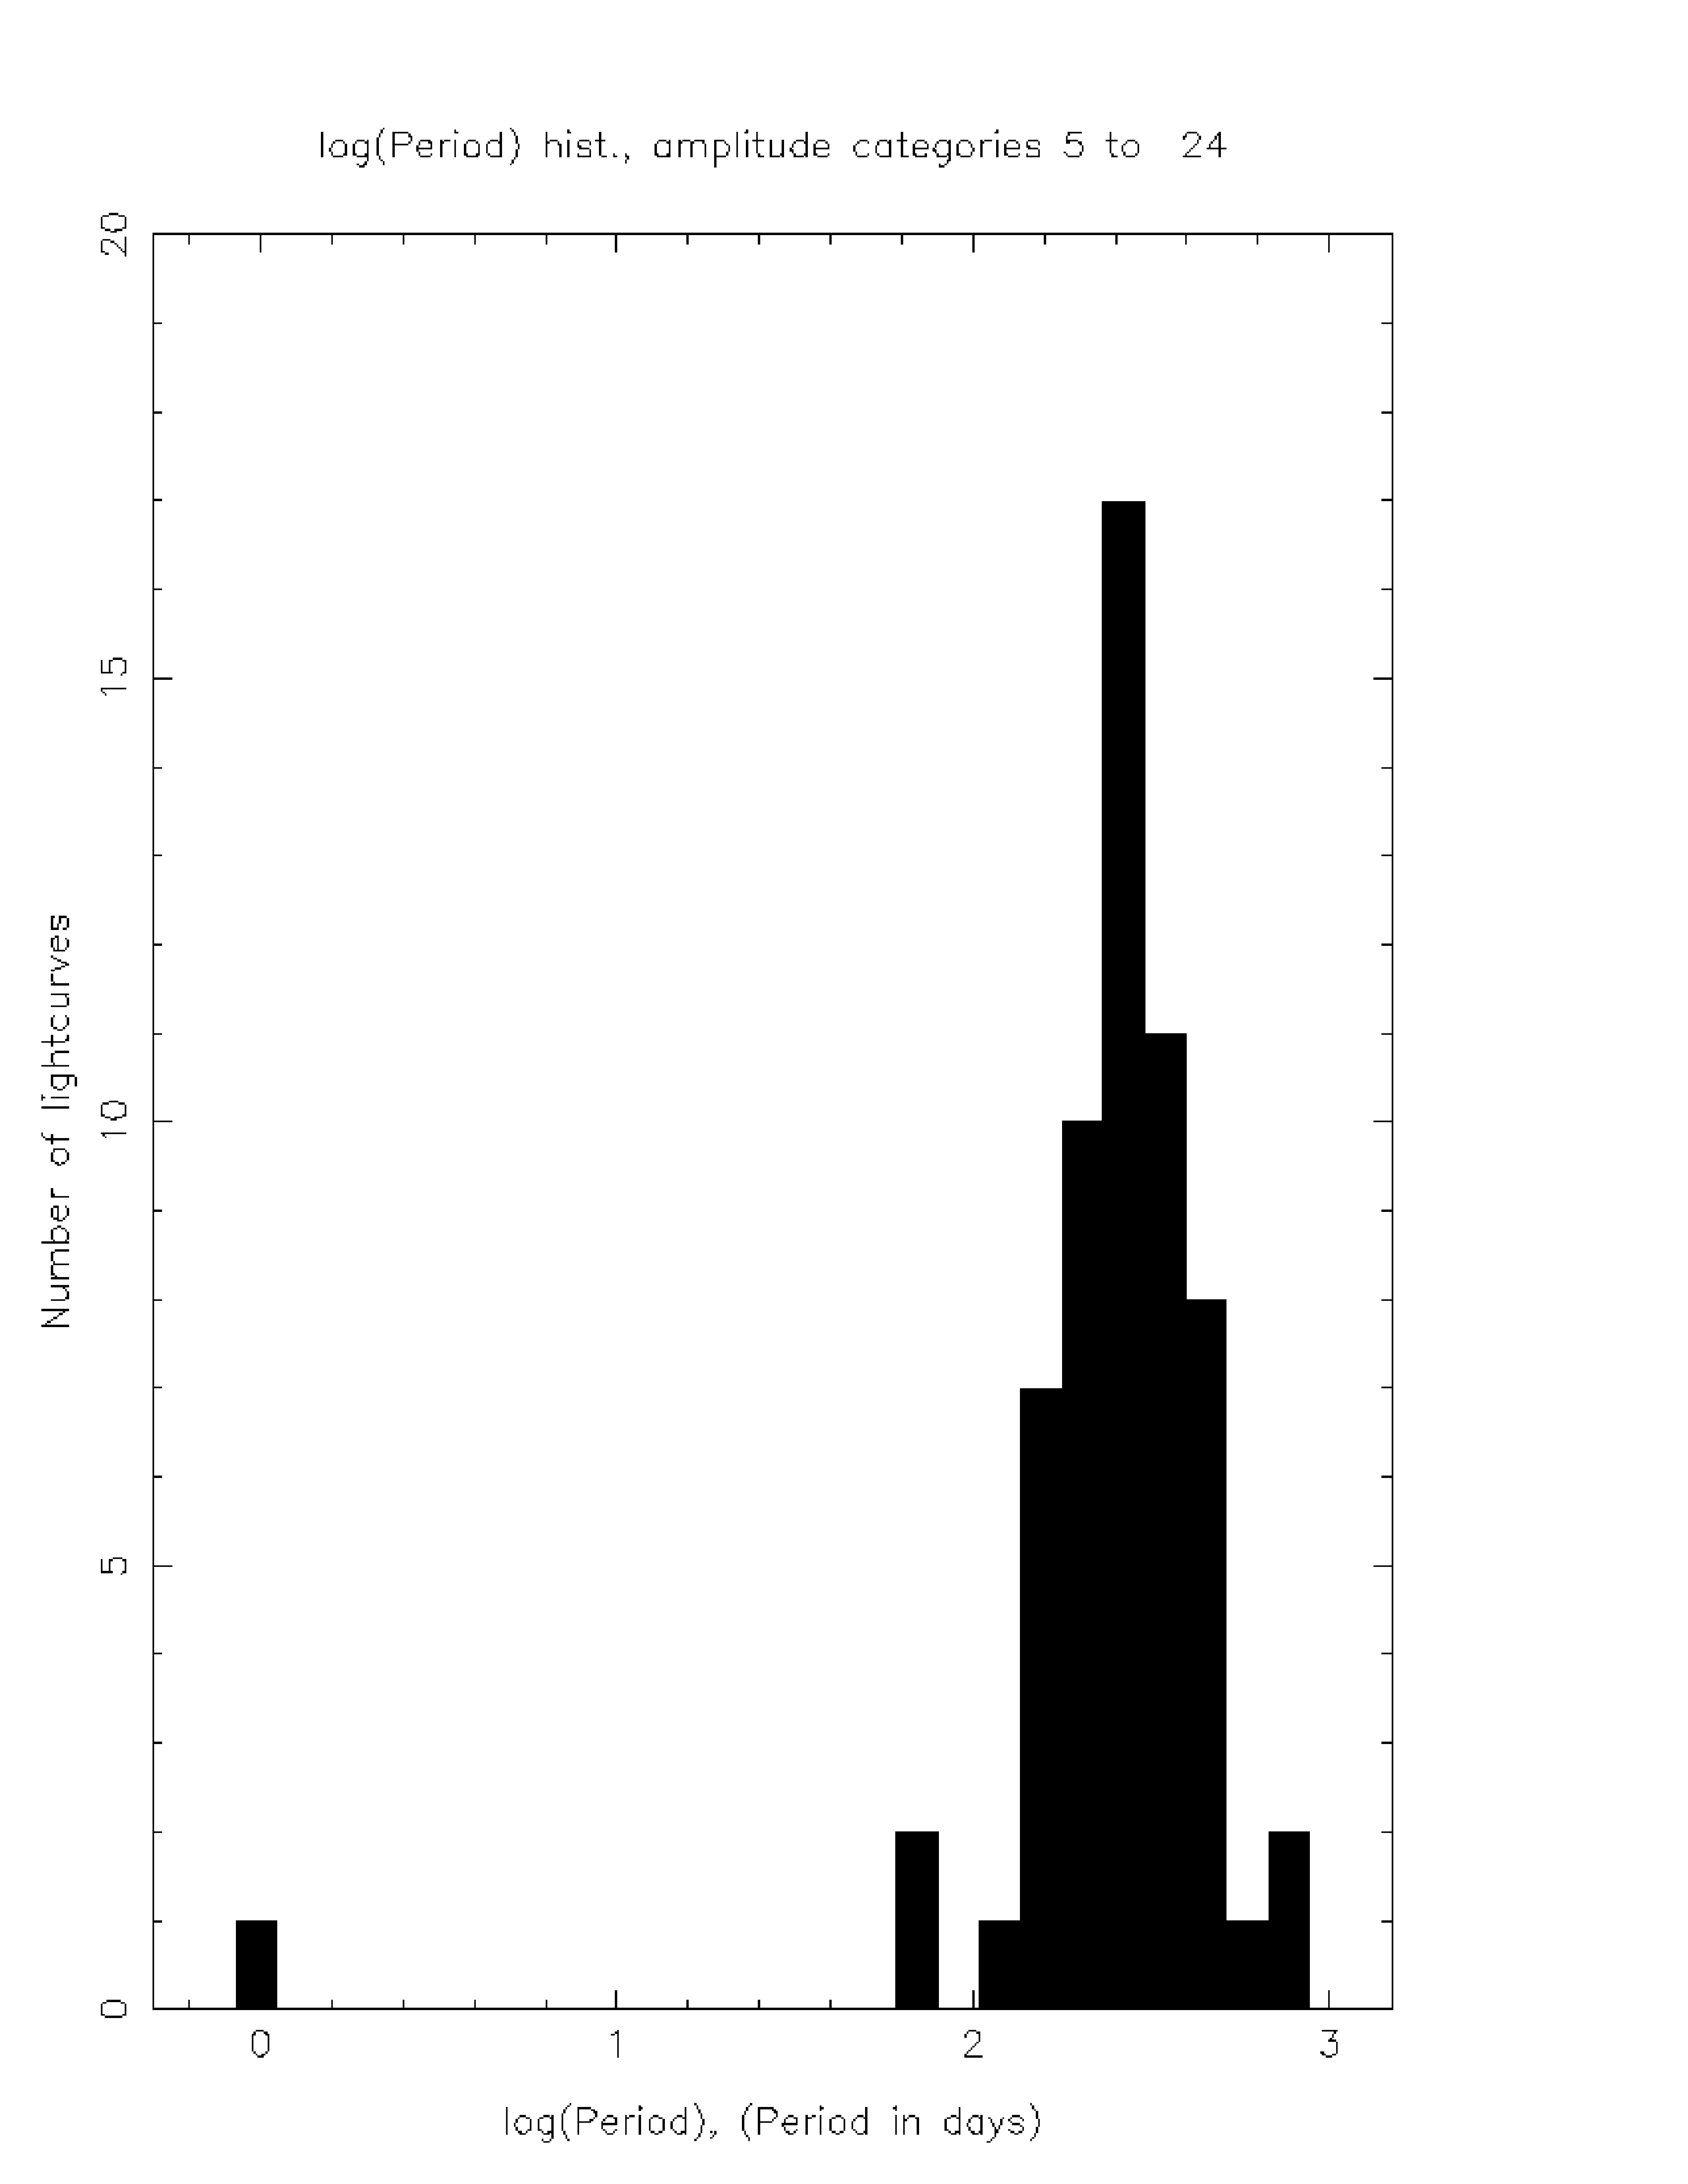} \\
\vspace*{0cm}
   \leavevmode
 \includegraphics{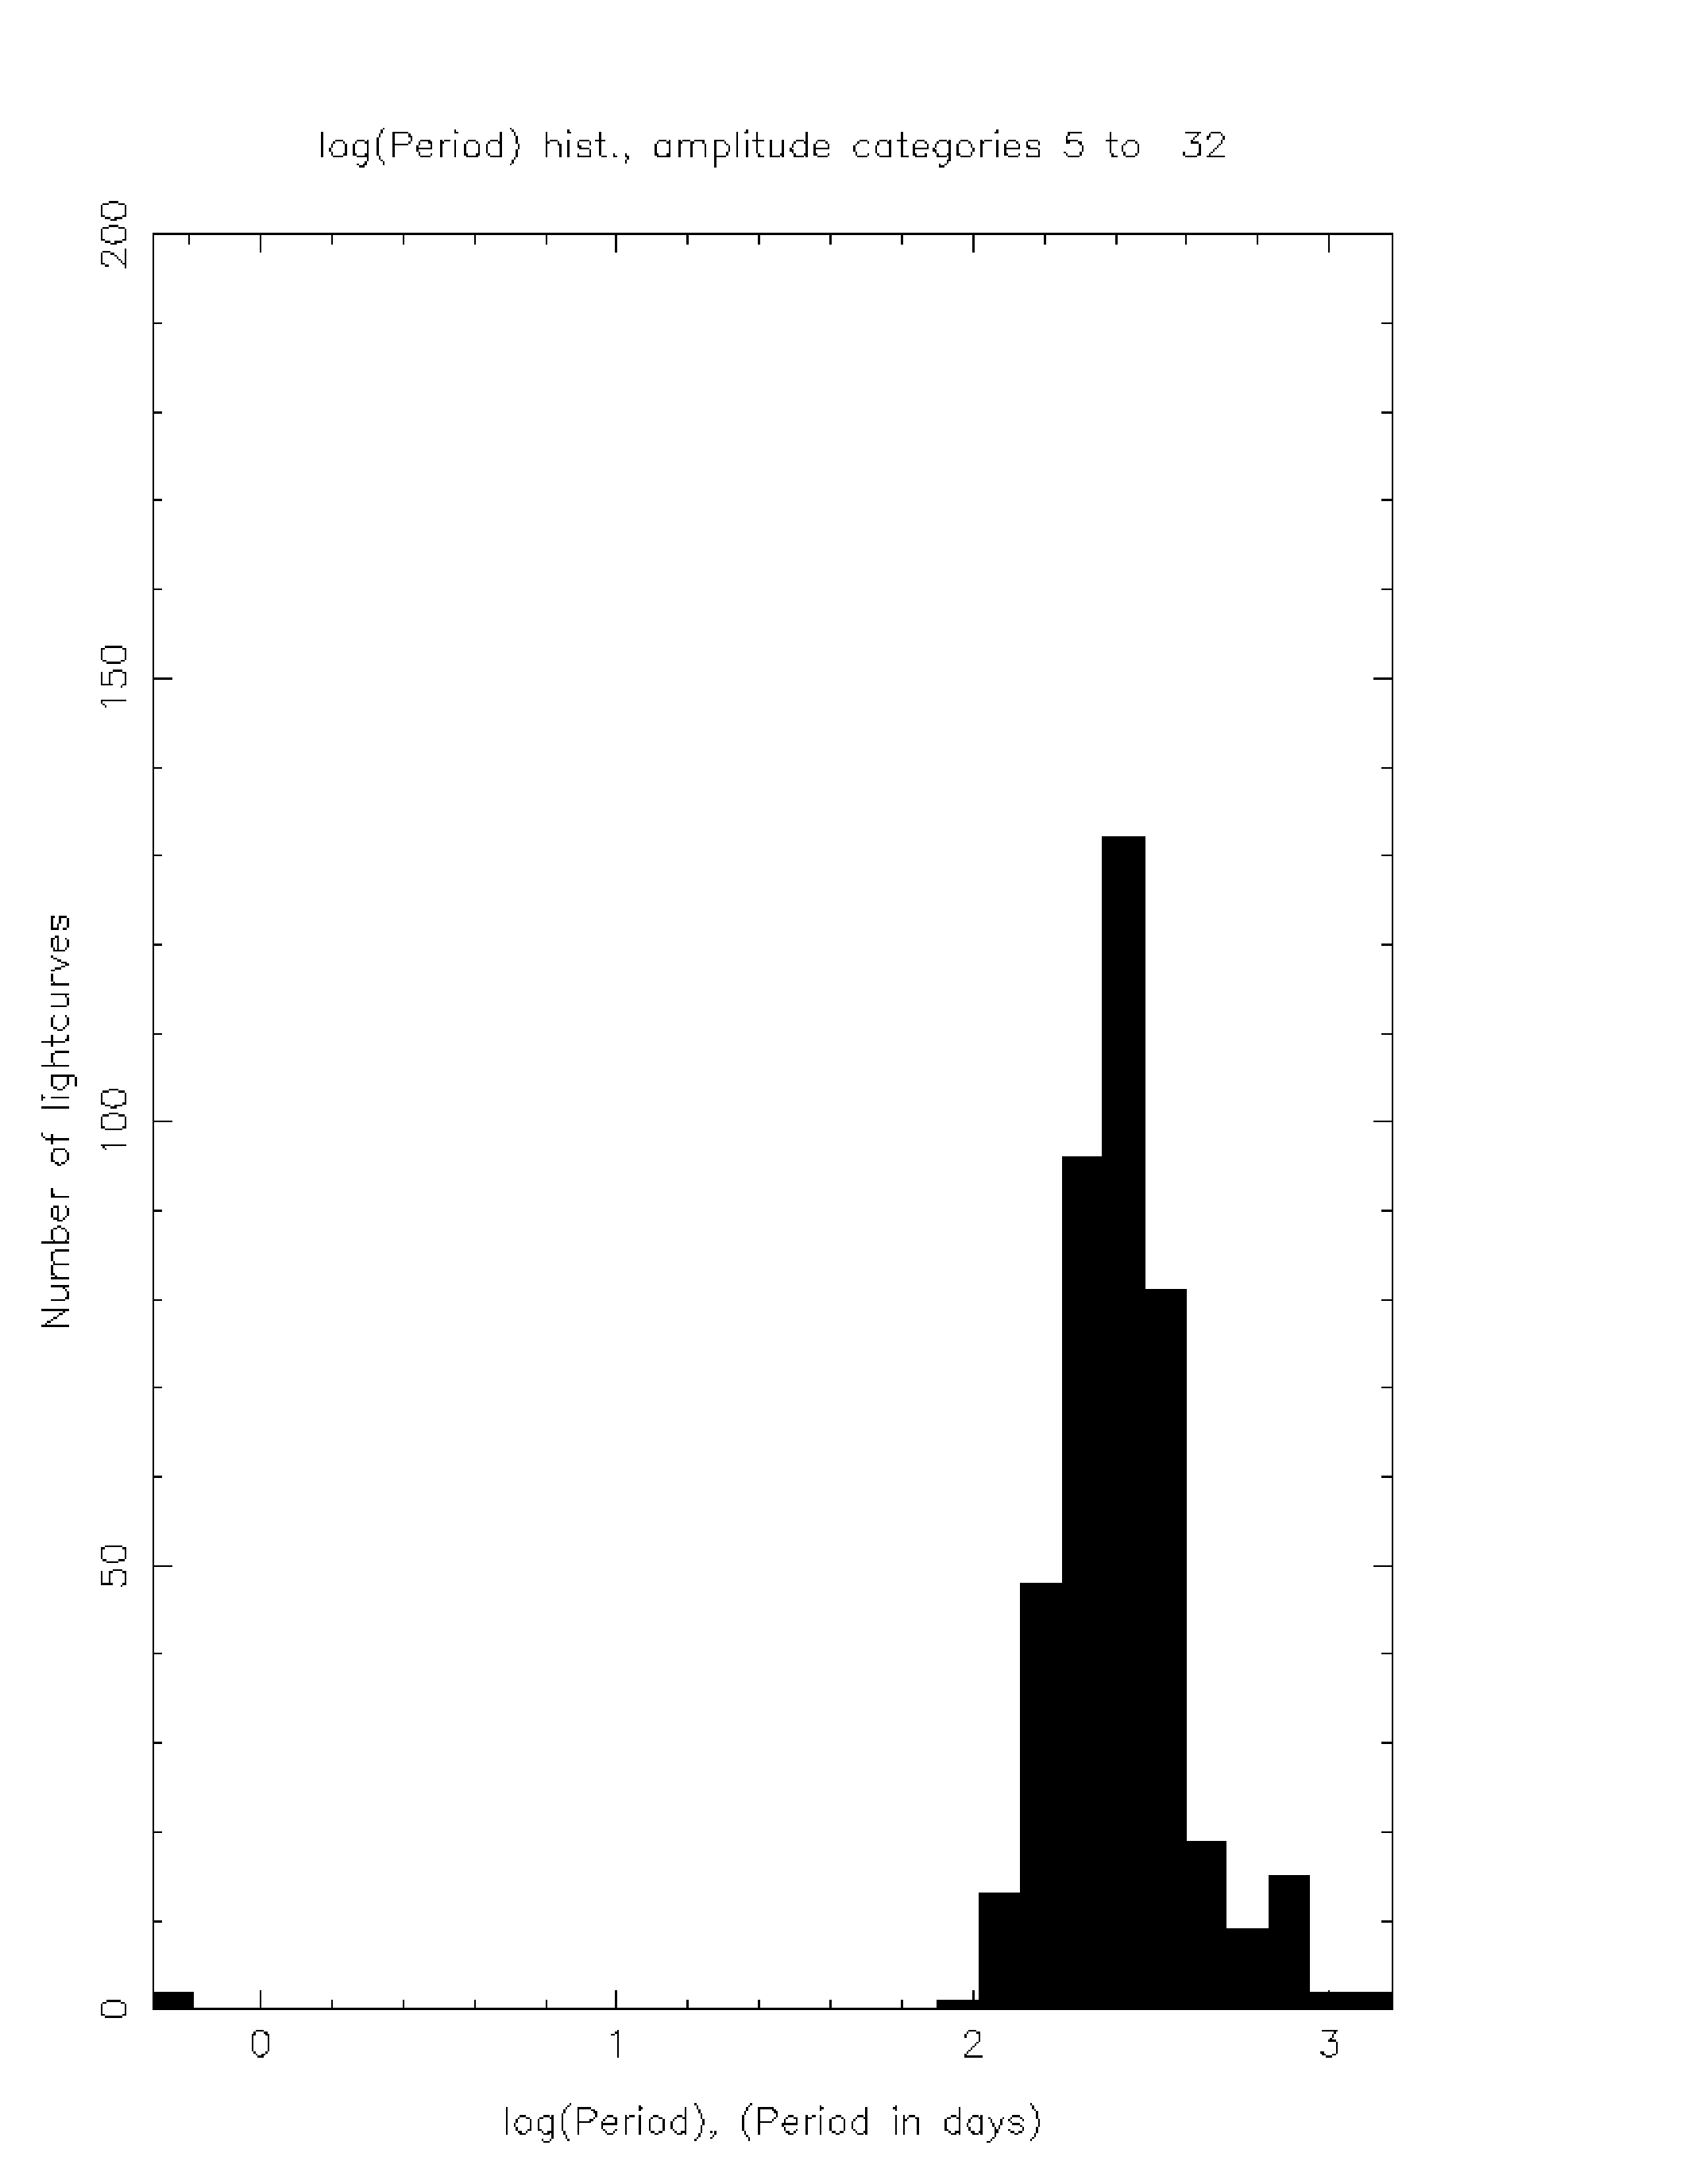} \\
  \end{tabular}
\hspace*{4cm}
  \begin{tabular}{ccc}
%% ALL amp categories.
\vspace*{5cm}
   \leavevmode
 \includegraphics{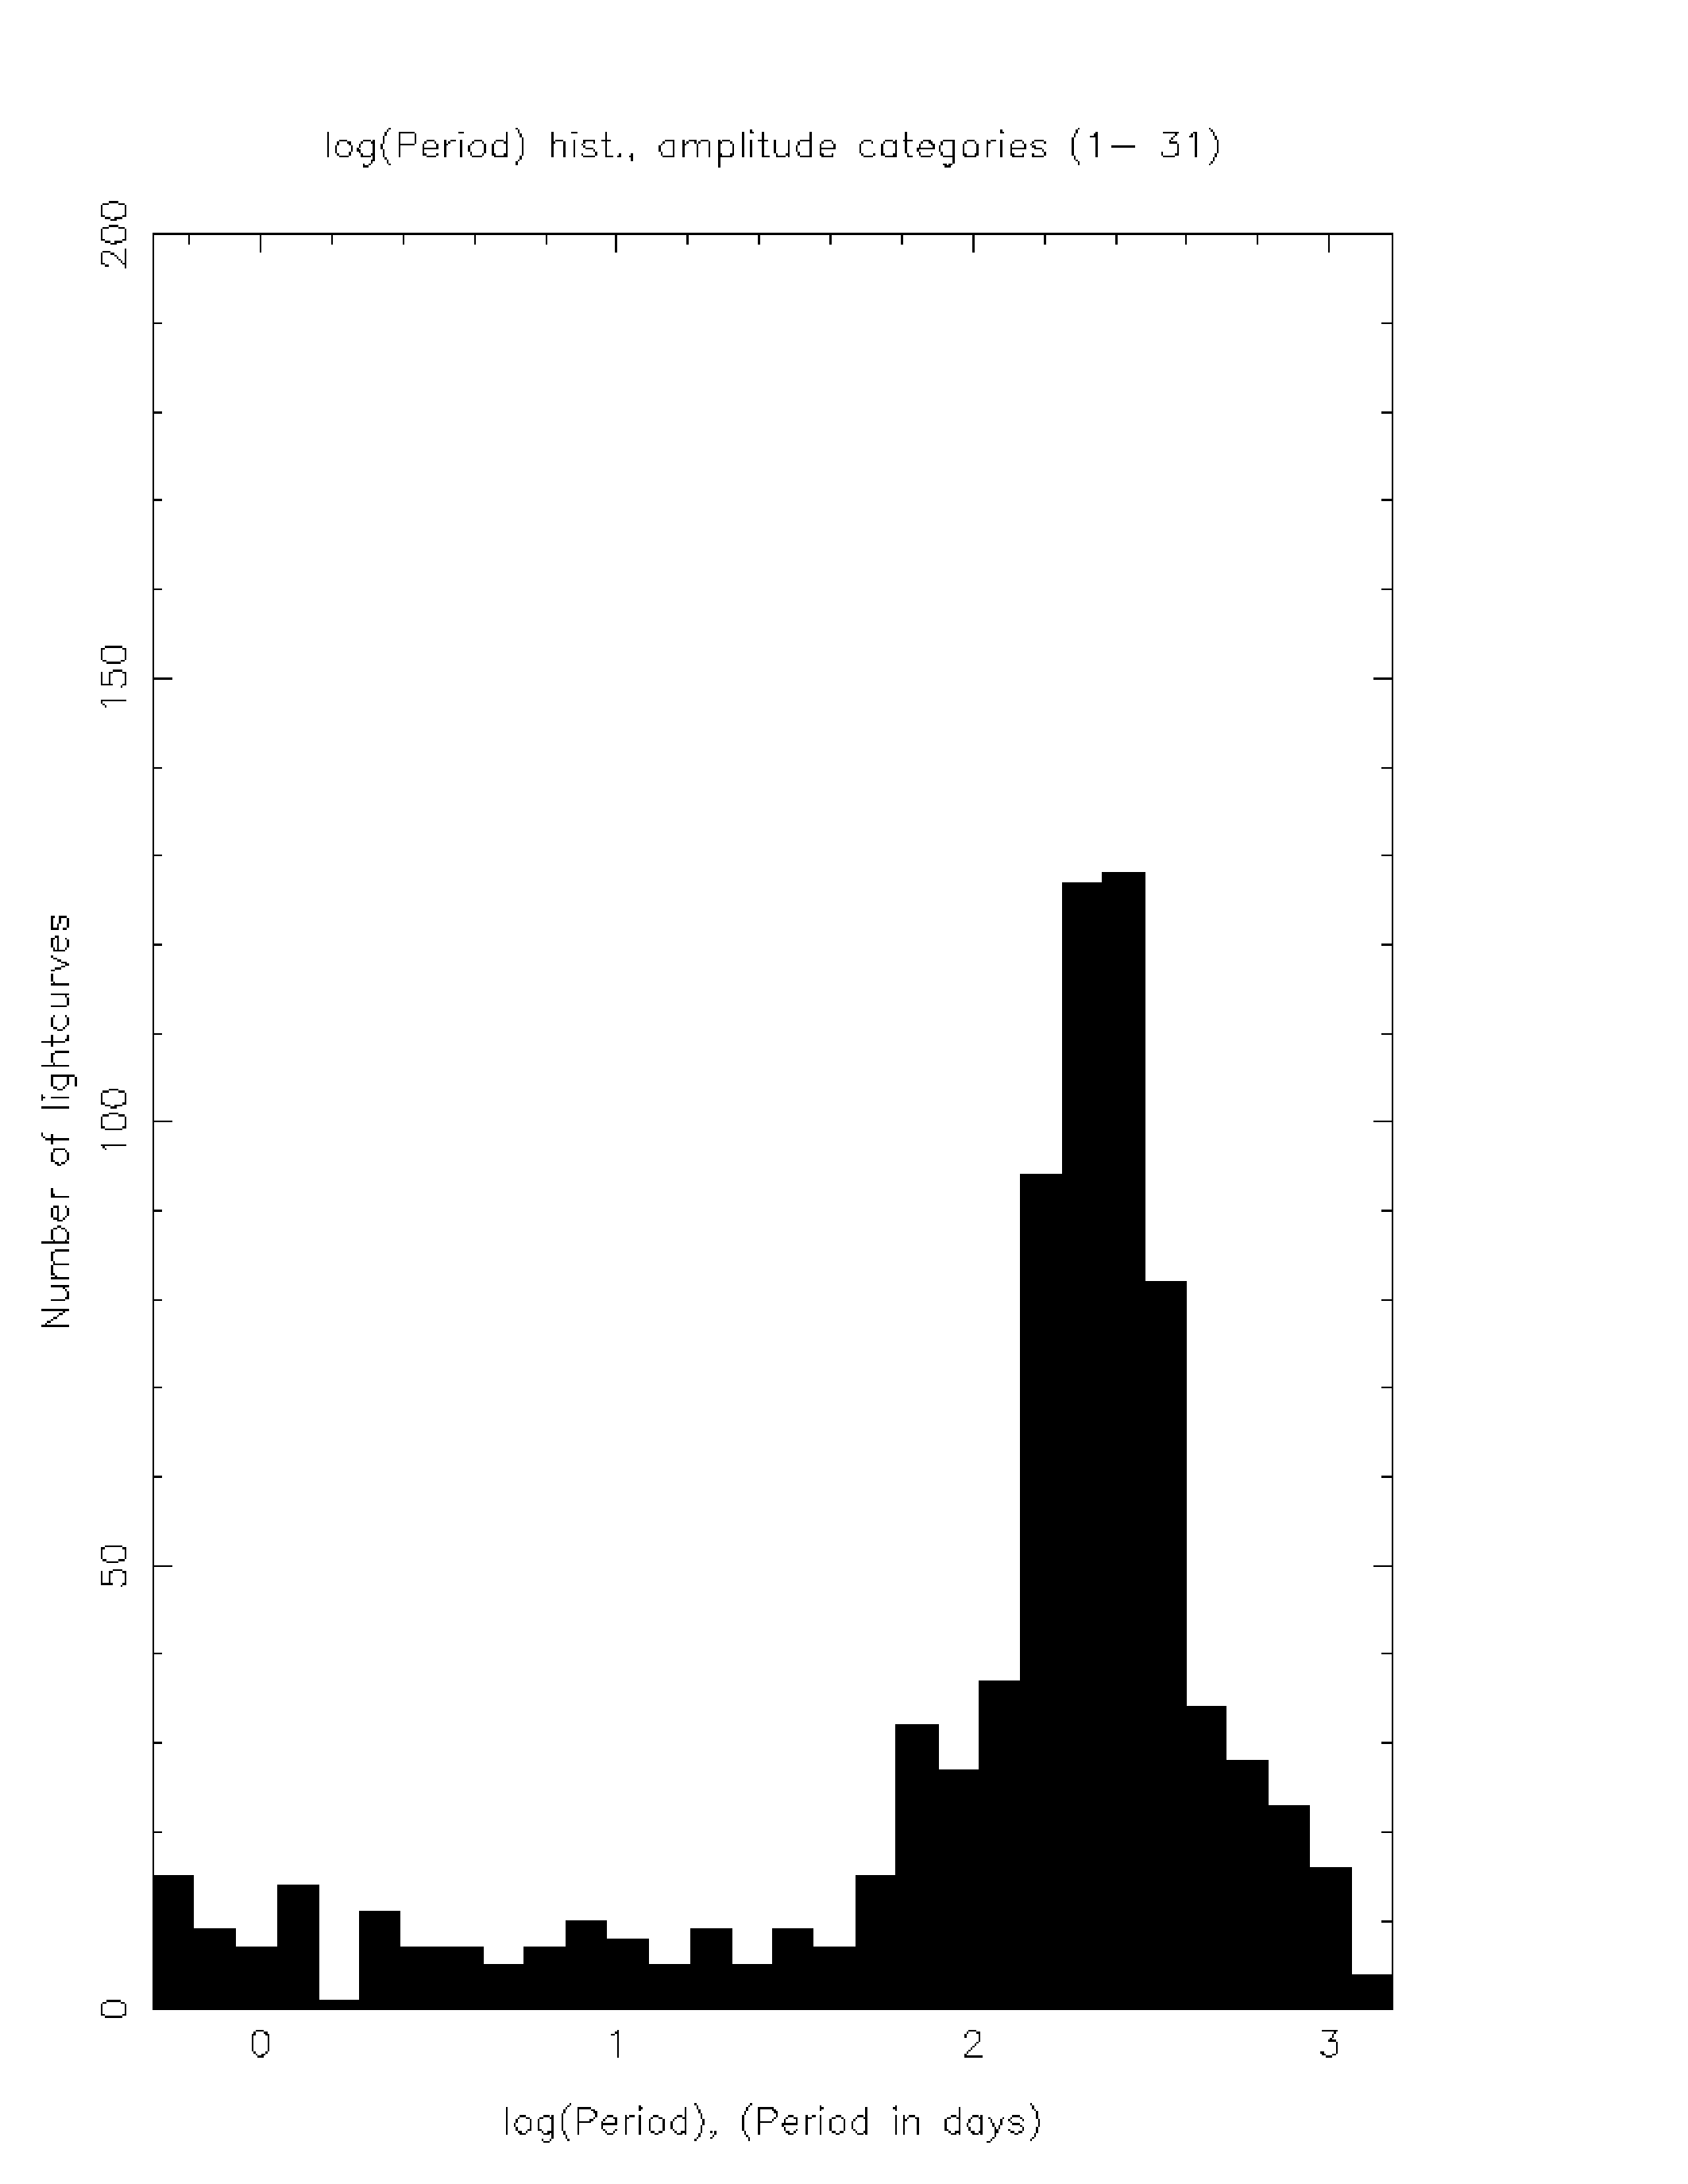} \\
\vspace*{5cm}
   \leavevmode
 \includegraphics{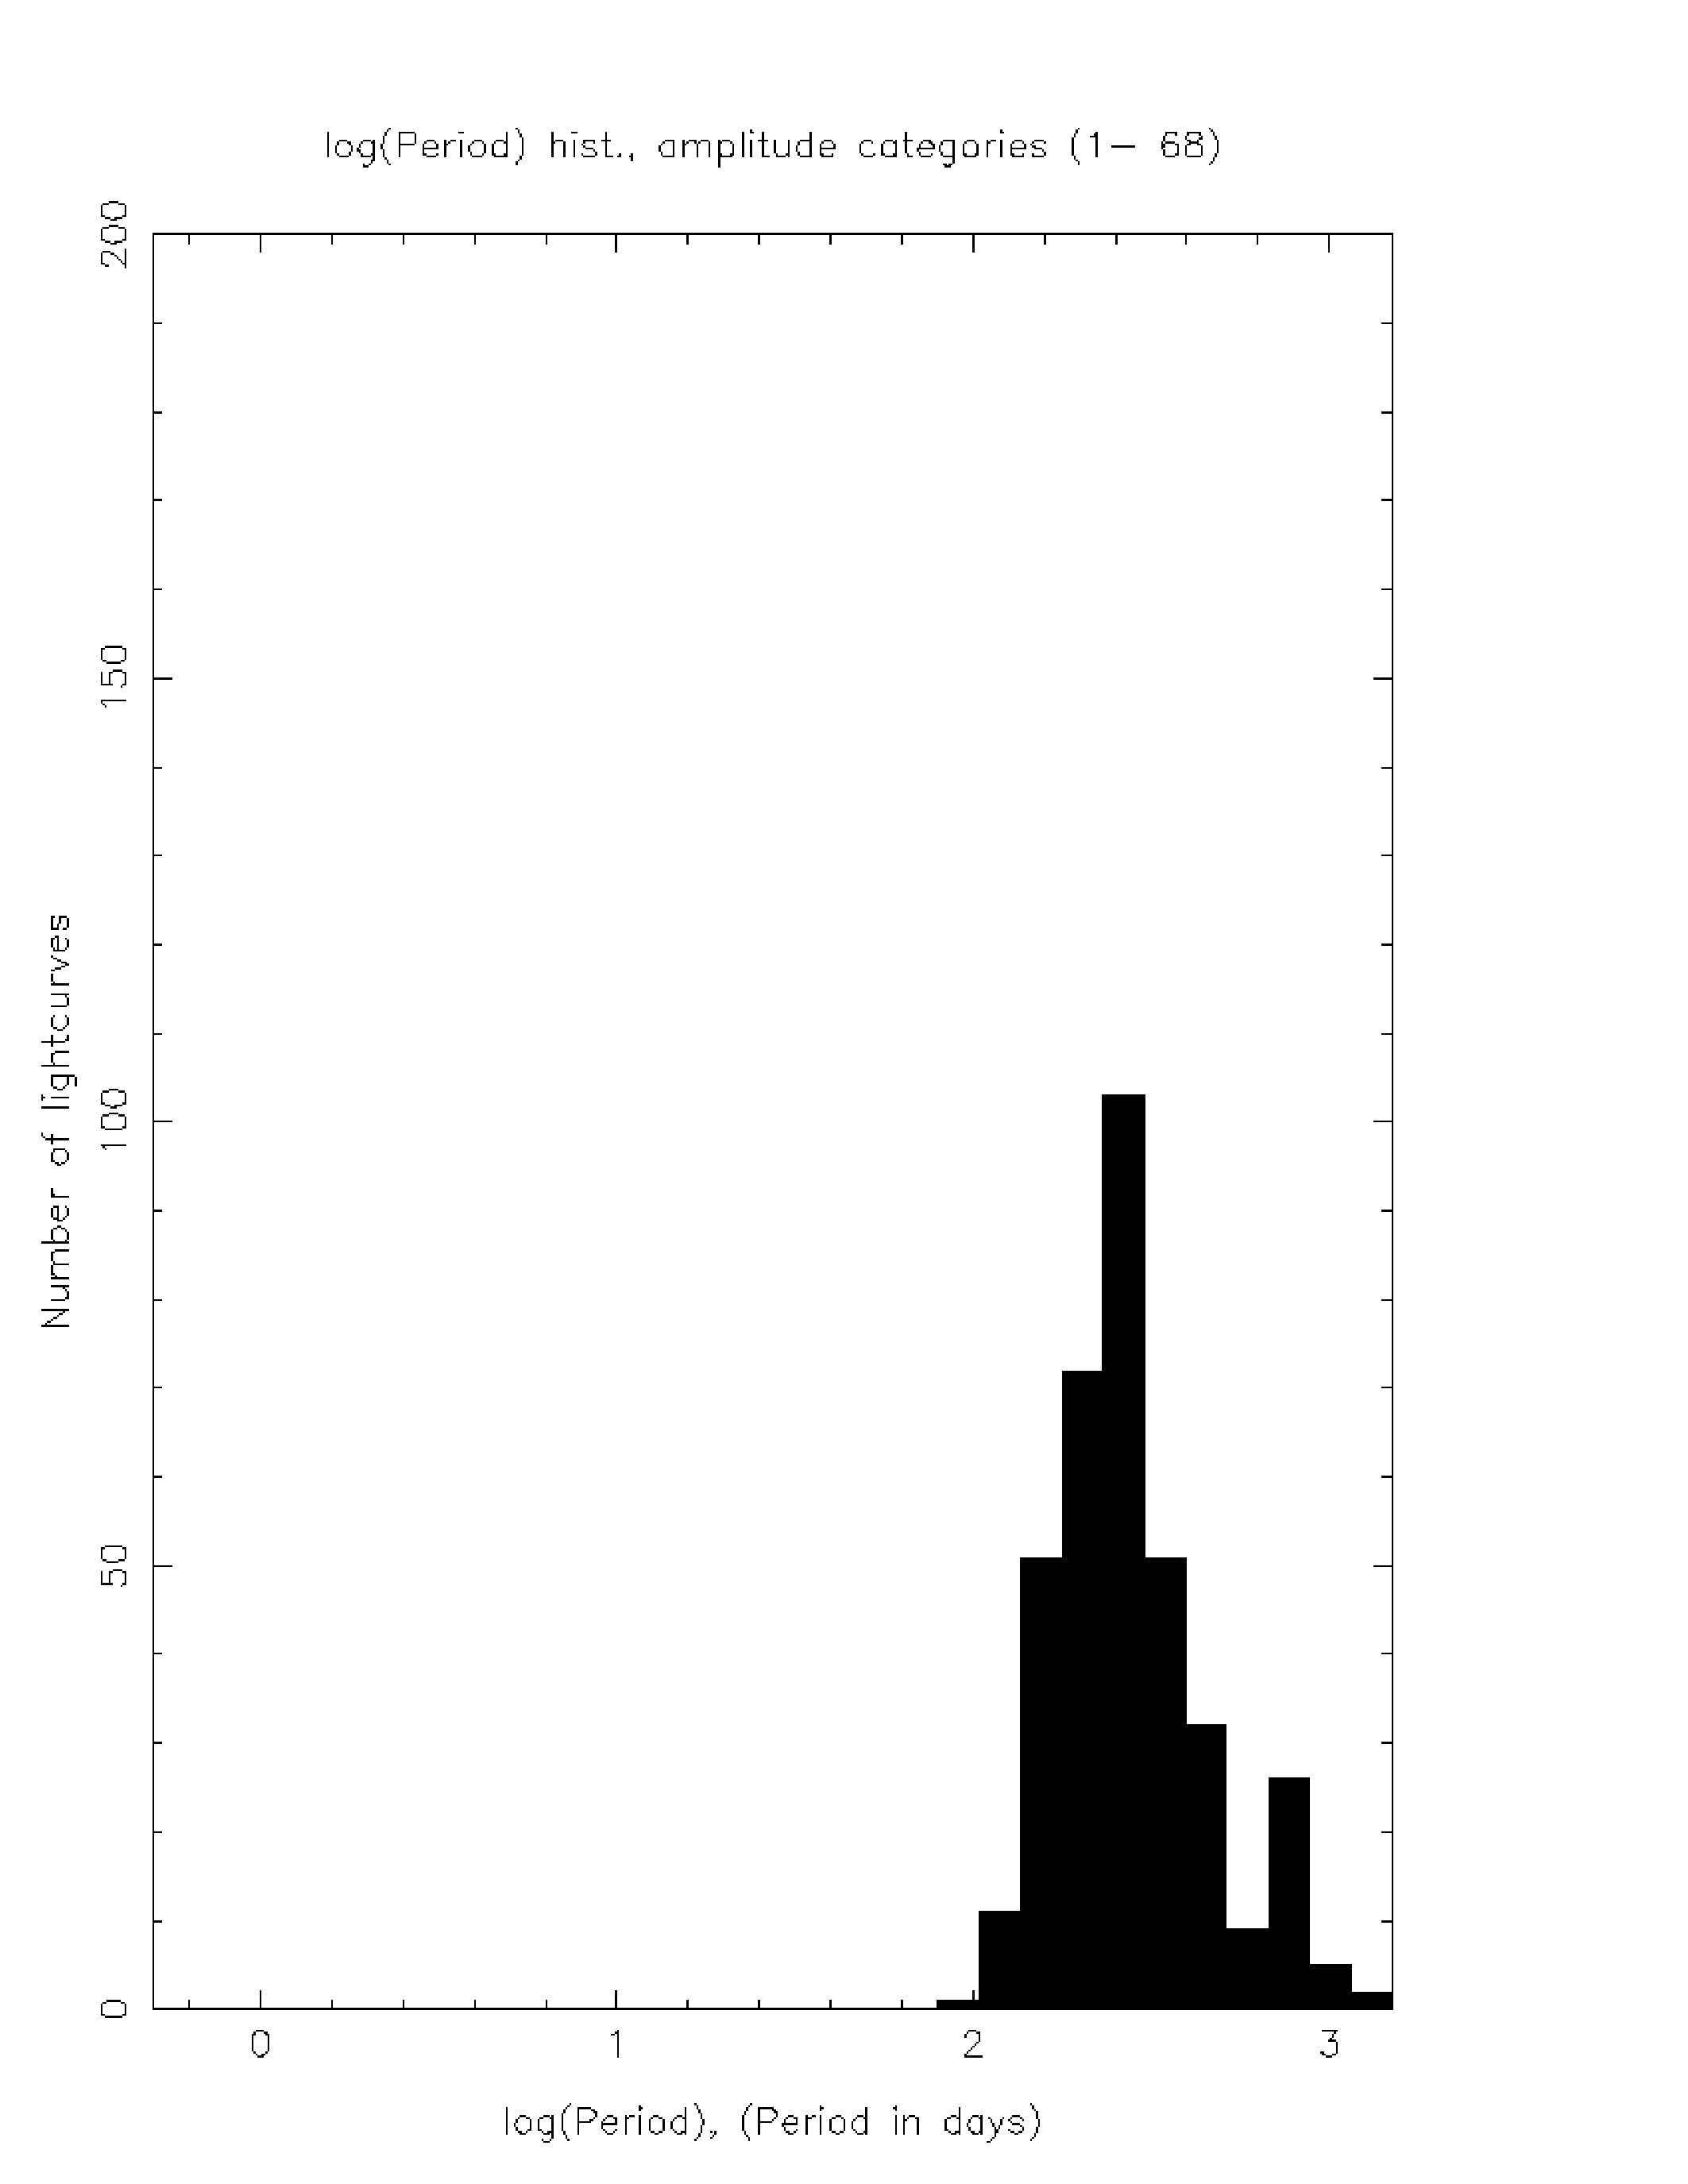} \\
\vspace*{5cm}
   \leavevmode
 \includegraphics{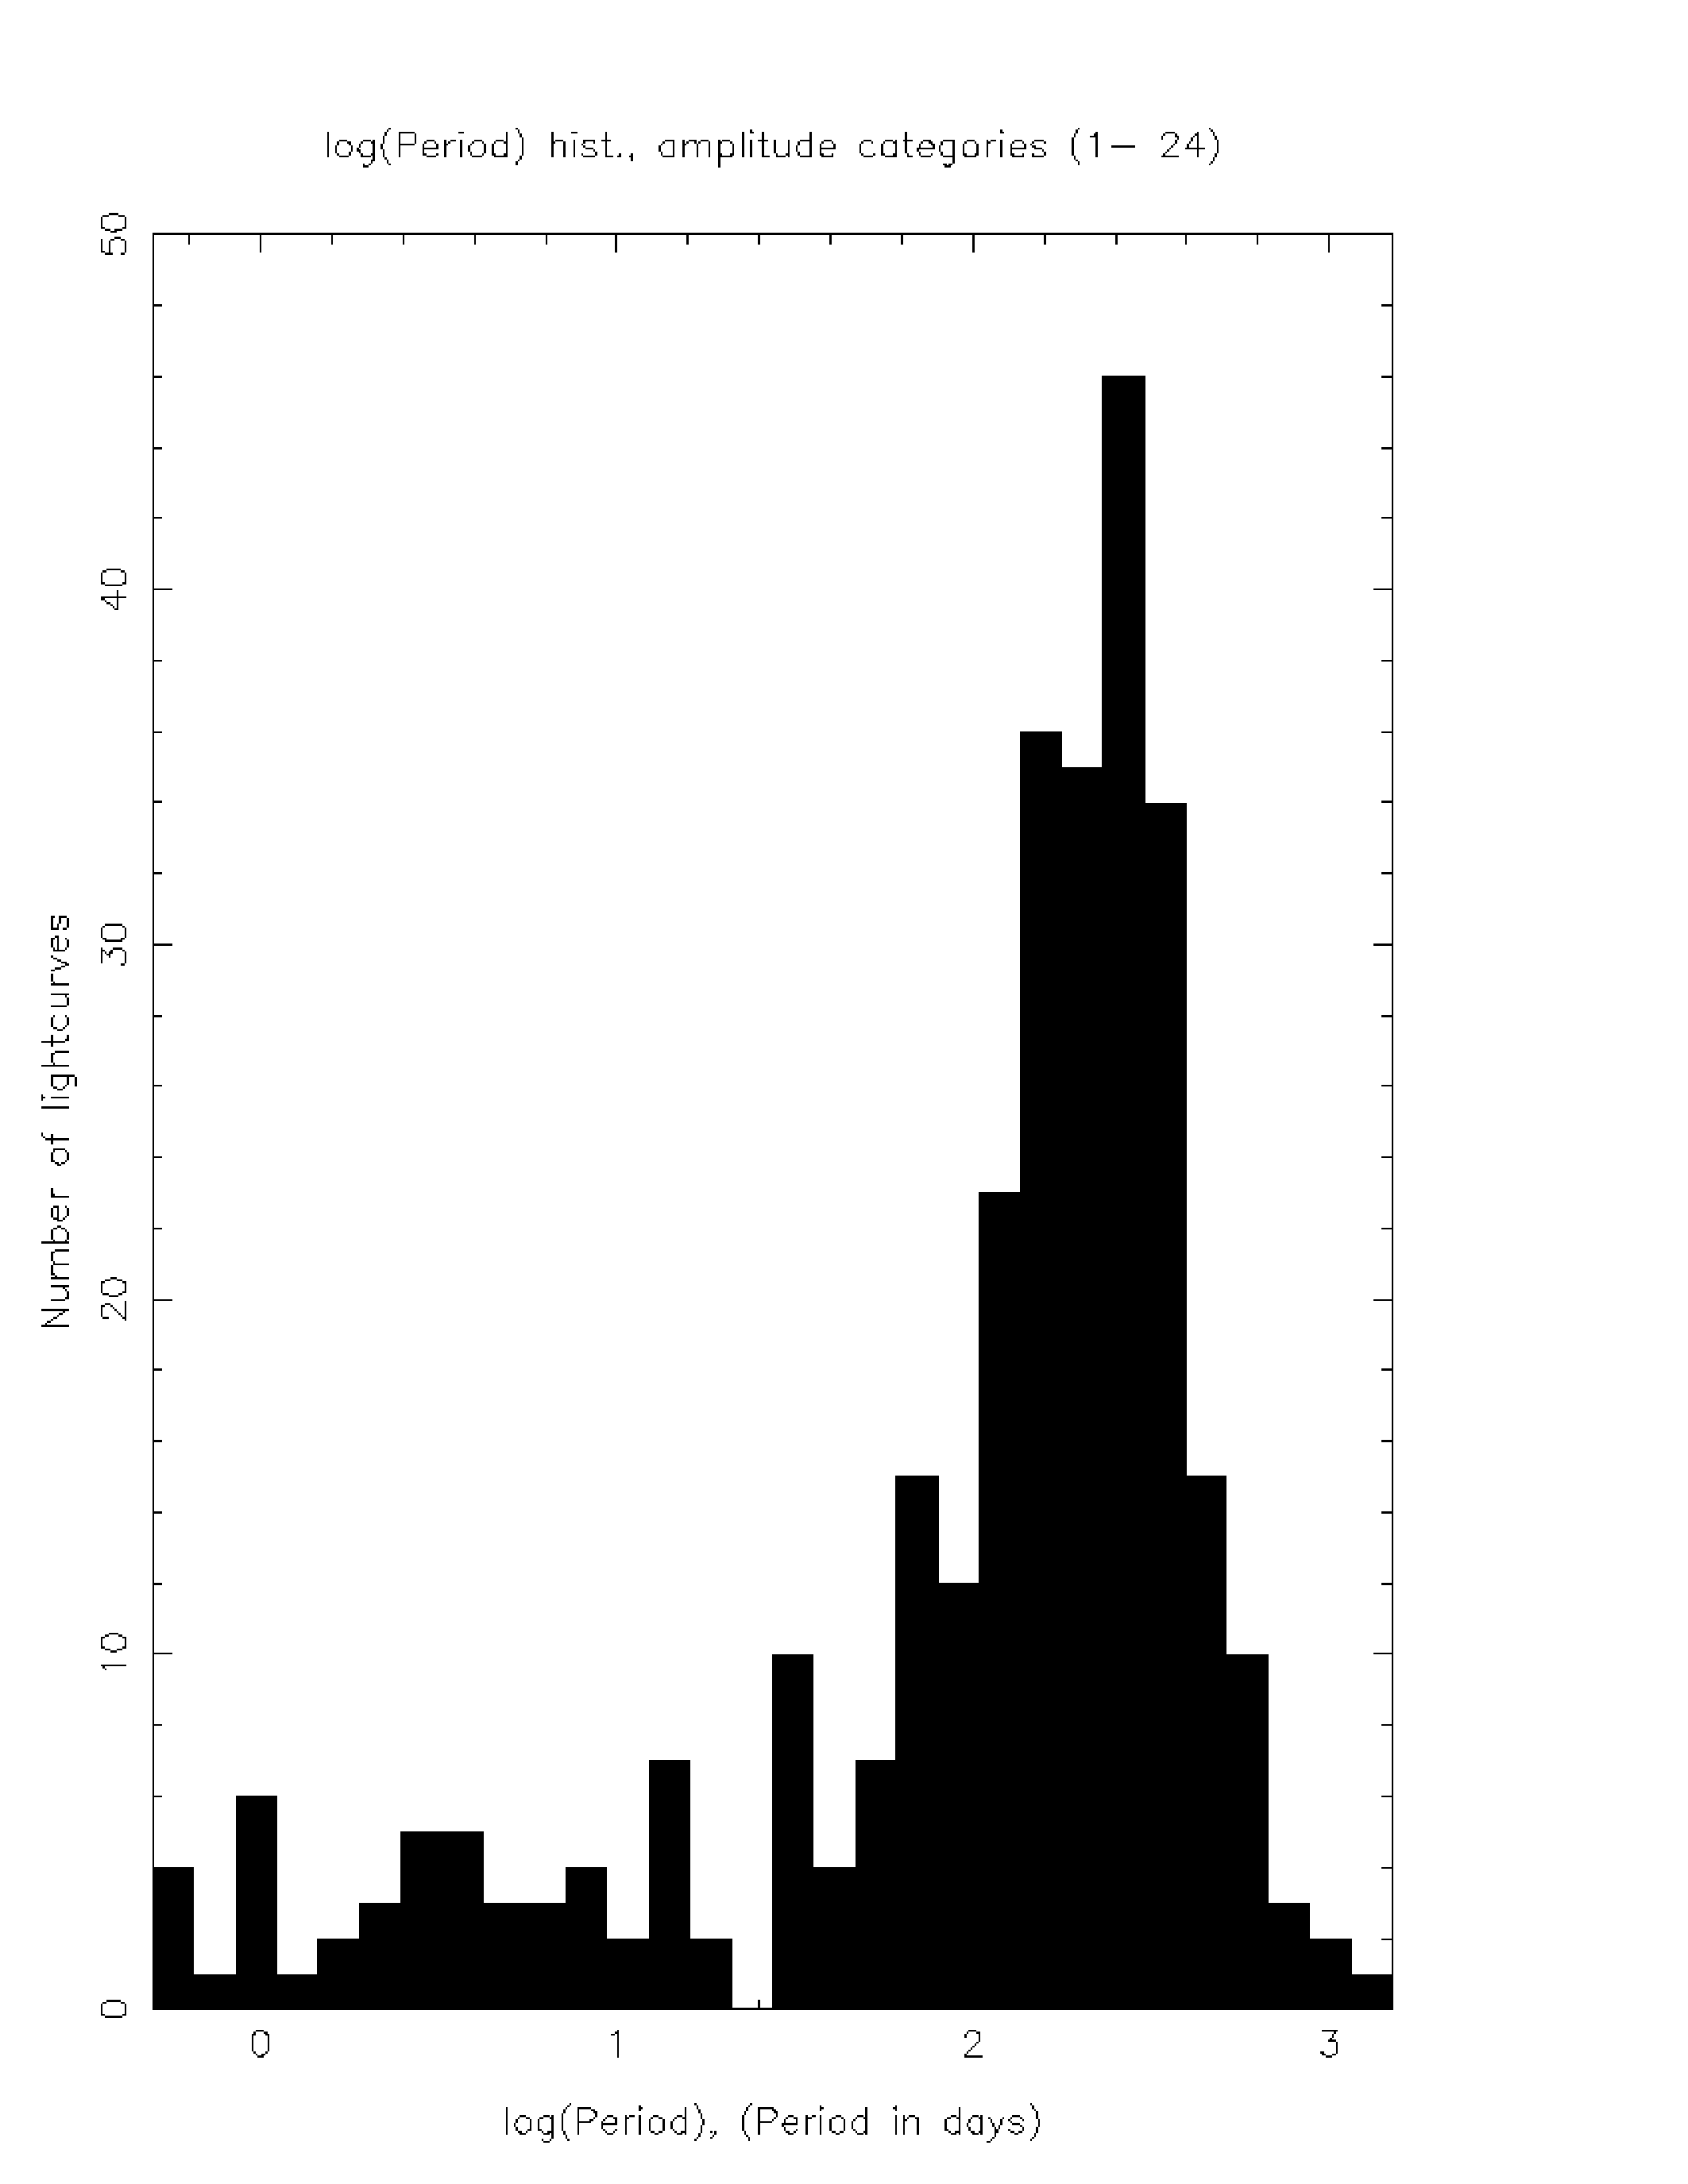} \\
\vspace*{0cm}
   \leavevmode
 \includegraphics{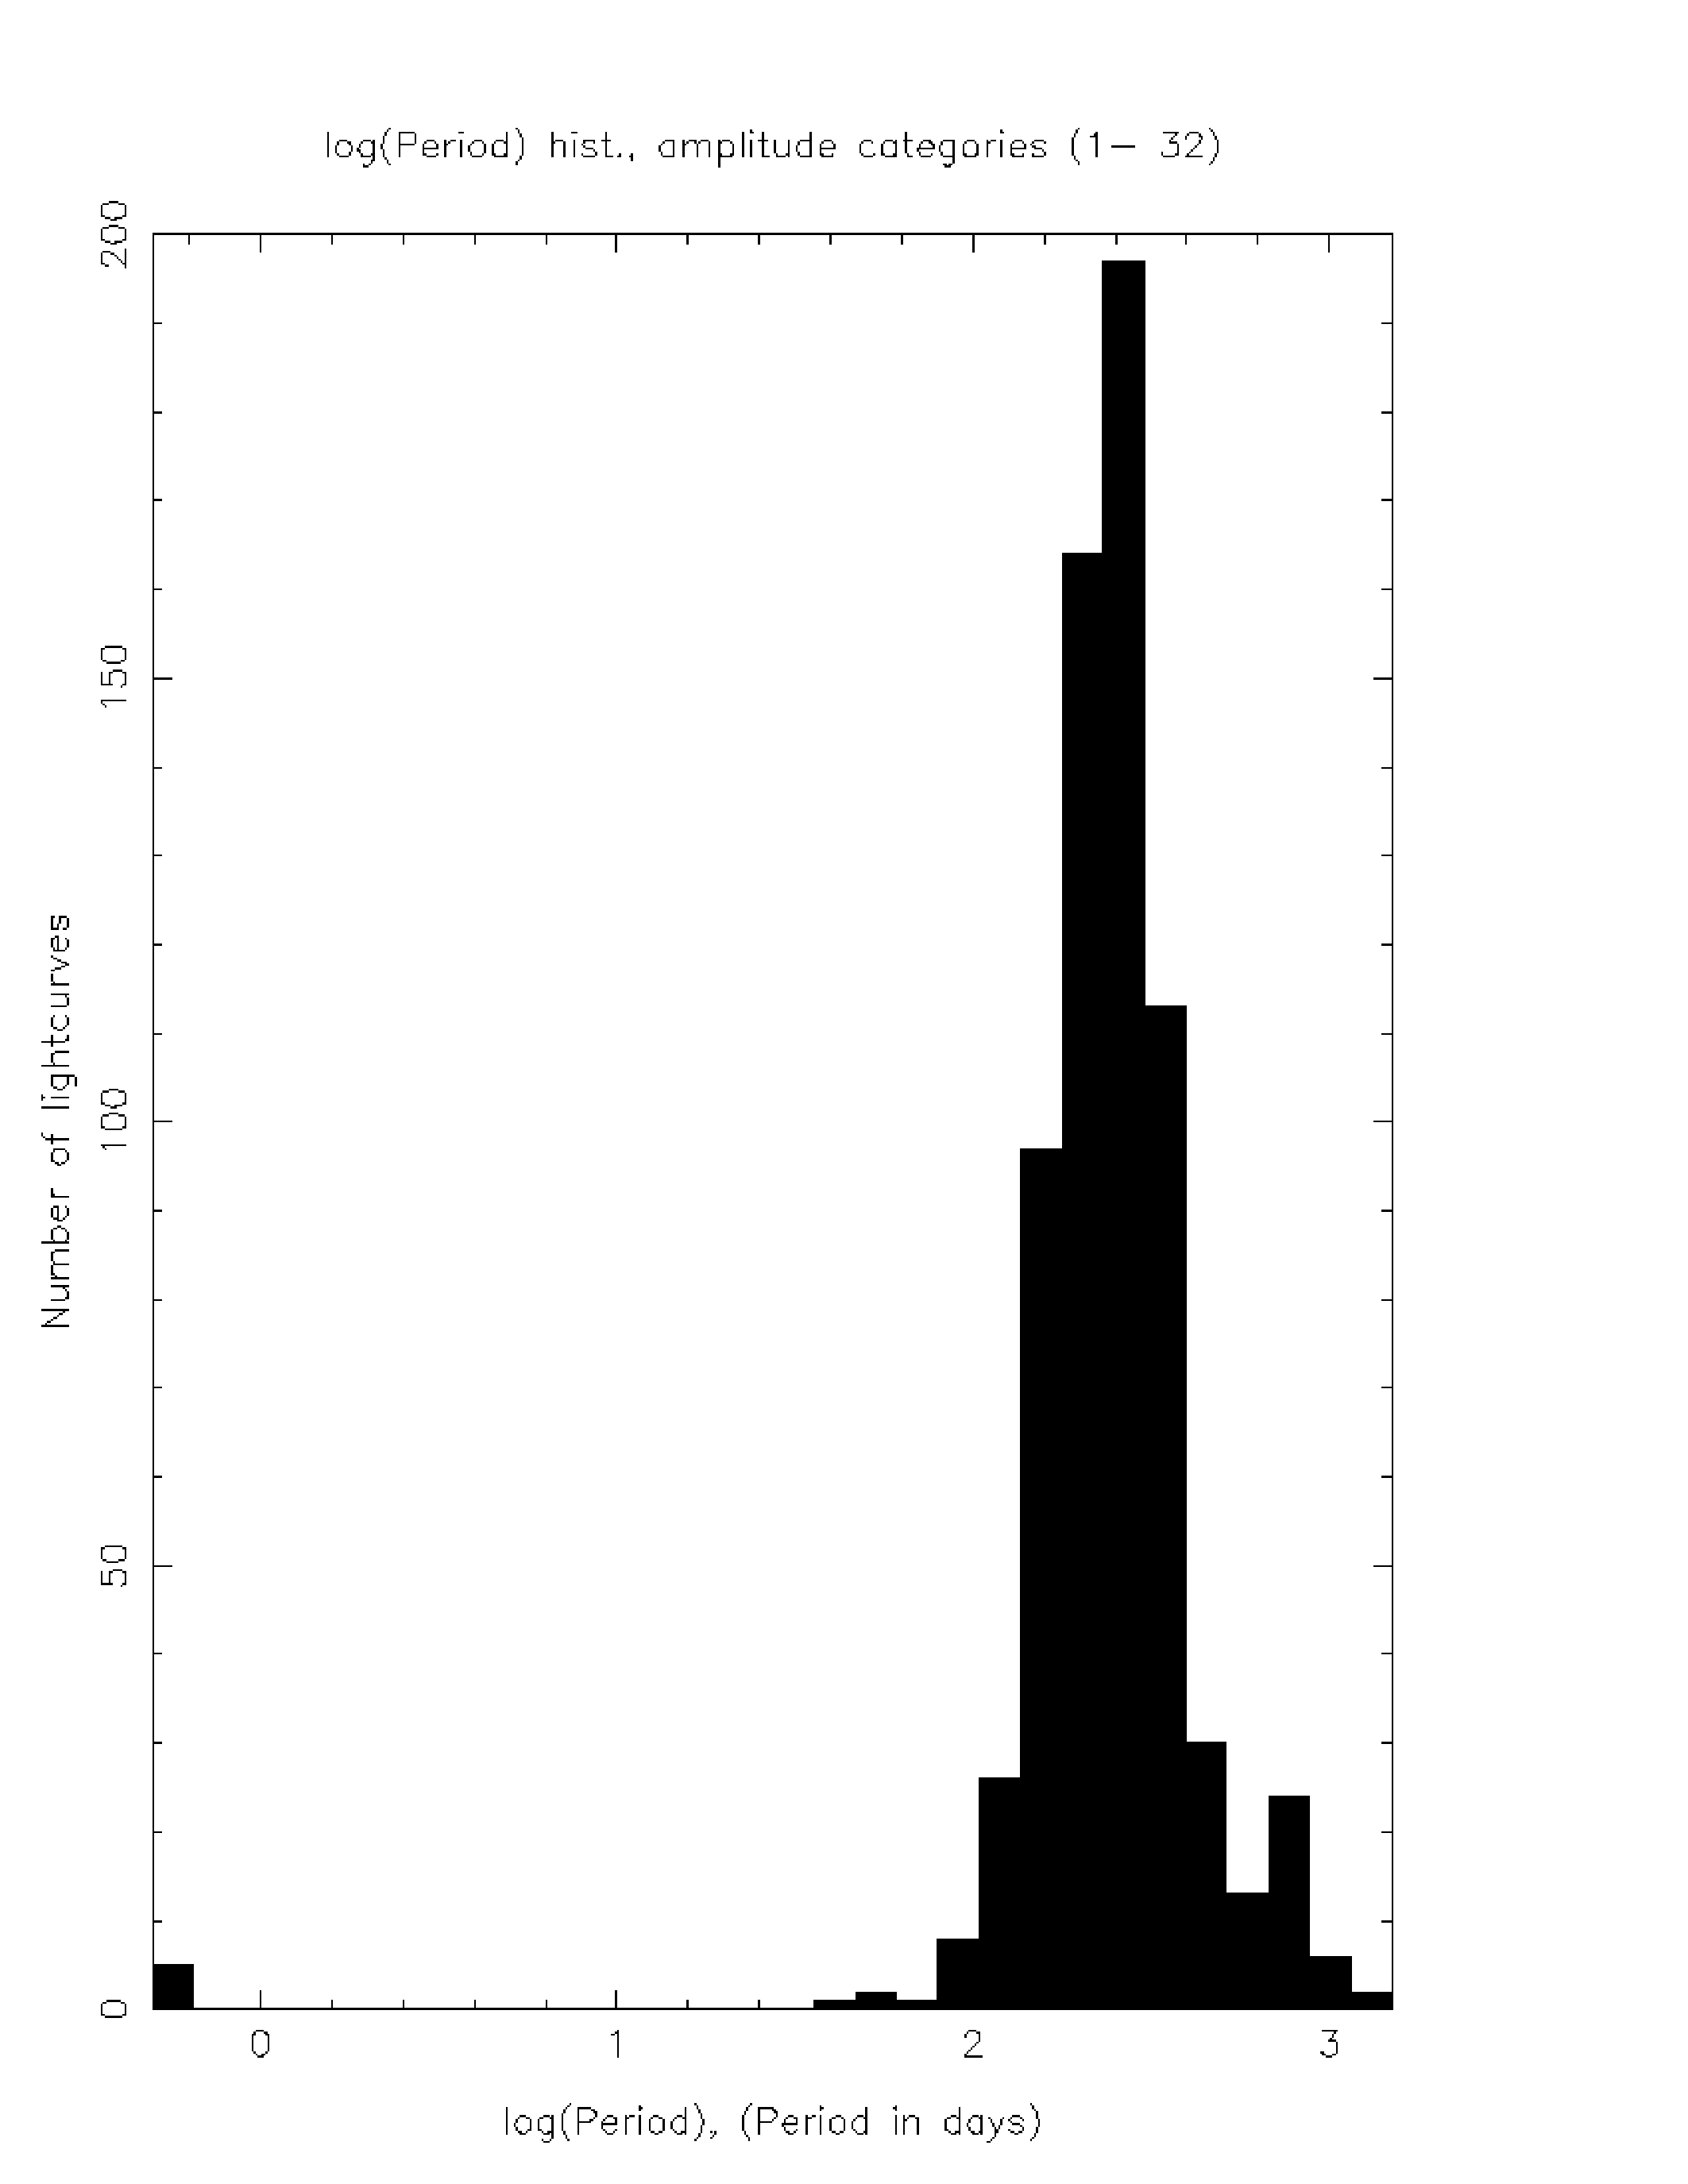} \\
  \end{tabular}
}
\caption[Histograms of variable lightcurve log(Period) distributions: PA/LT flux ratio = 7.89.]{Histograms of variable
 lightcurve log(Period) distributions: PA/LT flux ratio = 7.89; Rows, top to bottom:
1)`variable' lightcurves containing (LT) or (LT + FTN) data only,
2) ``mixed'' lightcurves containing (LT) or (LT + FTN) data only,
3)`variable' lightcurves containing (PA + LT) or (PA + LT + FTN) data,
4) ``mixed'' lightcurves containing (PA + LT) or (PA + LT + FTN) data.
Columns, left to right: Flux amplitudes, 1) 0-5, 2) 5-`MAX' 3) Sum of all categories
`MAX' varies with row as: 1) 31 2) 68 3) 24 4) 32 .}
 \label{Log(P)_all_categories_low_ratio}
\end{figure}

\newpage

\begin{figure}
\vspace*{4cm}
\center{
  \begin{tabular}{ccc}
% 0-5
\vspace*{5cm}
   \leavevmode
 \includegraphics{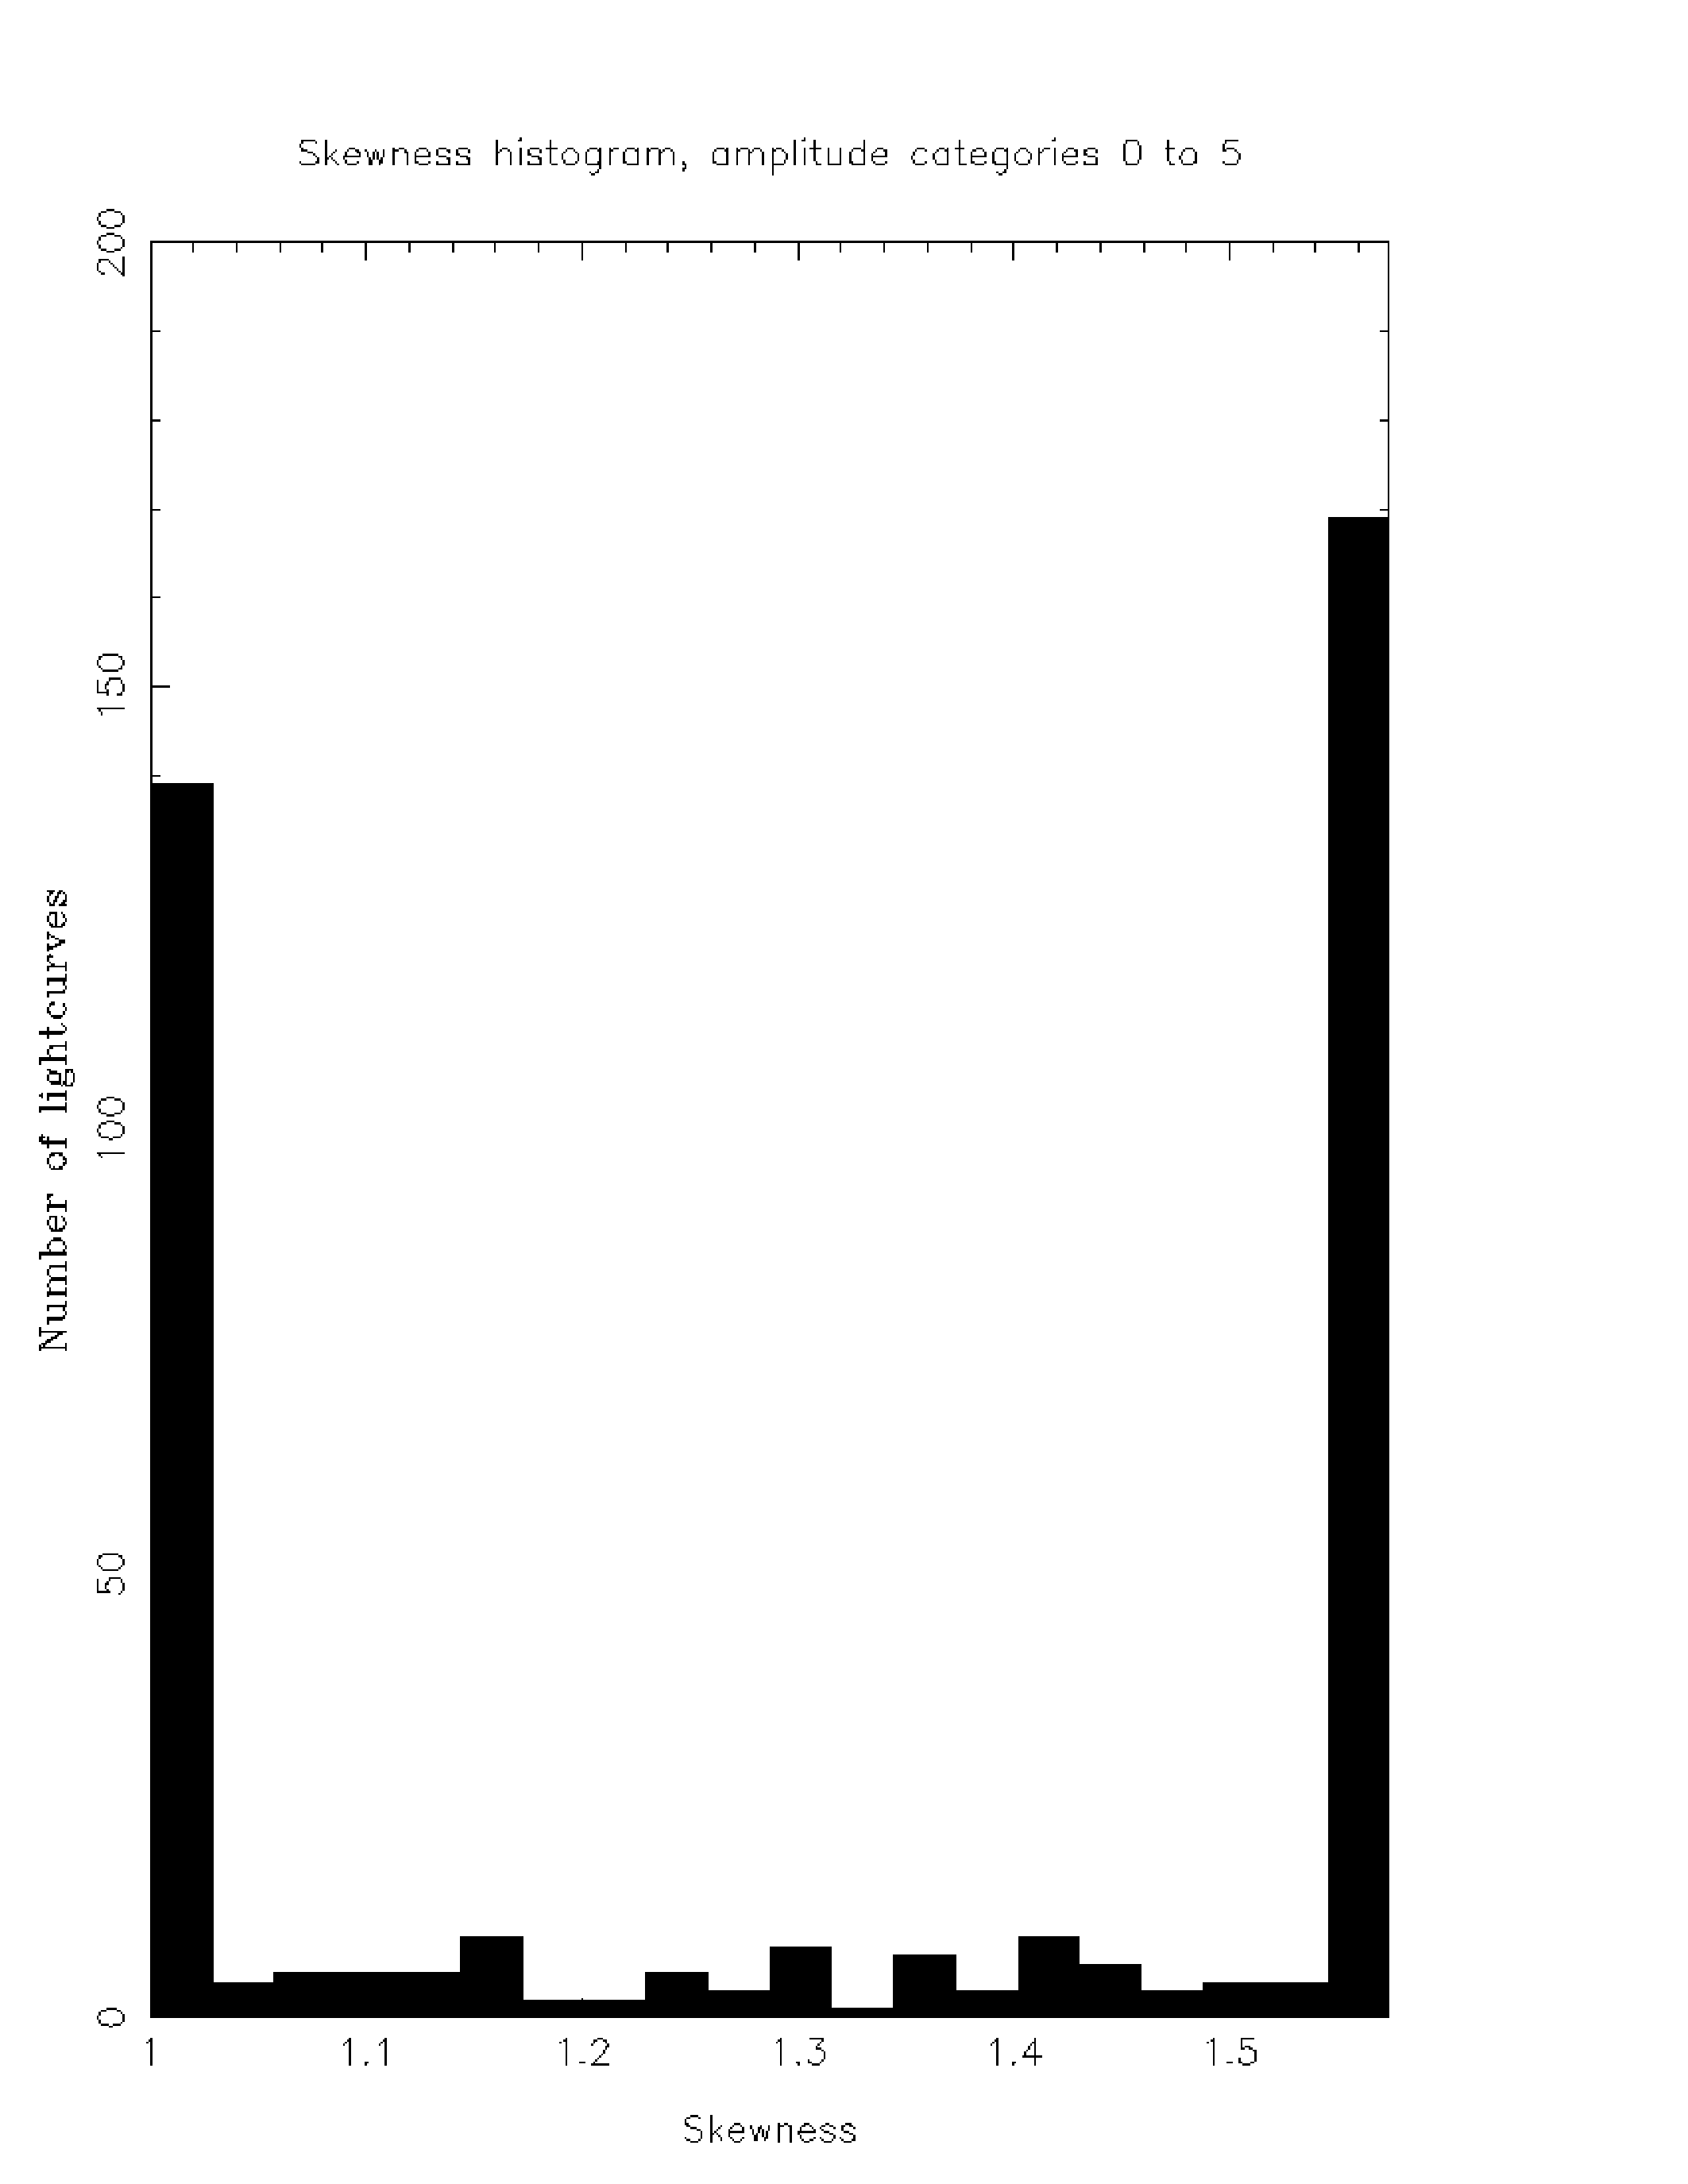} \\
\vspace*{5cm}
   \leavevmode
 \includegraphics{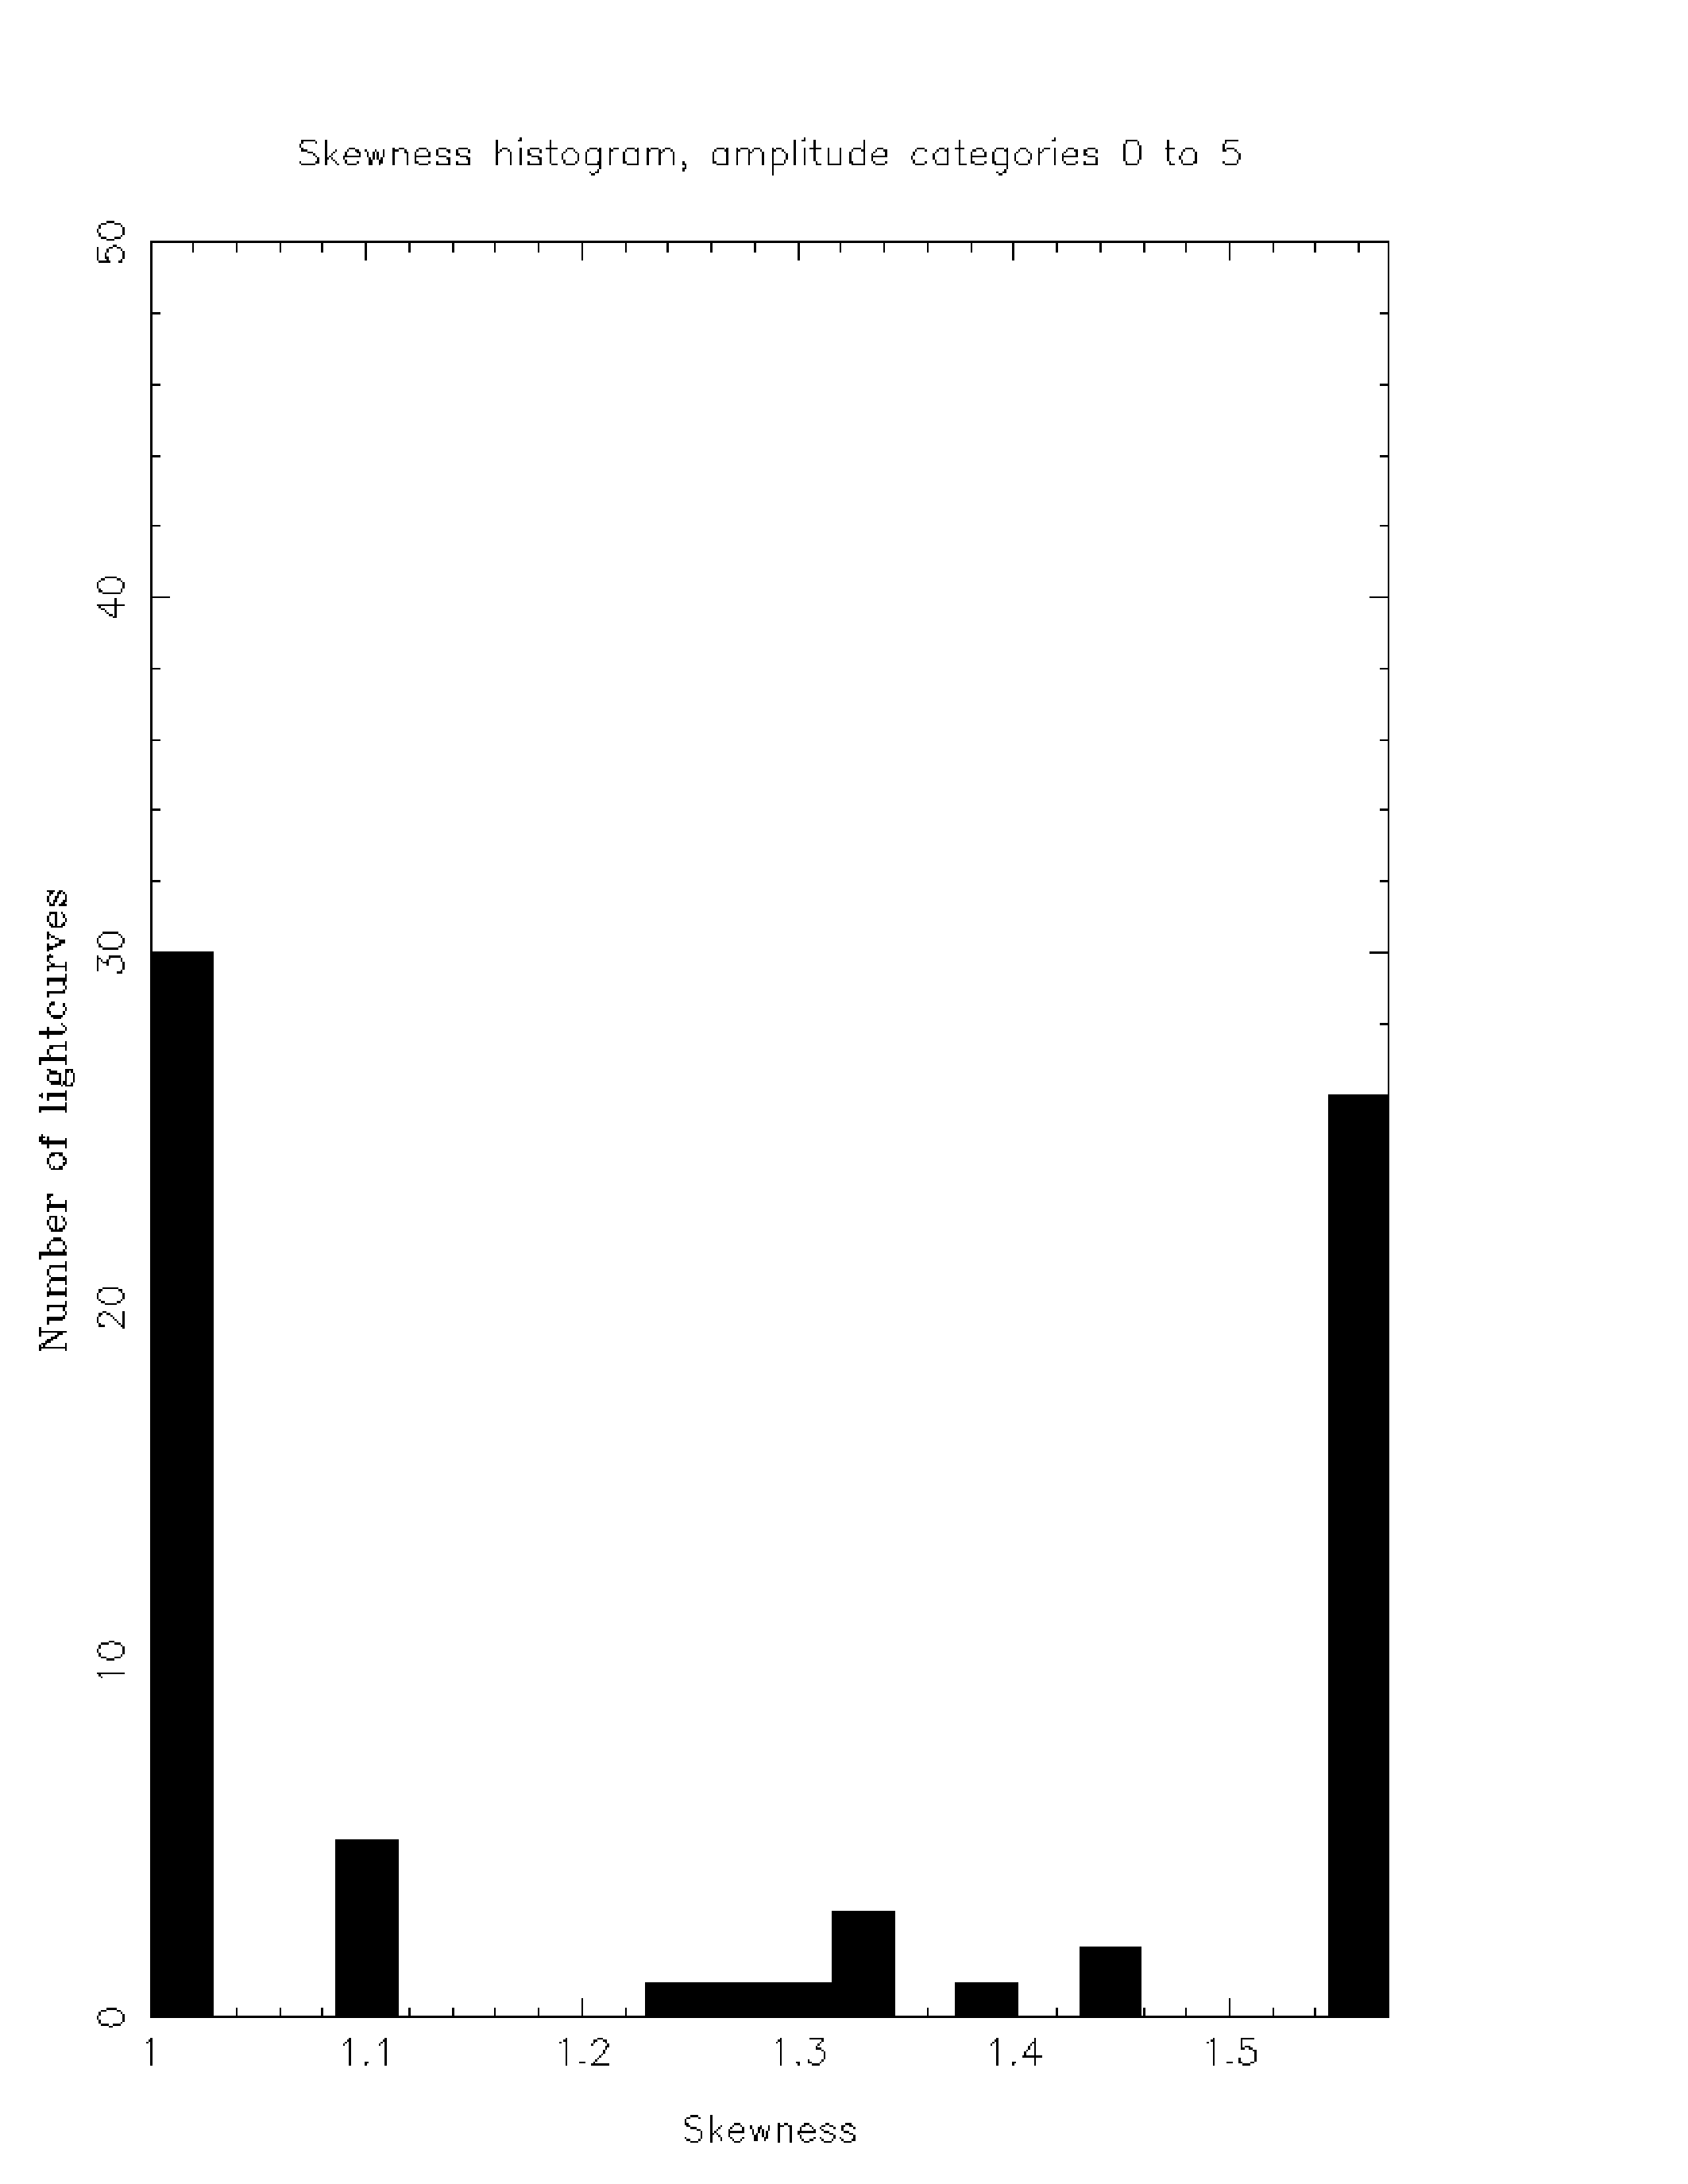} \\
\vspace*{5cm}
   \leavevmode
 \includegraphics{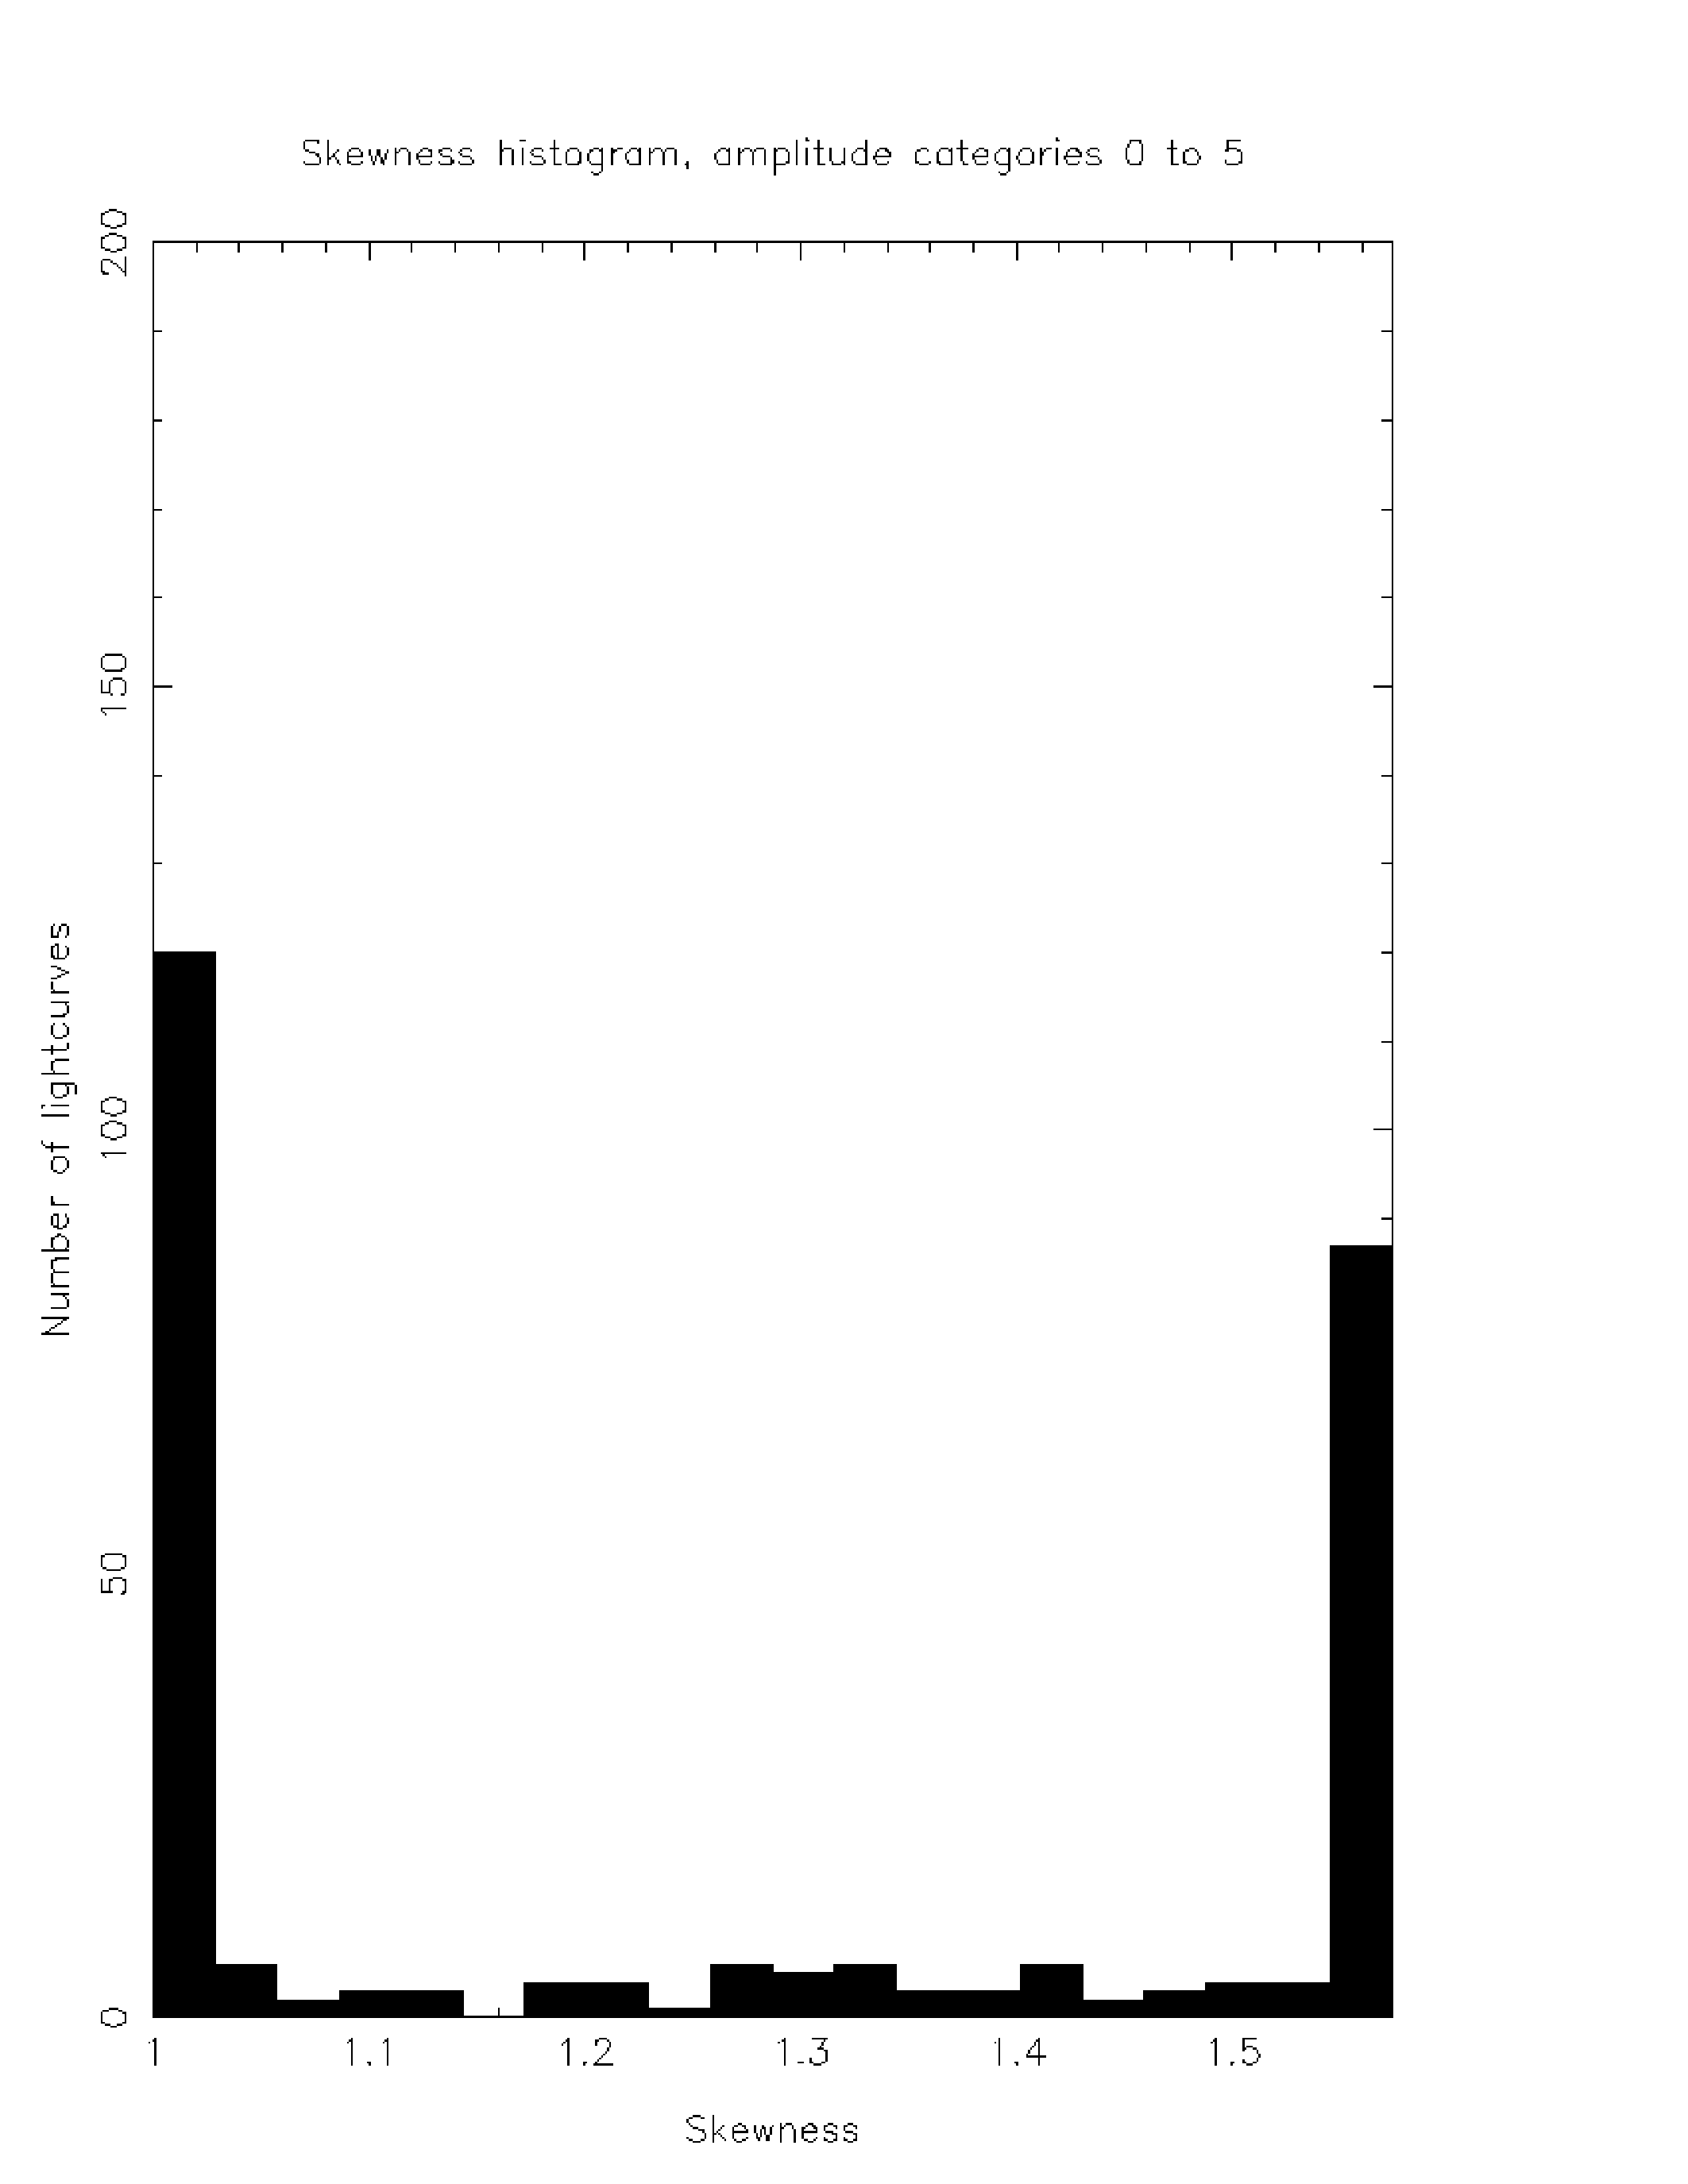} \\
\vspace*{0cm}
   \leavevmode
 \includegraphics{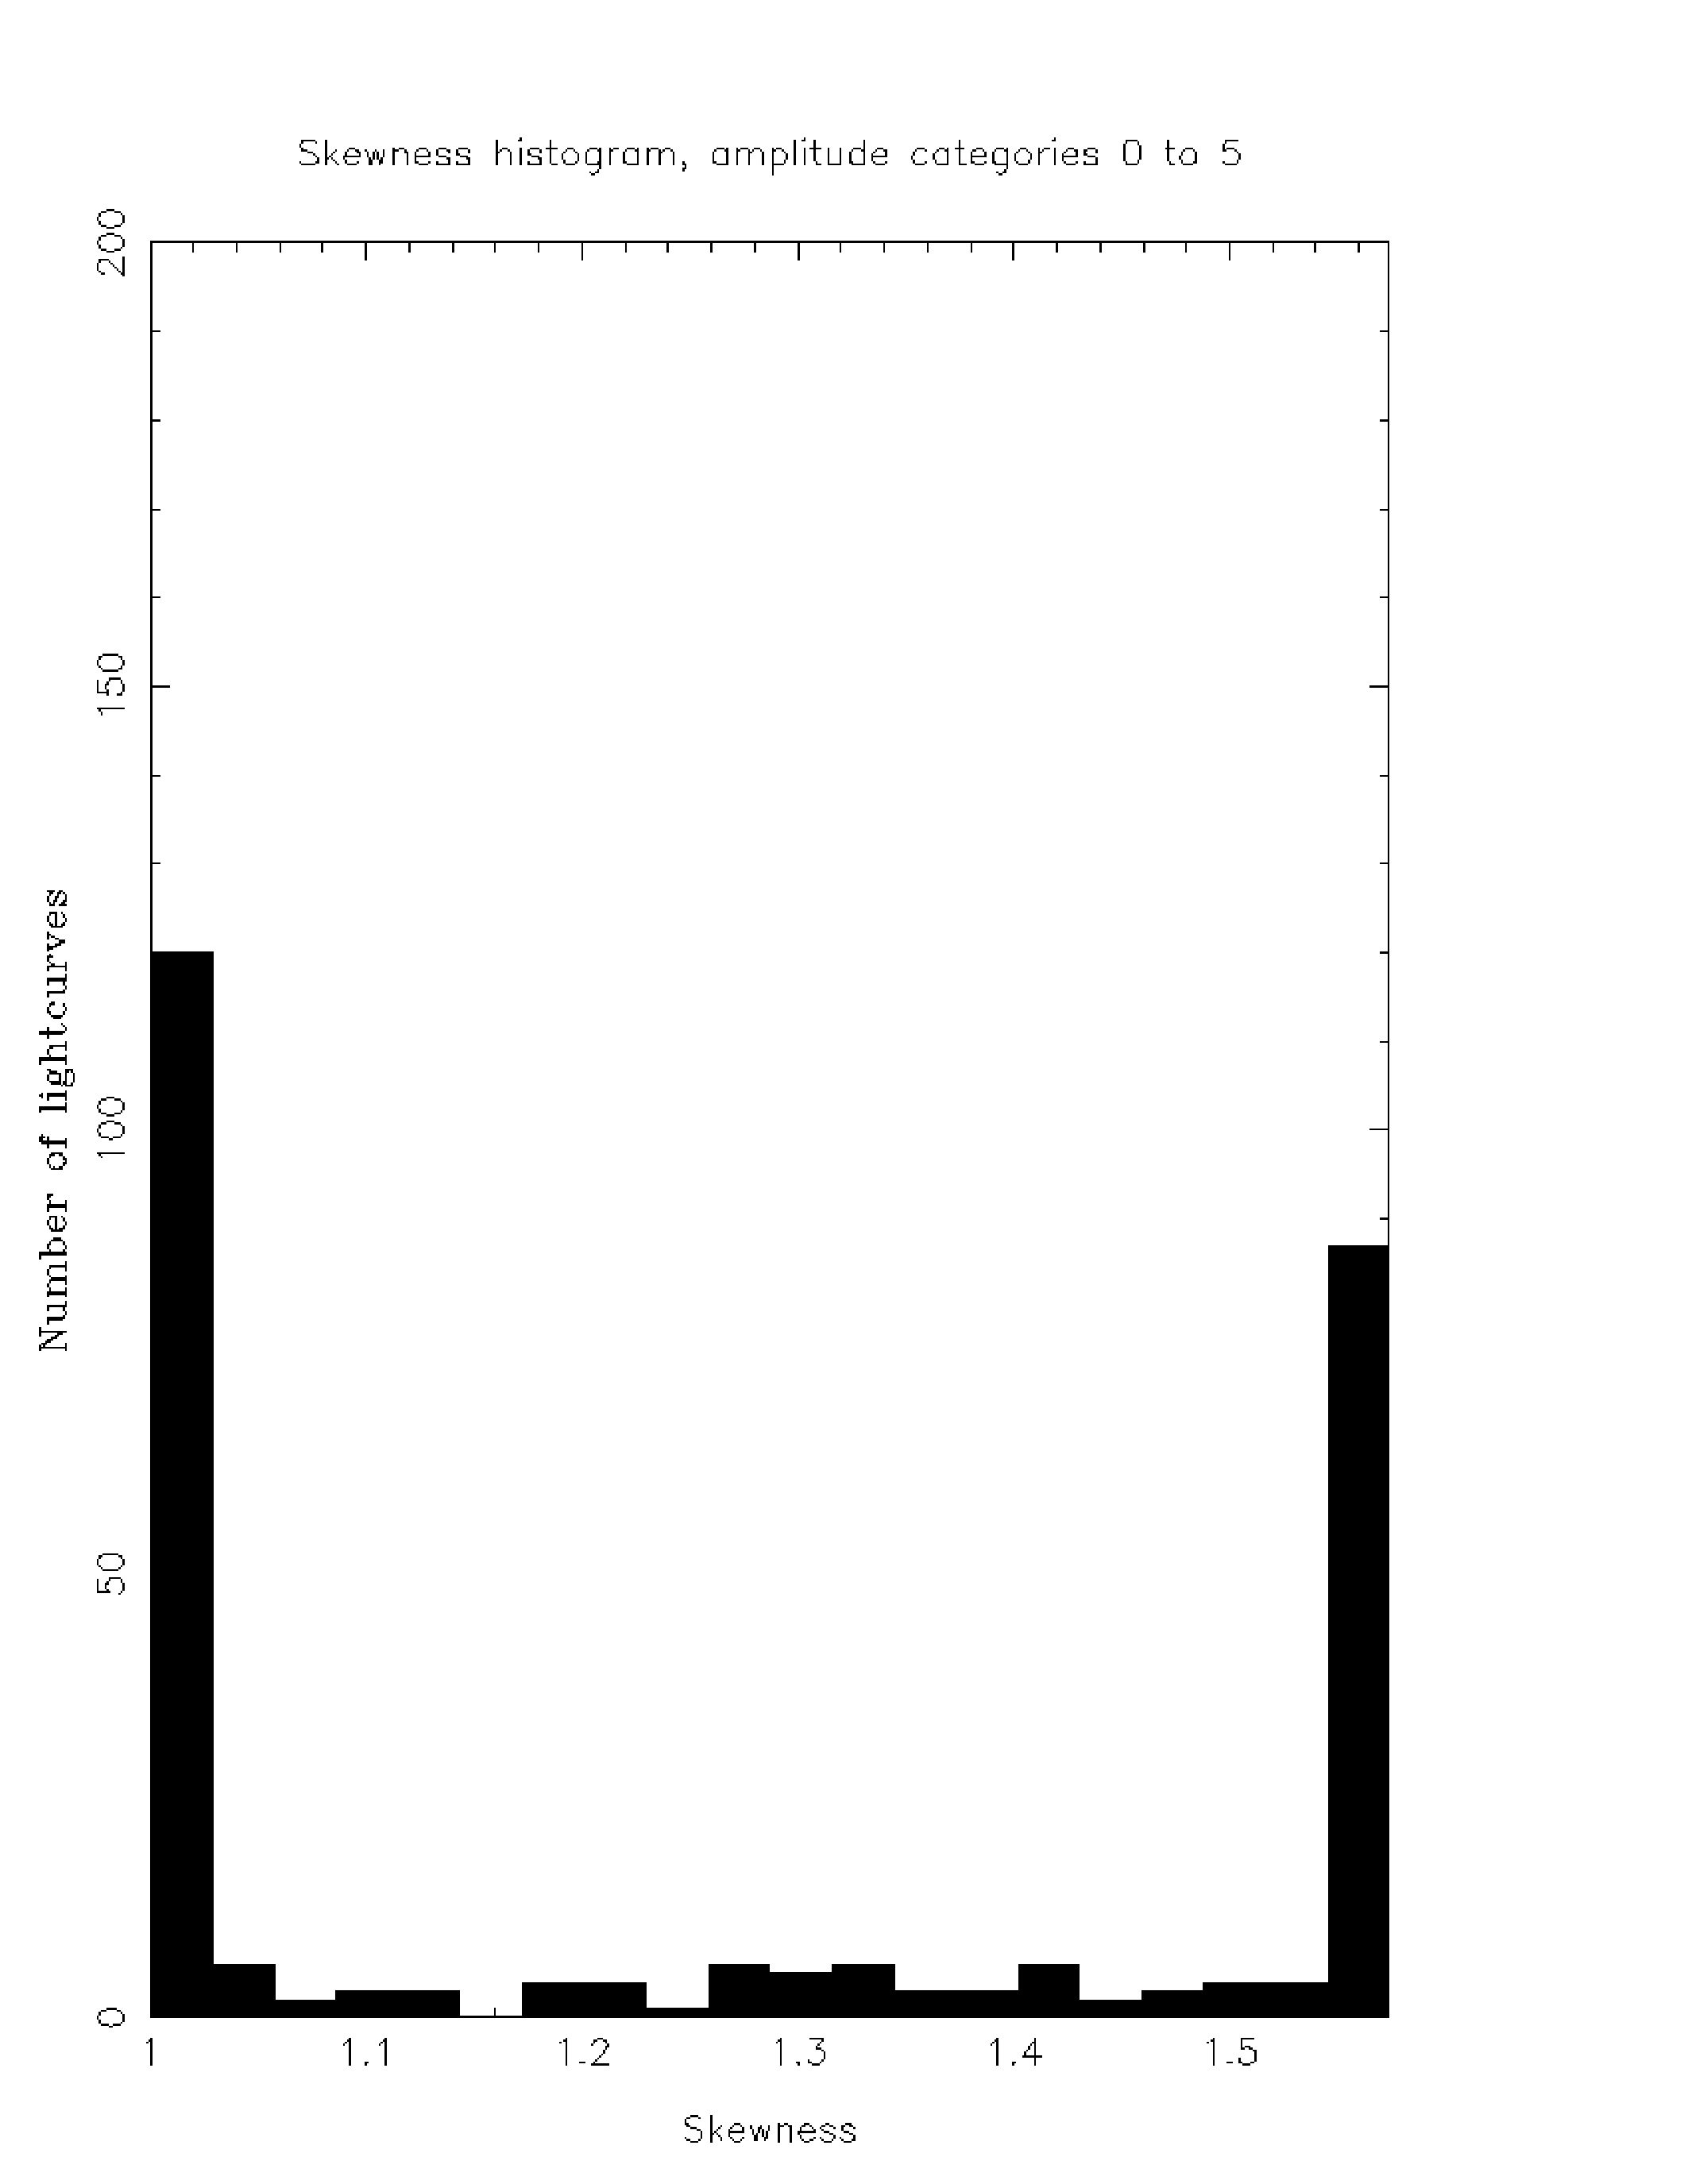} \\
  \end{tabular}
 %}
\hspace*{4cm}
  \begin{tabular}{ccc}
% 5 - whatever
\vspace*{5cm}
   \leavevmode
 \includegraphics{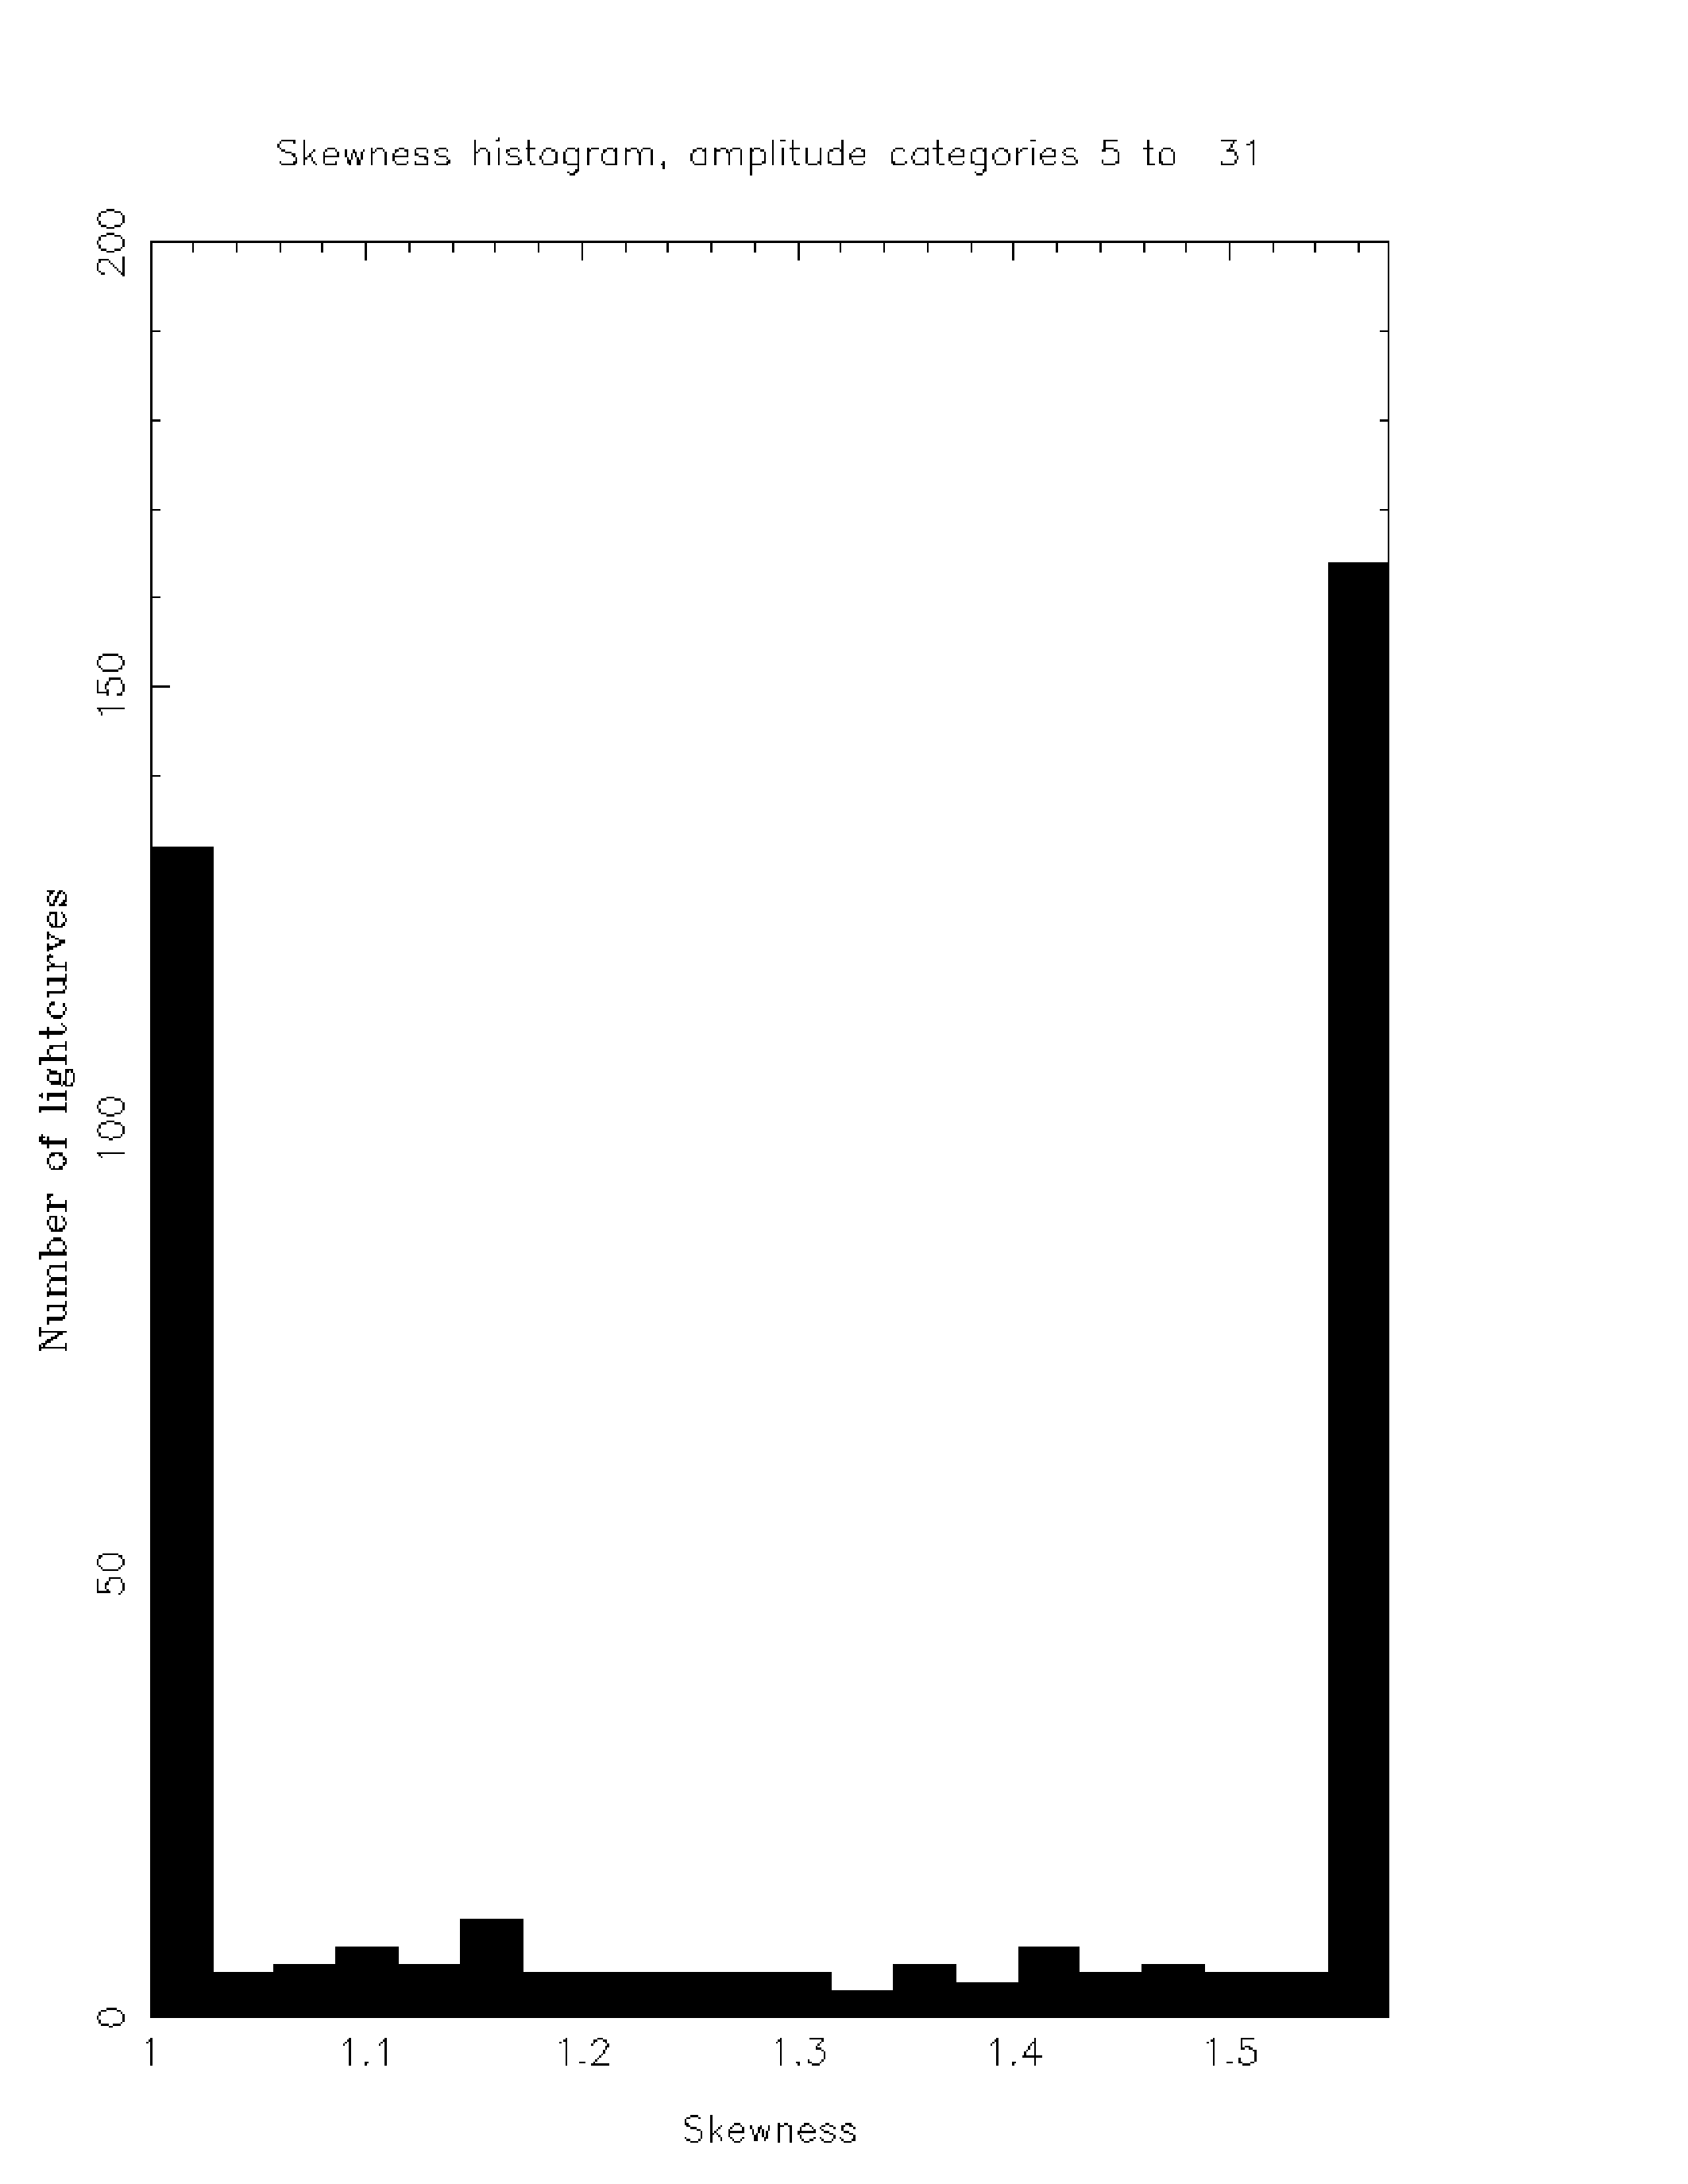} \\
 \vspace*{5cm}
   \leavevmode
\includegraphics{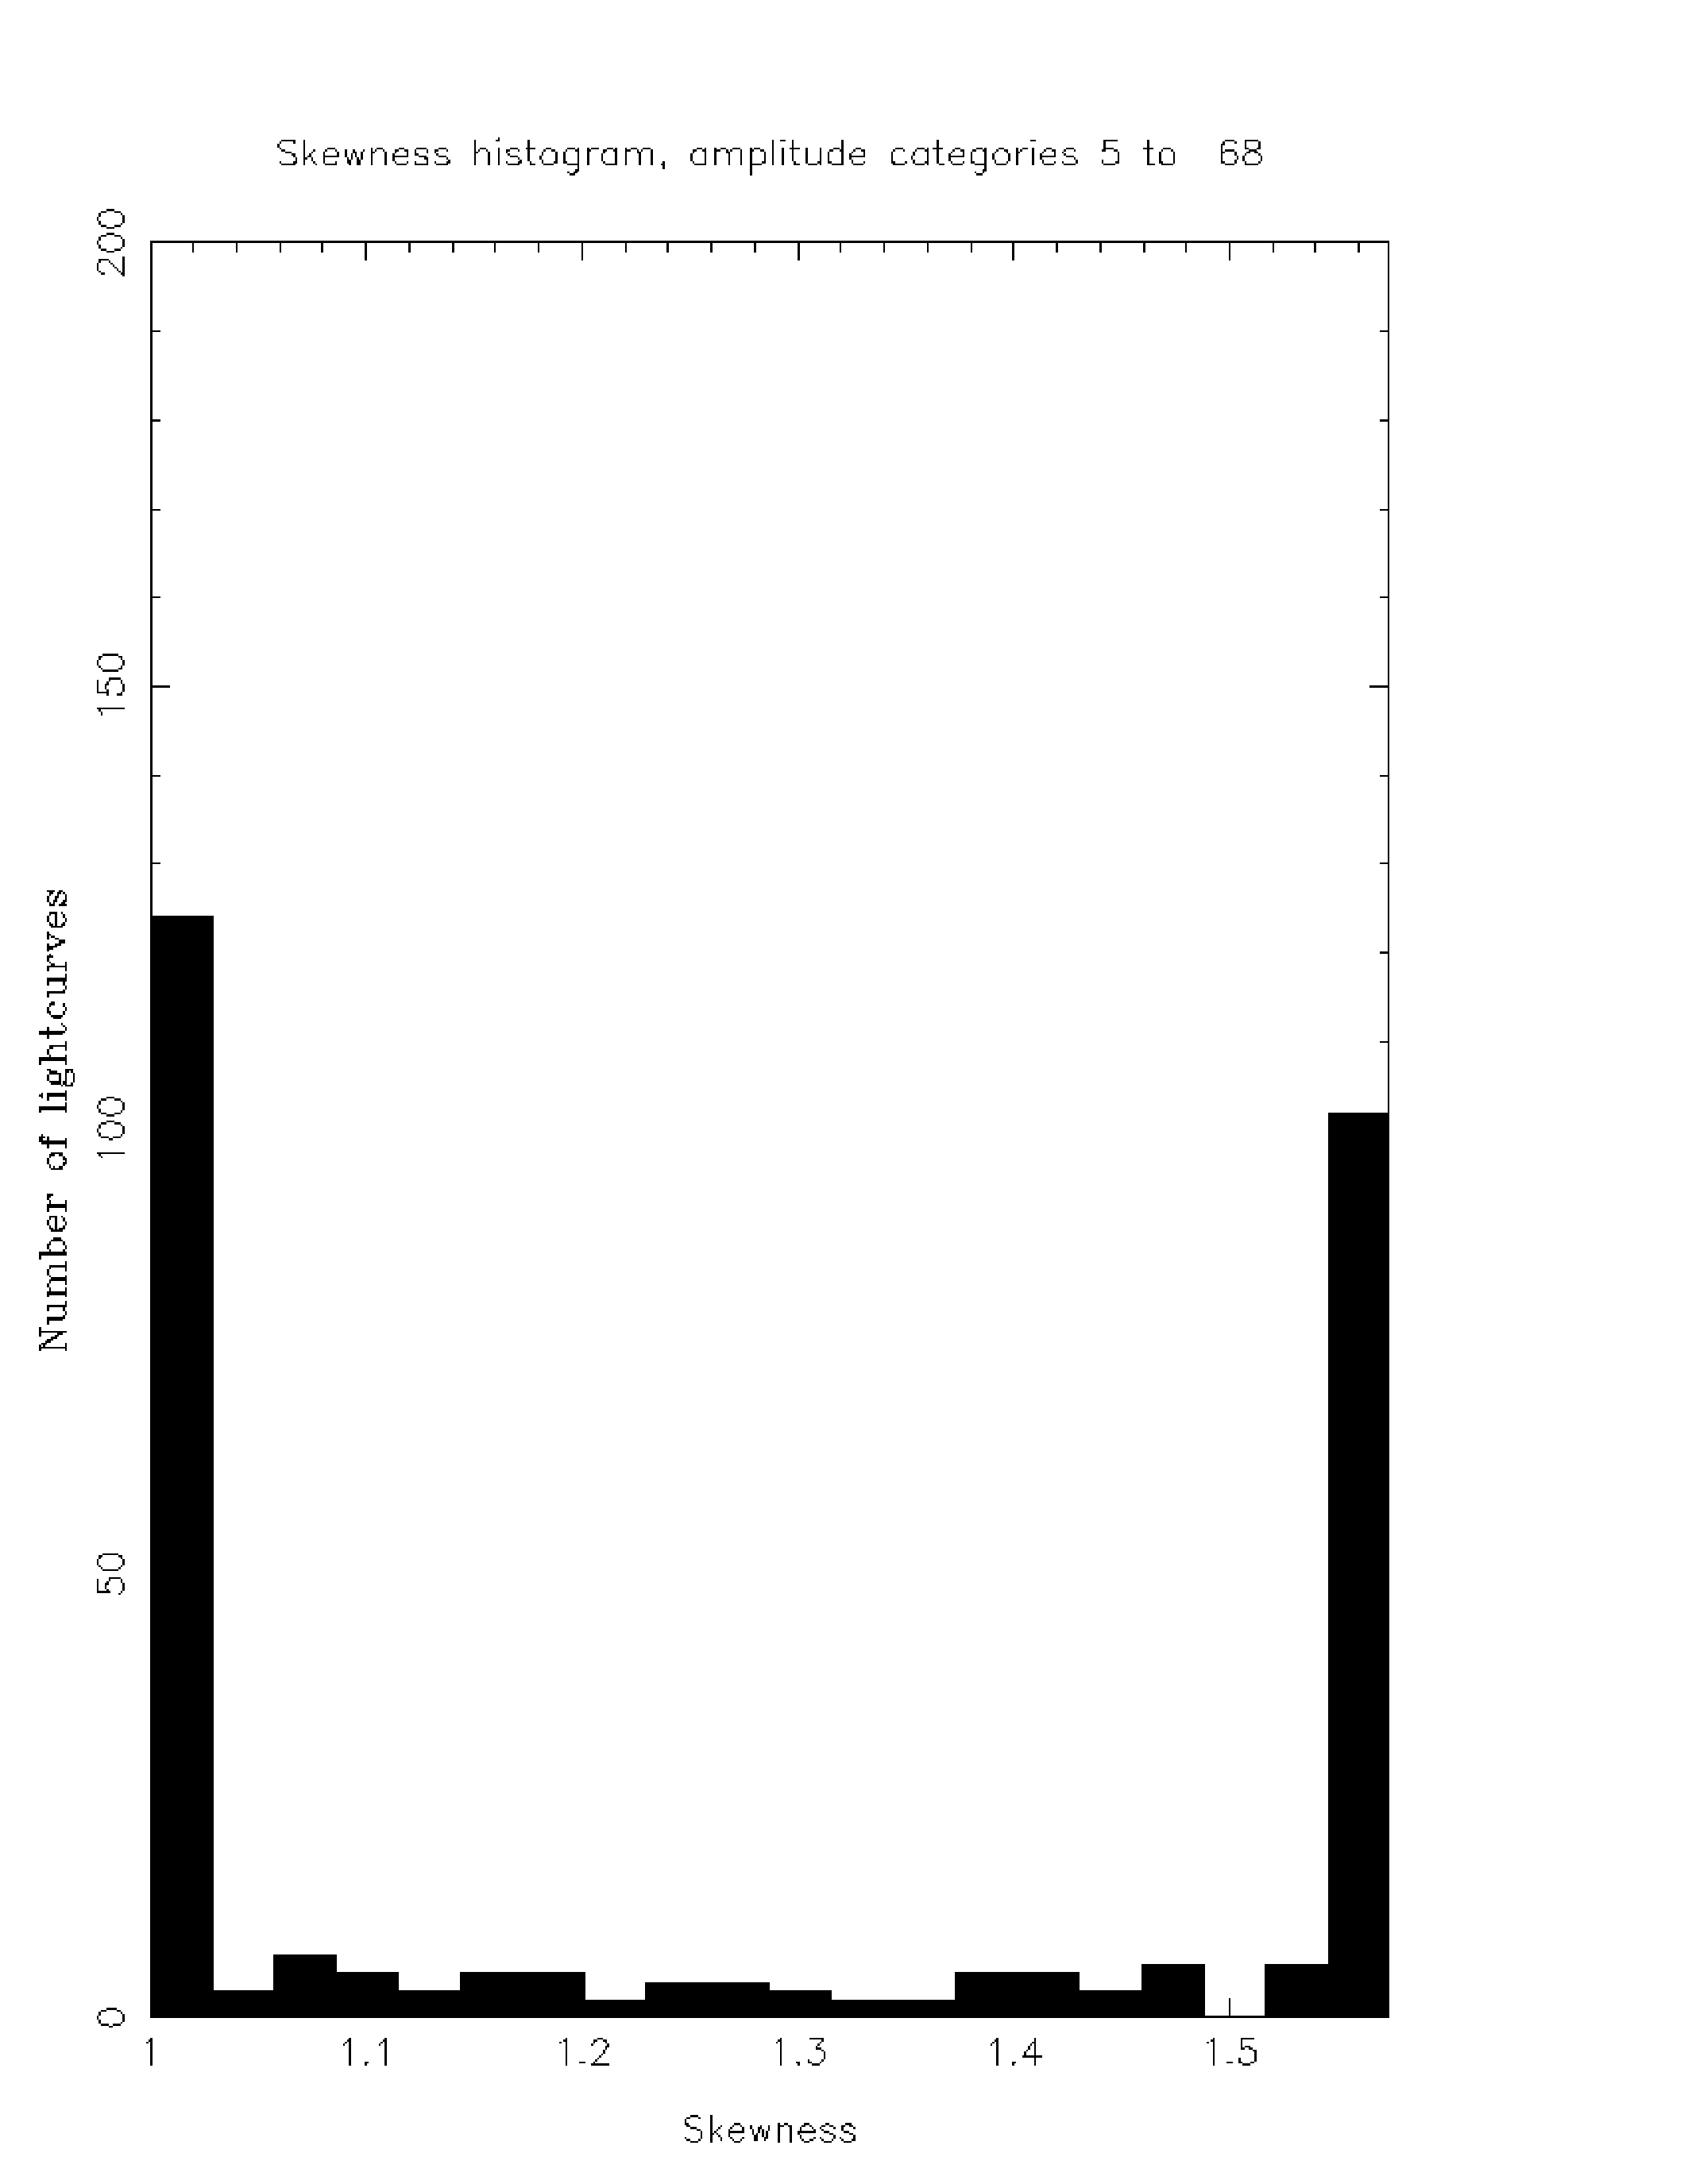} \\
\vspace*{5cm}
   \leavevmode
 \includegraphics{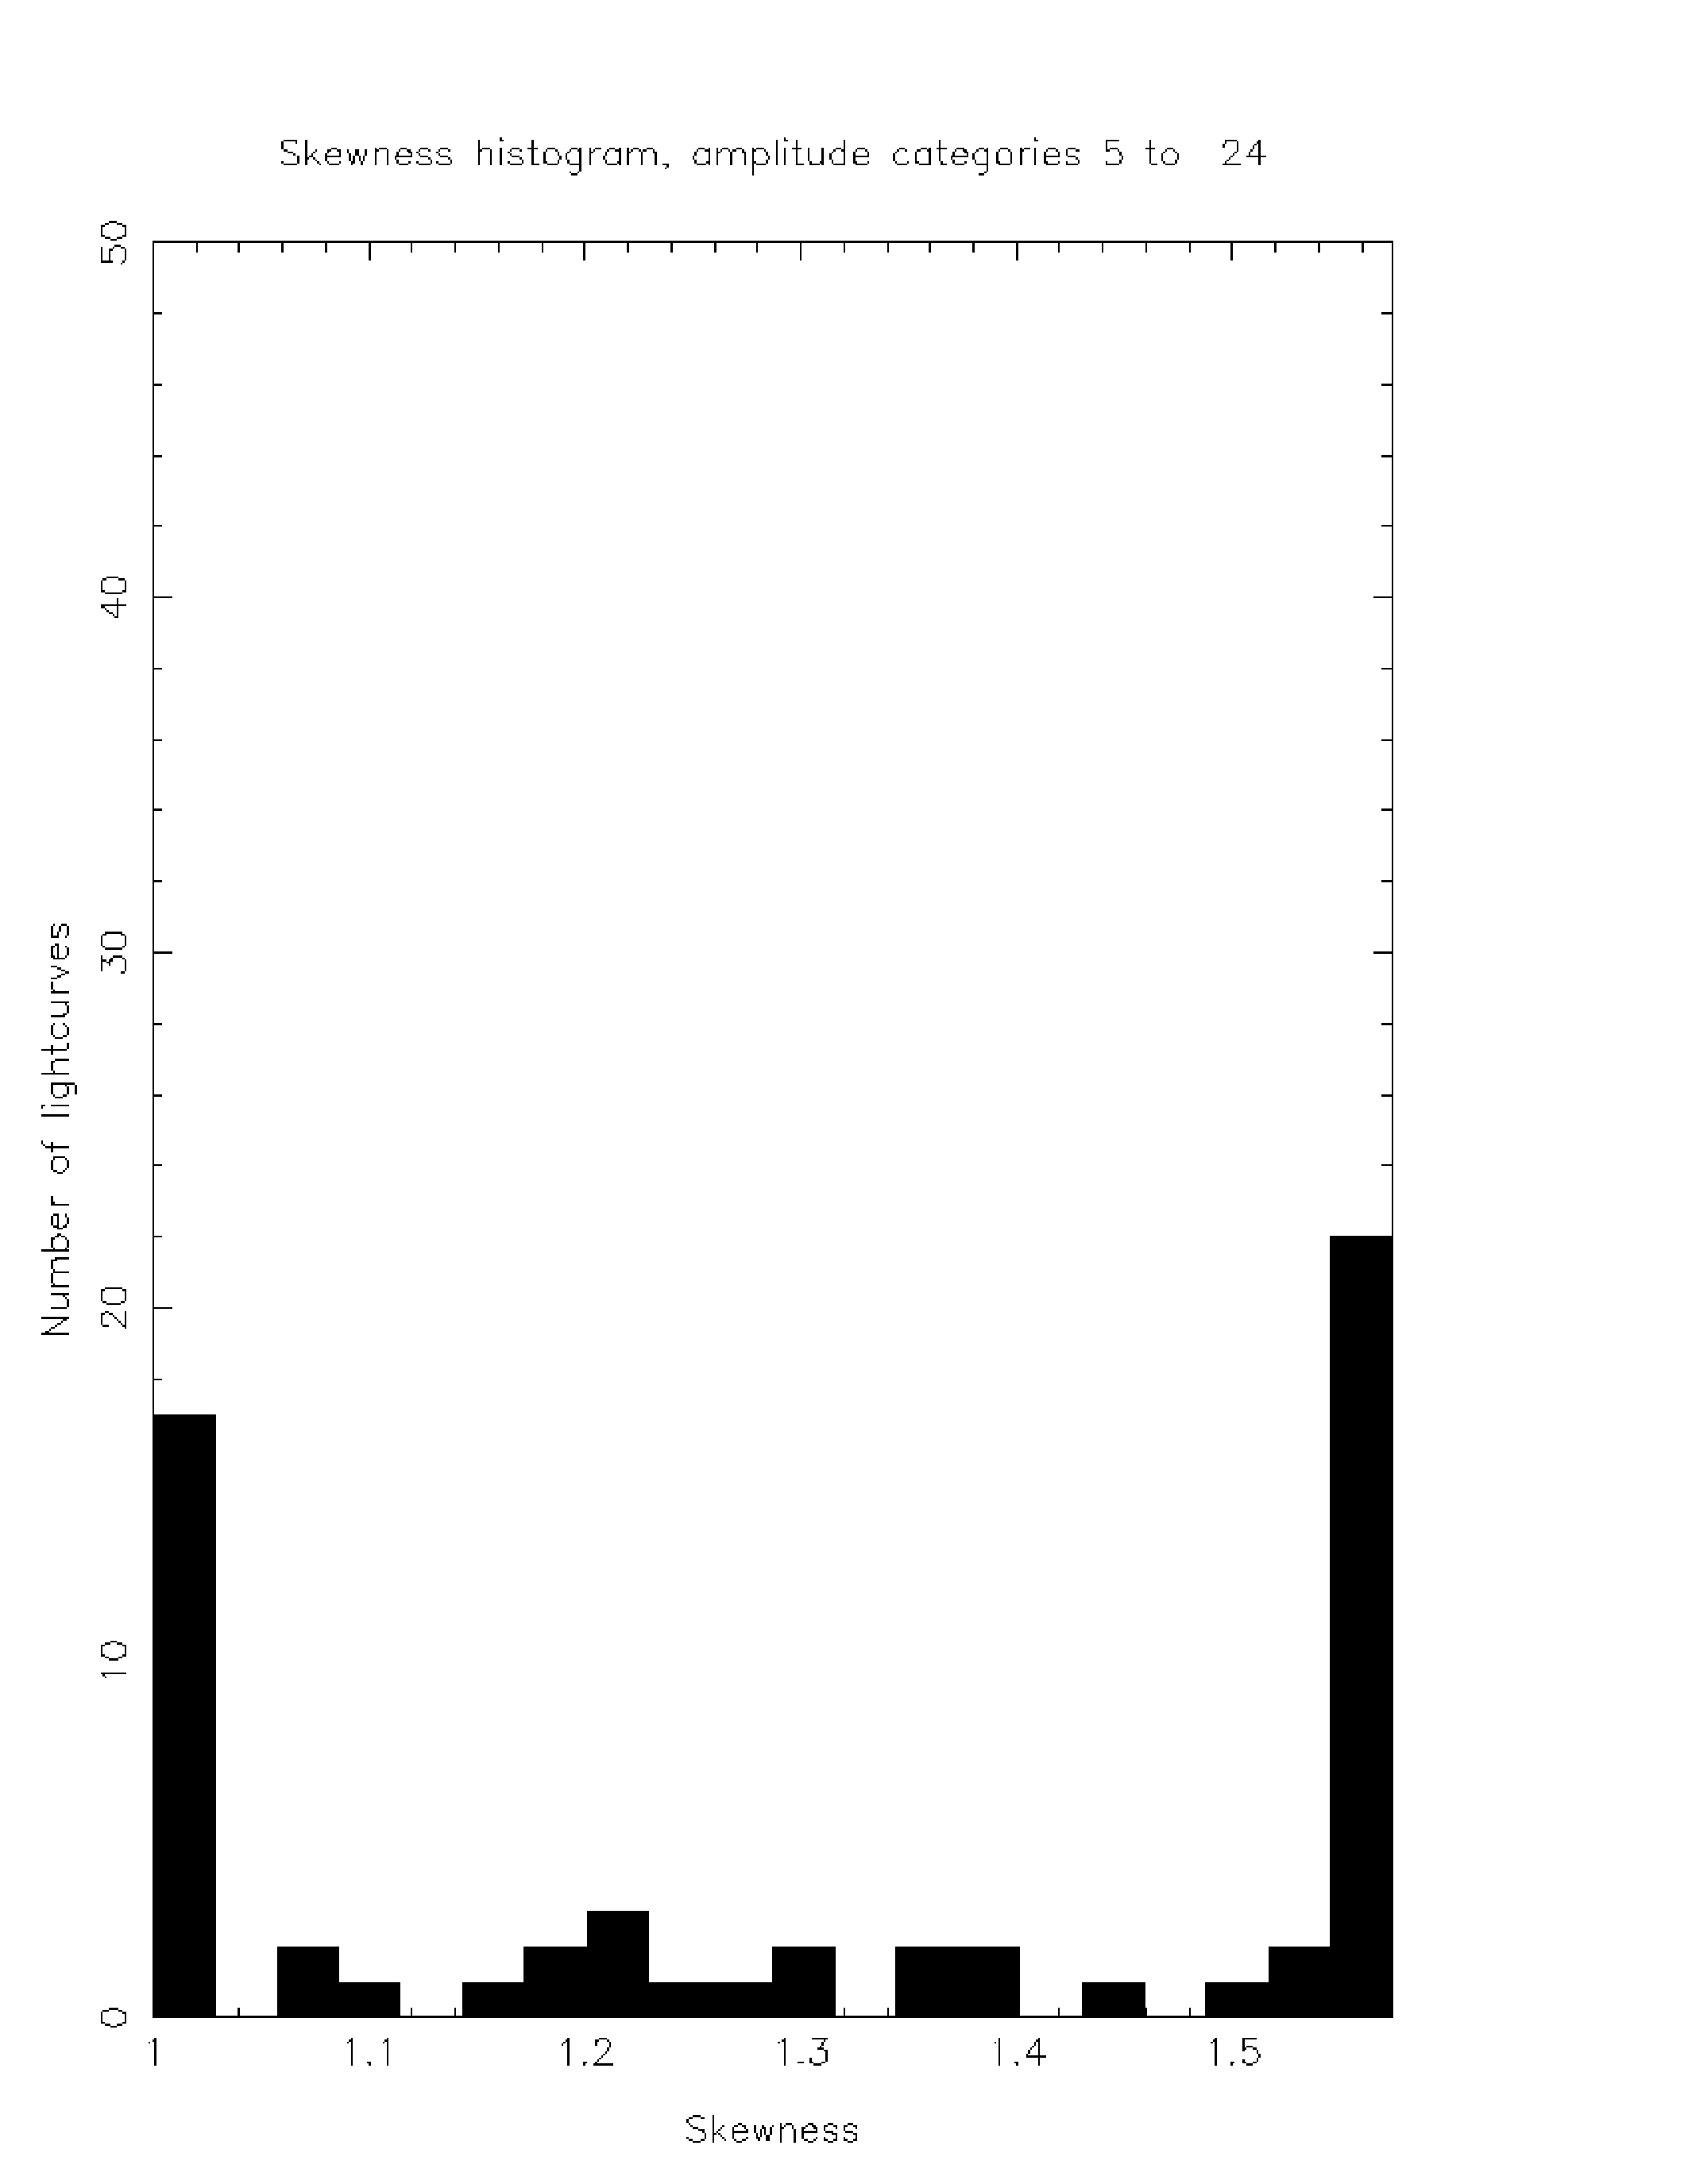} \\
\vspace*{0cm}
   \leavevmode
 \includegraphics{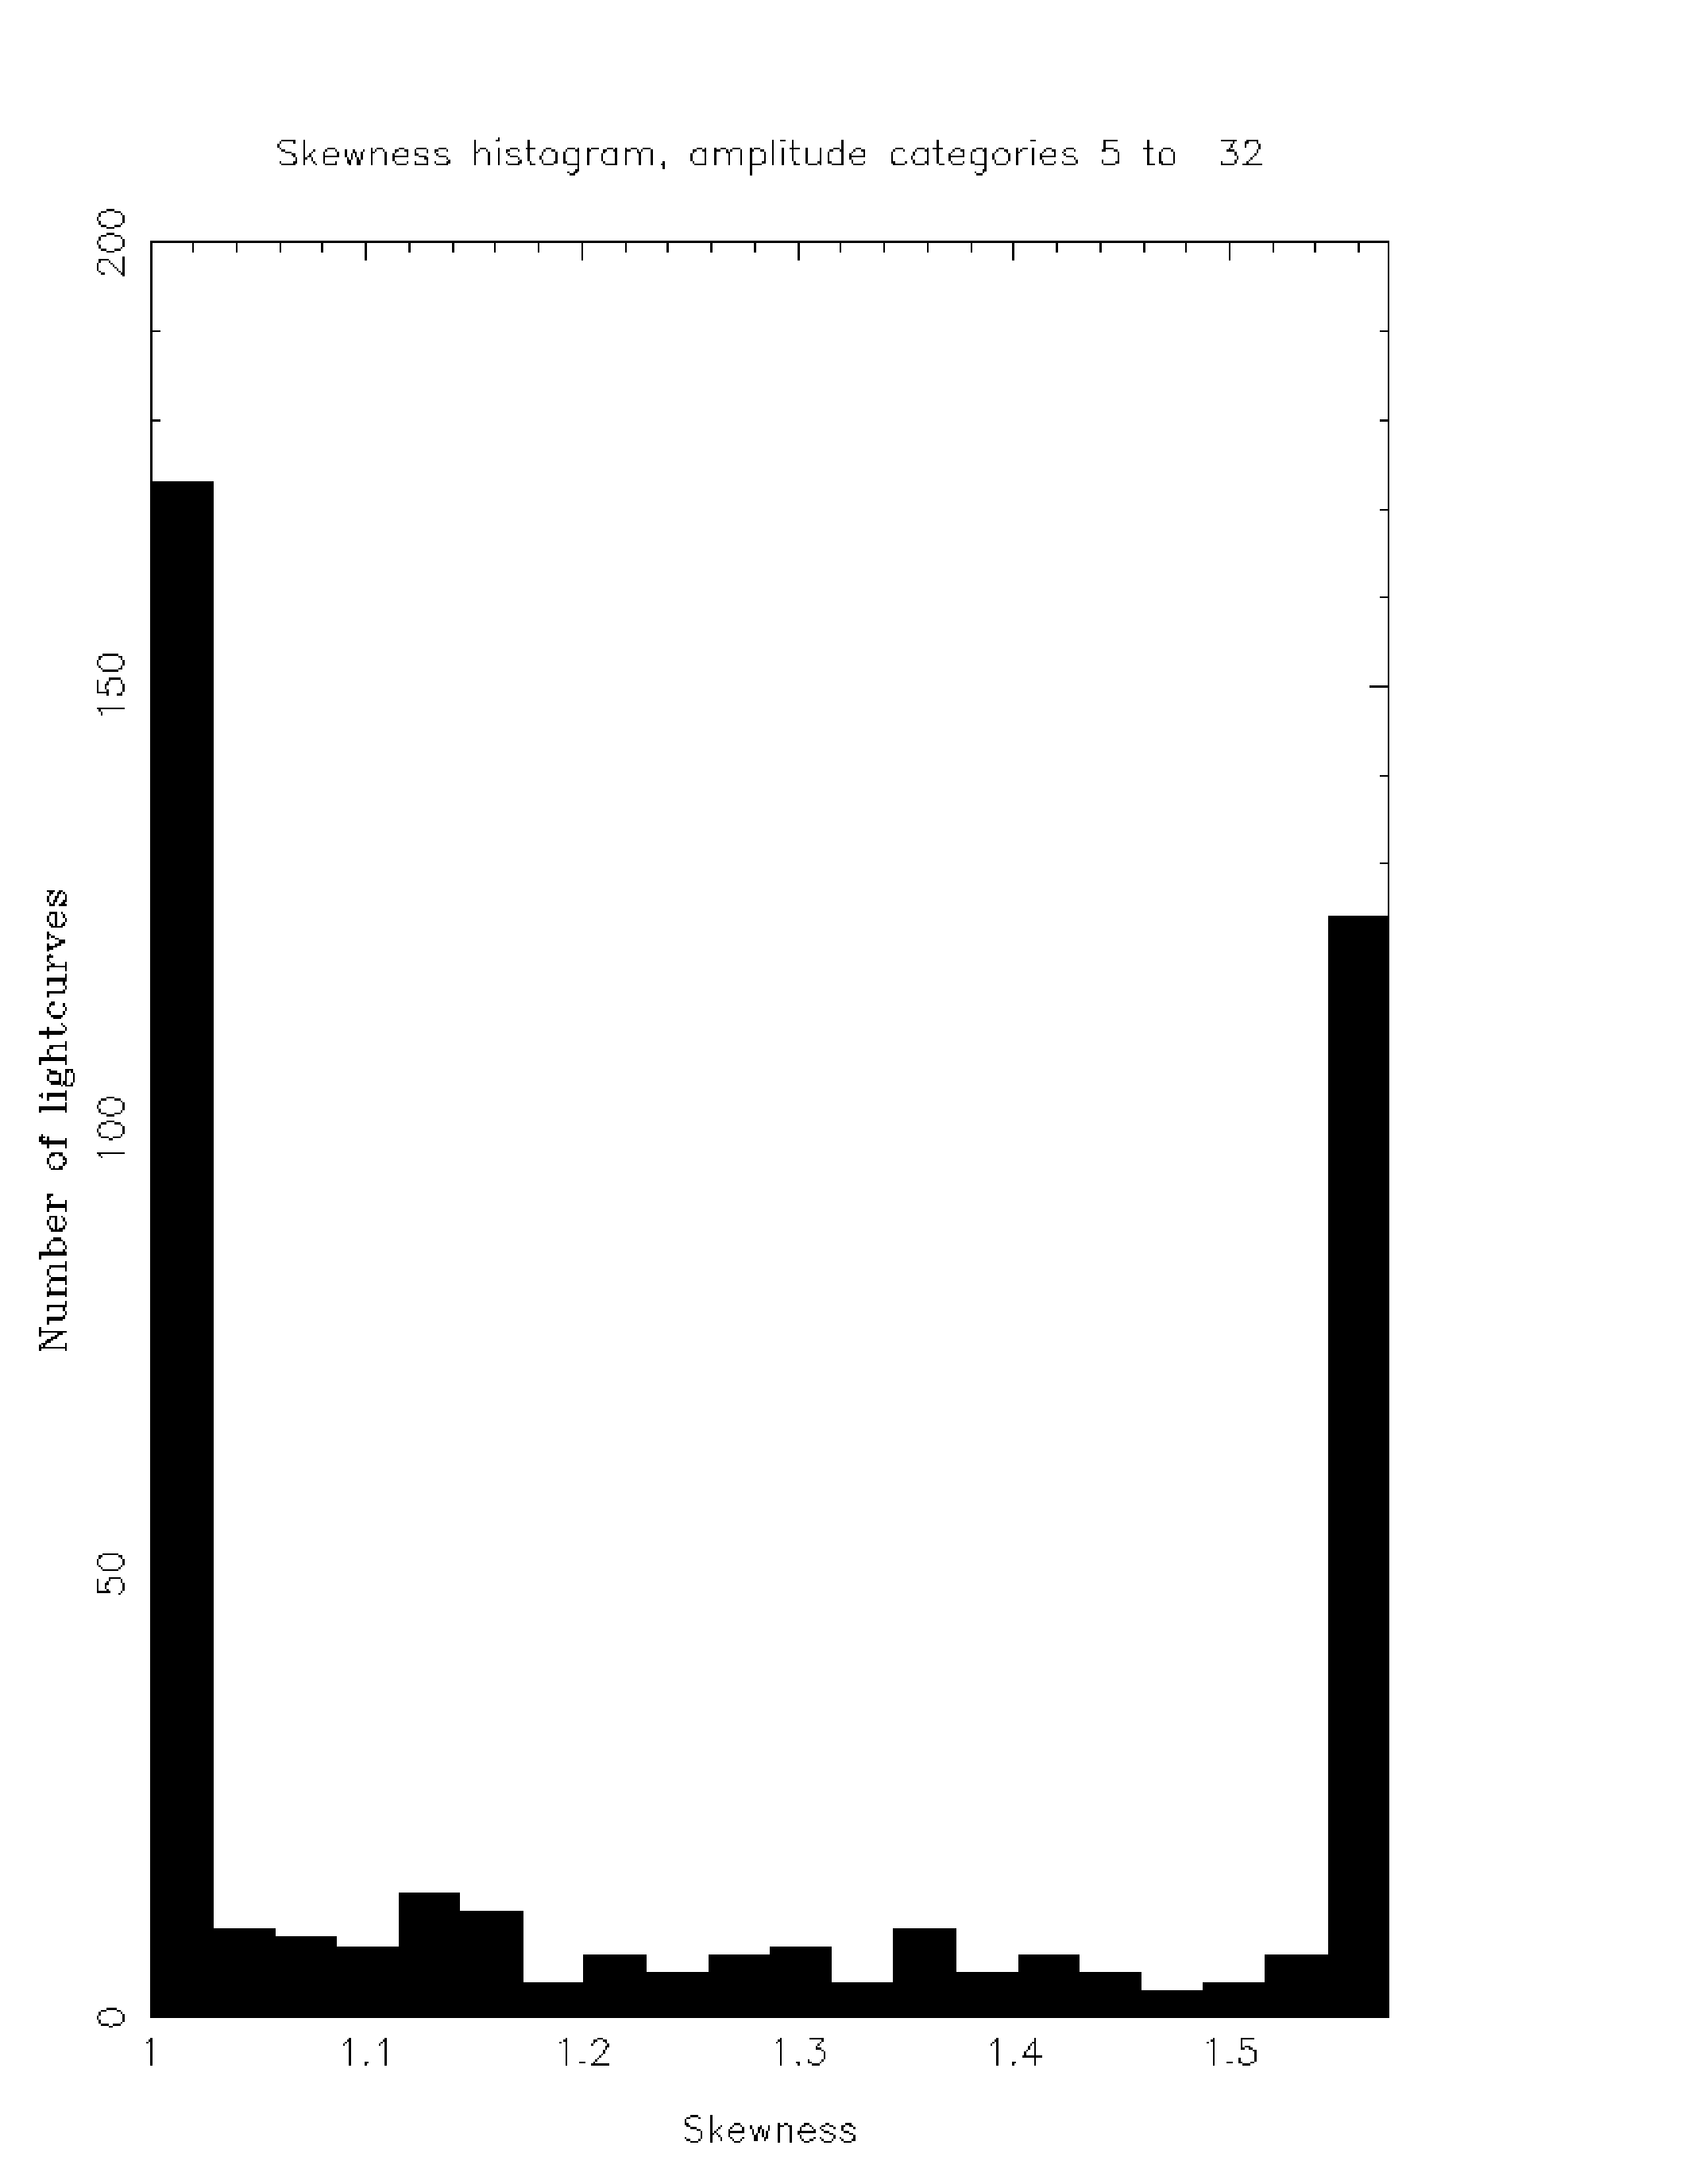} \\
  \end{tabular}
\hspace*{4cm}
  \begin{tabular}{ccc}
%% ALL amp categories.
\vspace*{5cm}
   \leavevmode
 \includegraphics{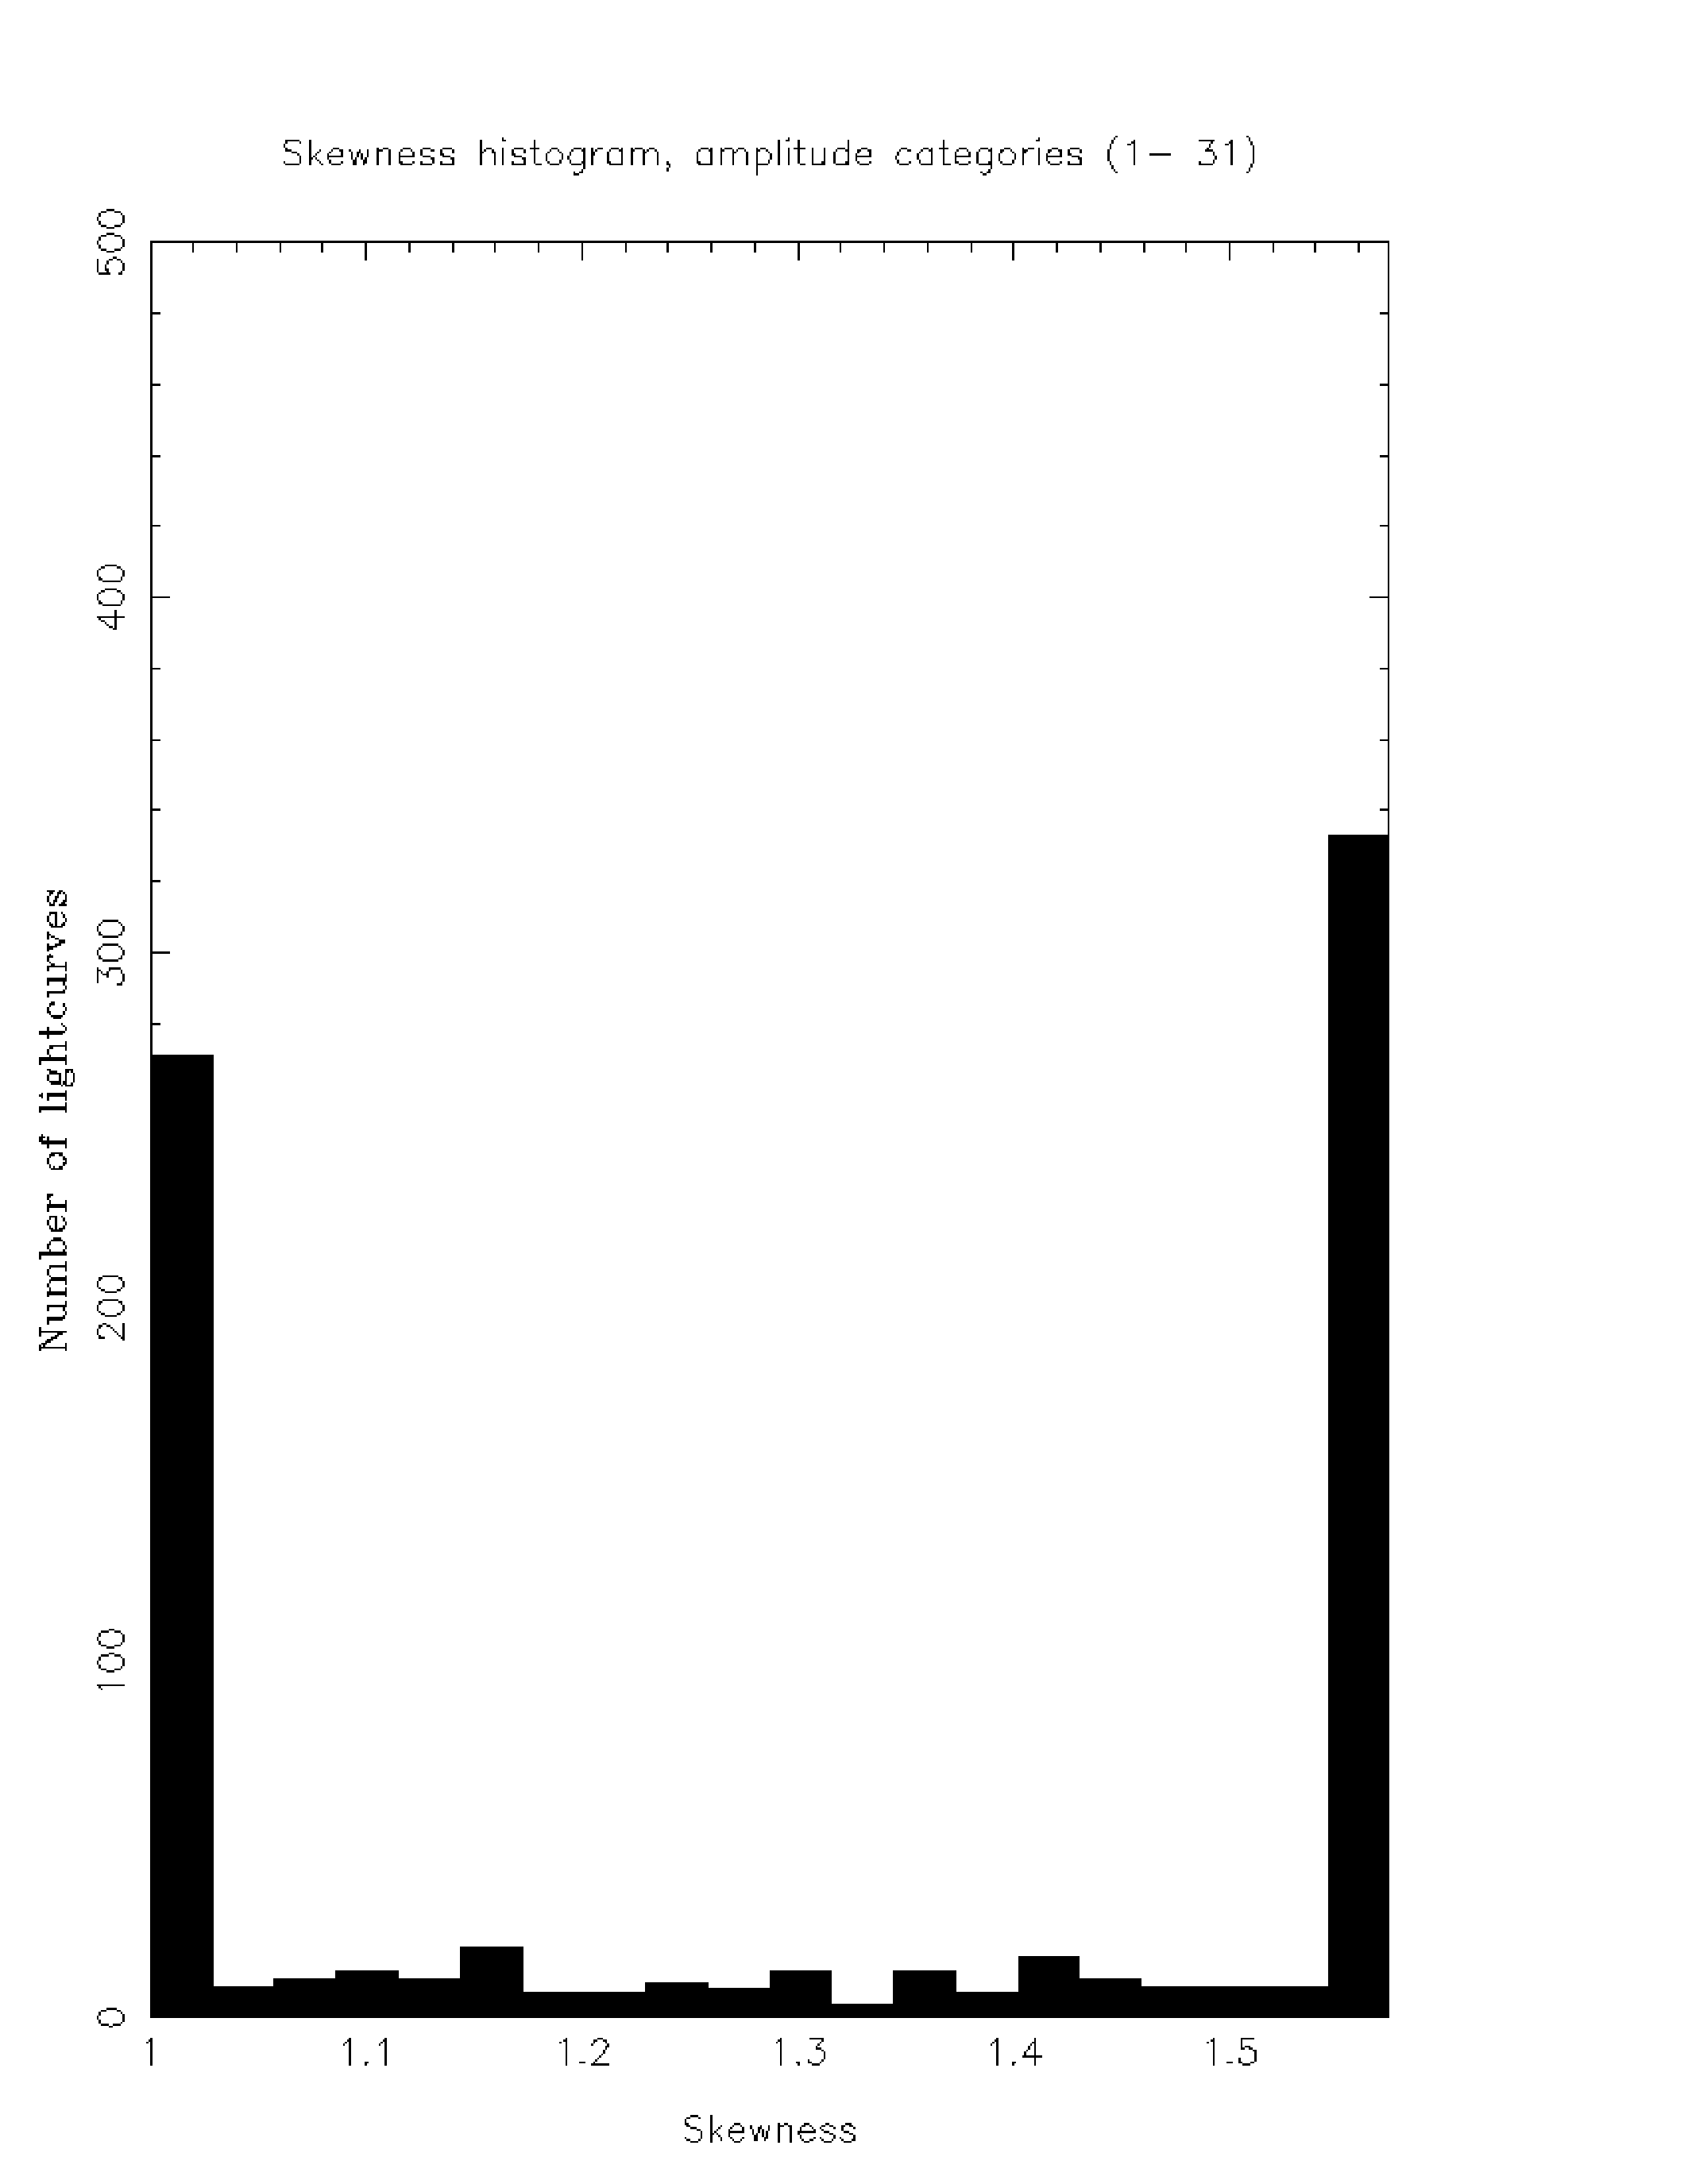} \\
\vspace*{5cm}
   \leavevmode
 \includegraphics{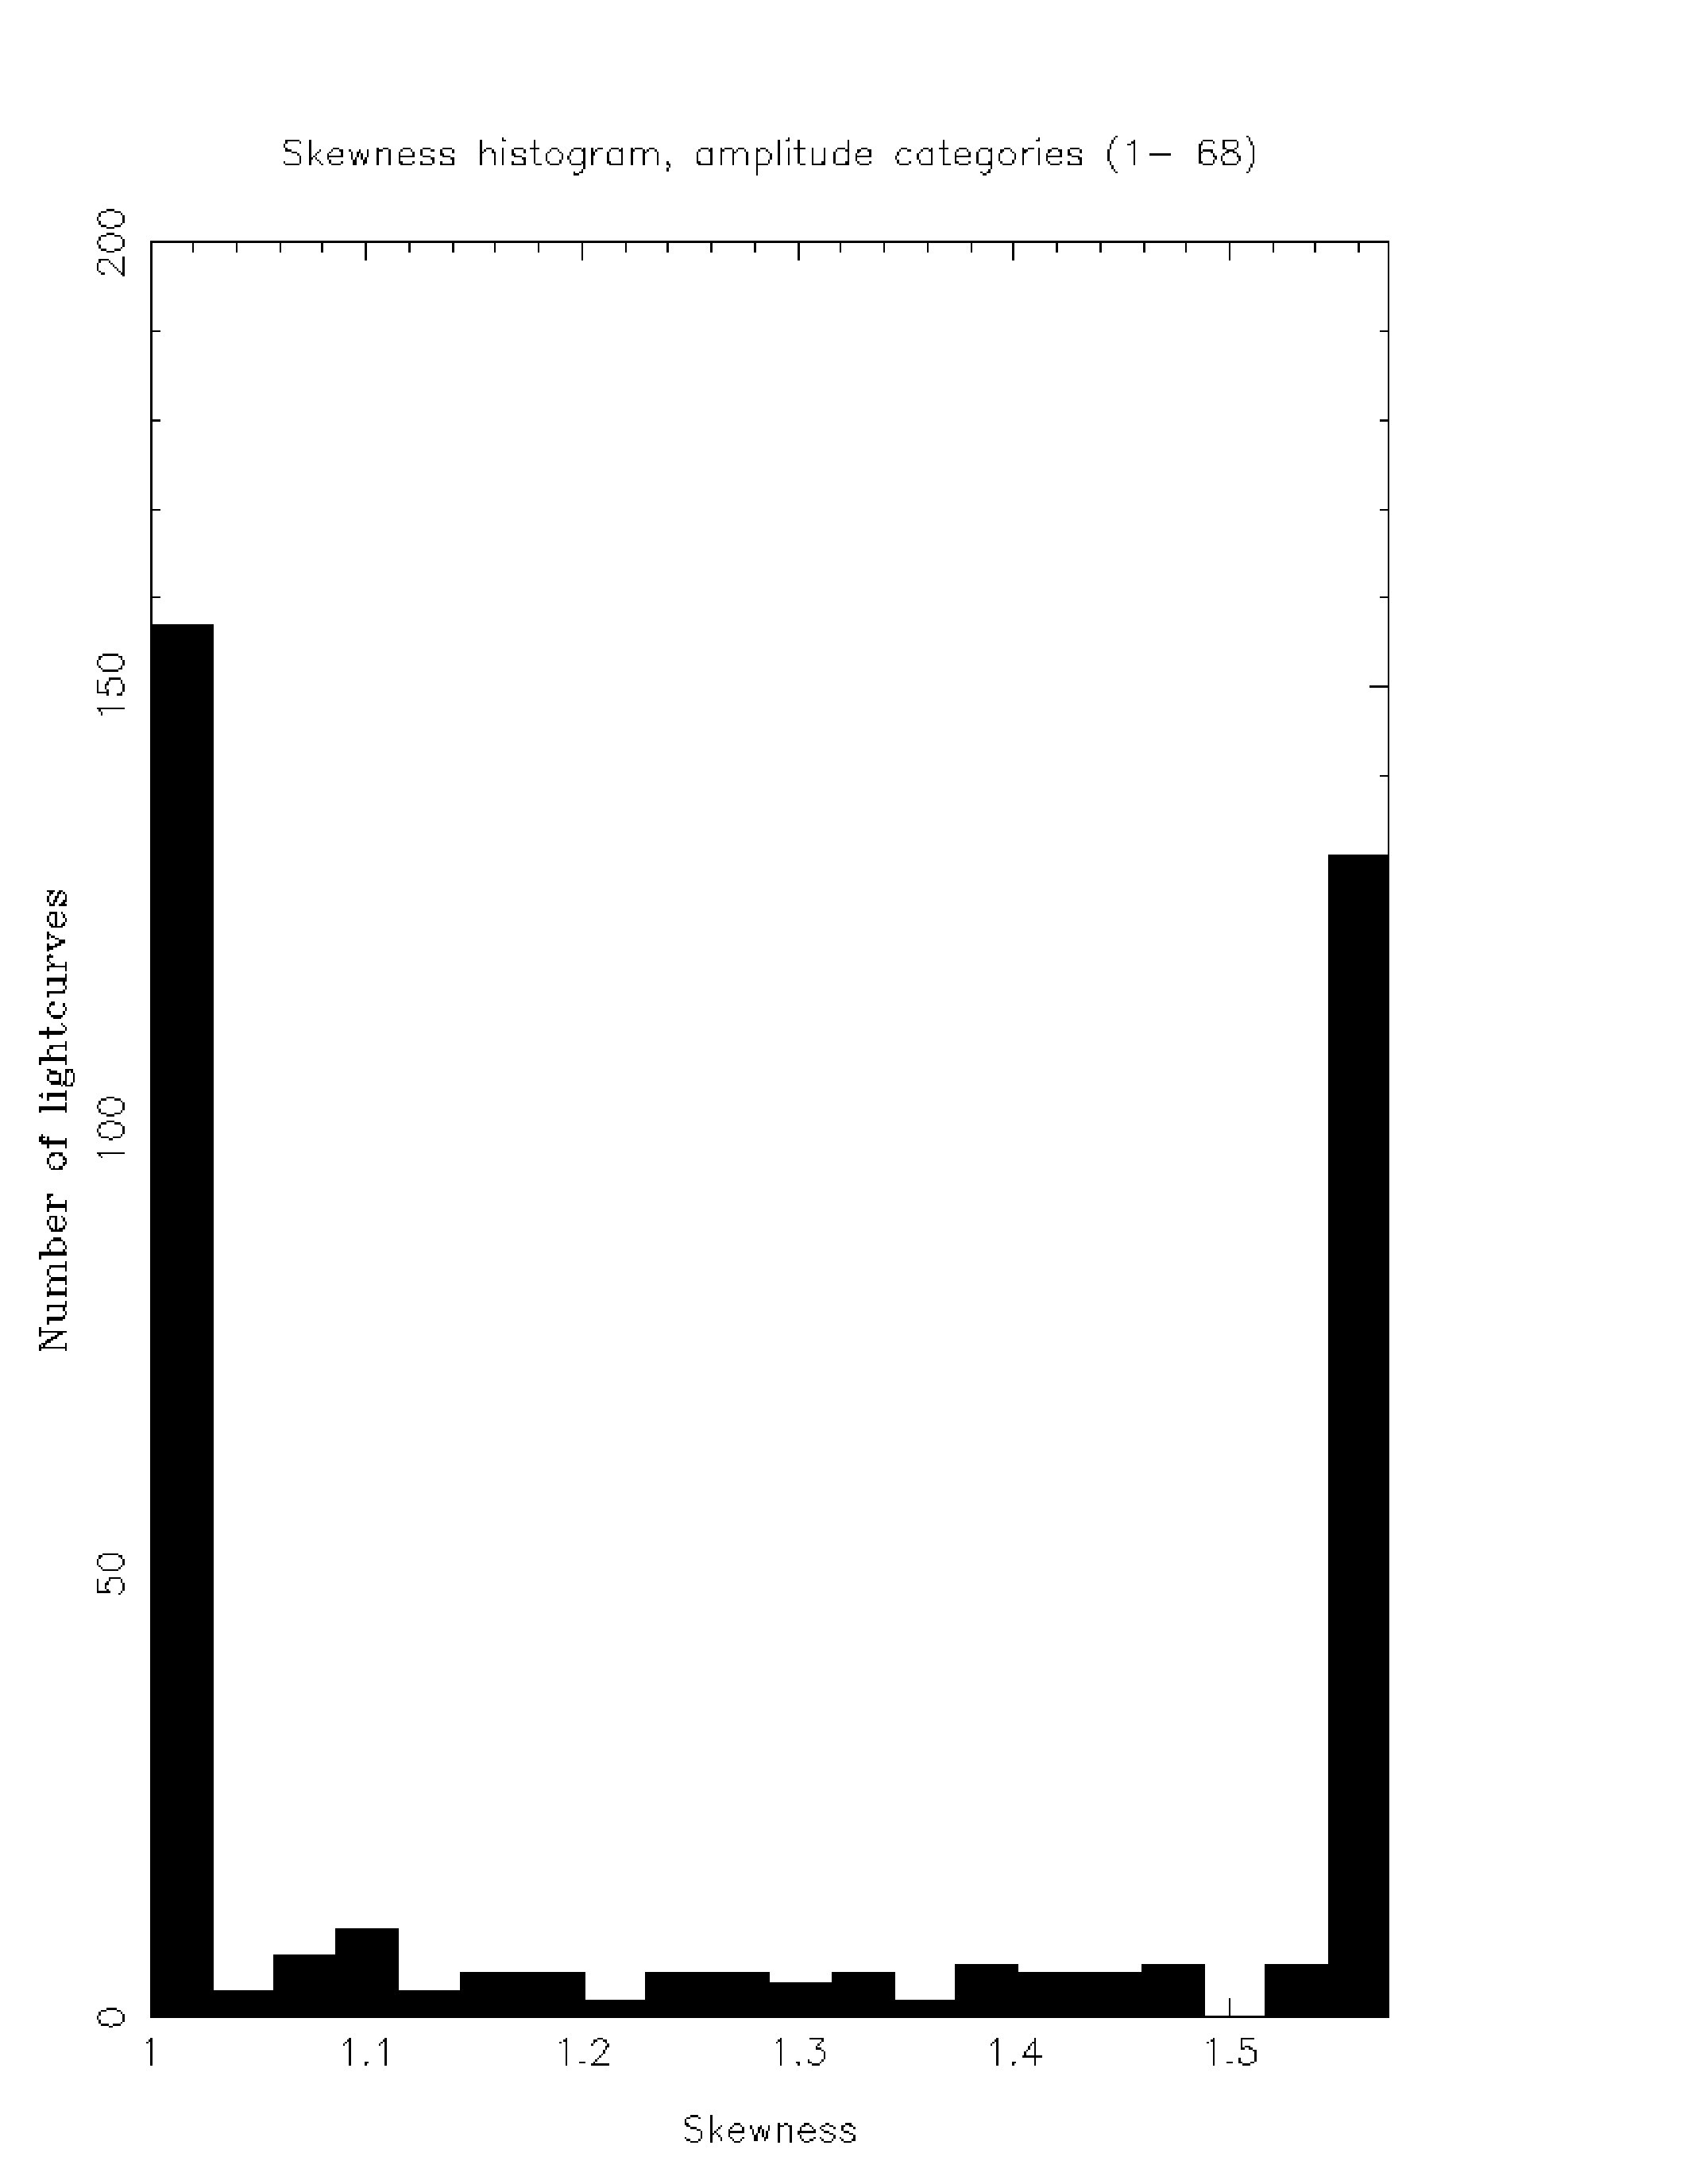} \\
\vspace*{5cm}
   \leavevmode
 \includegraphics{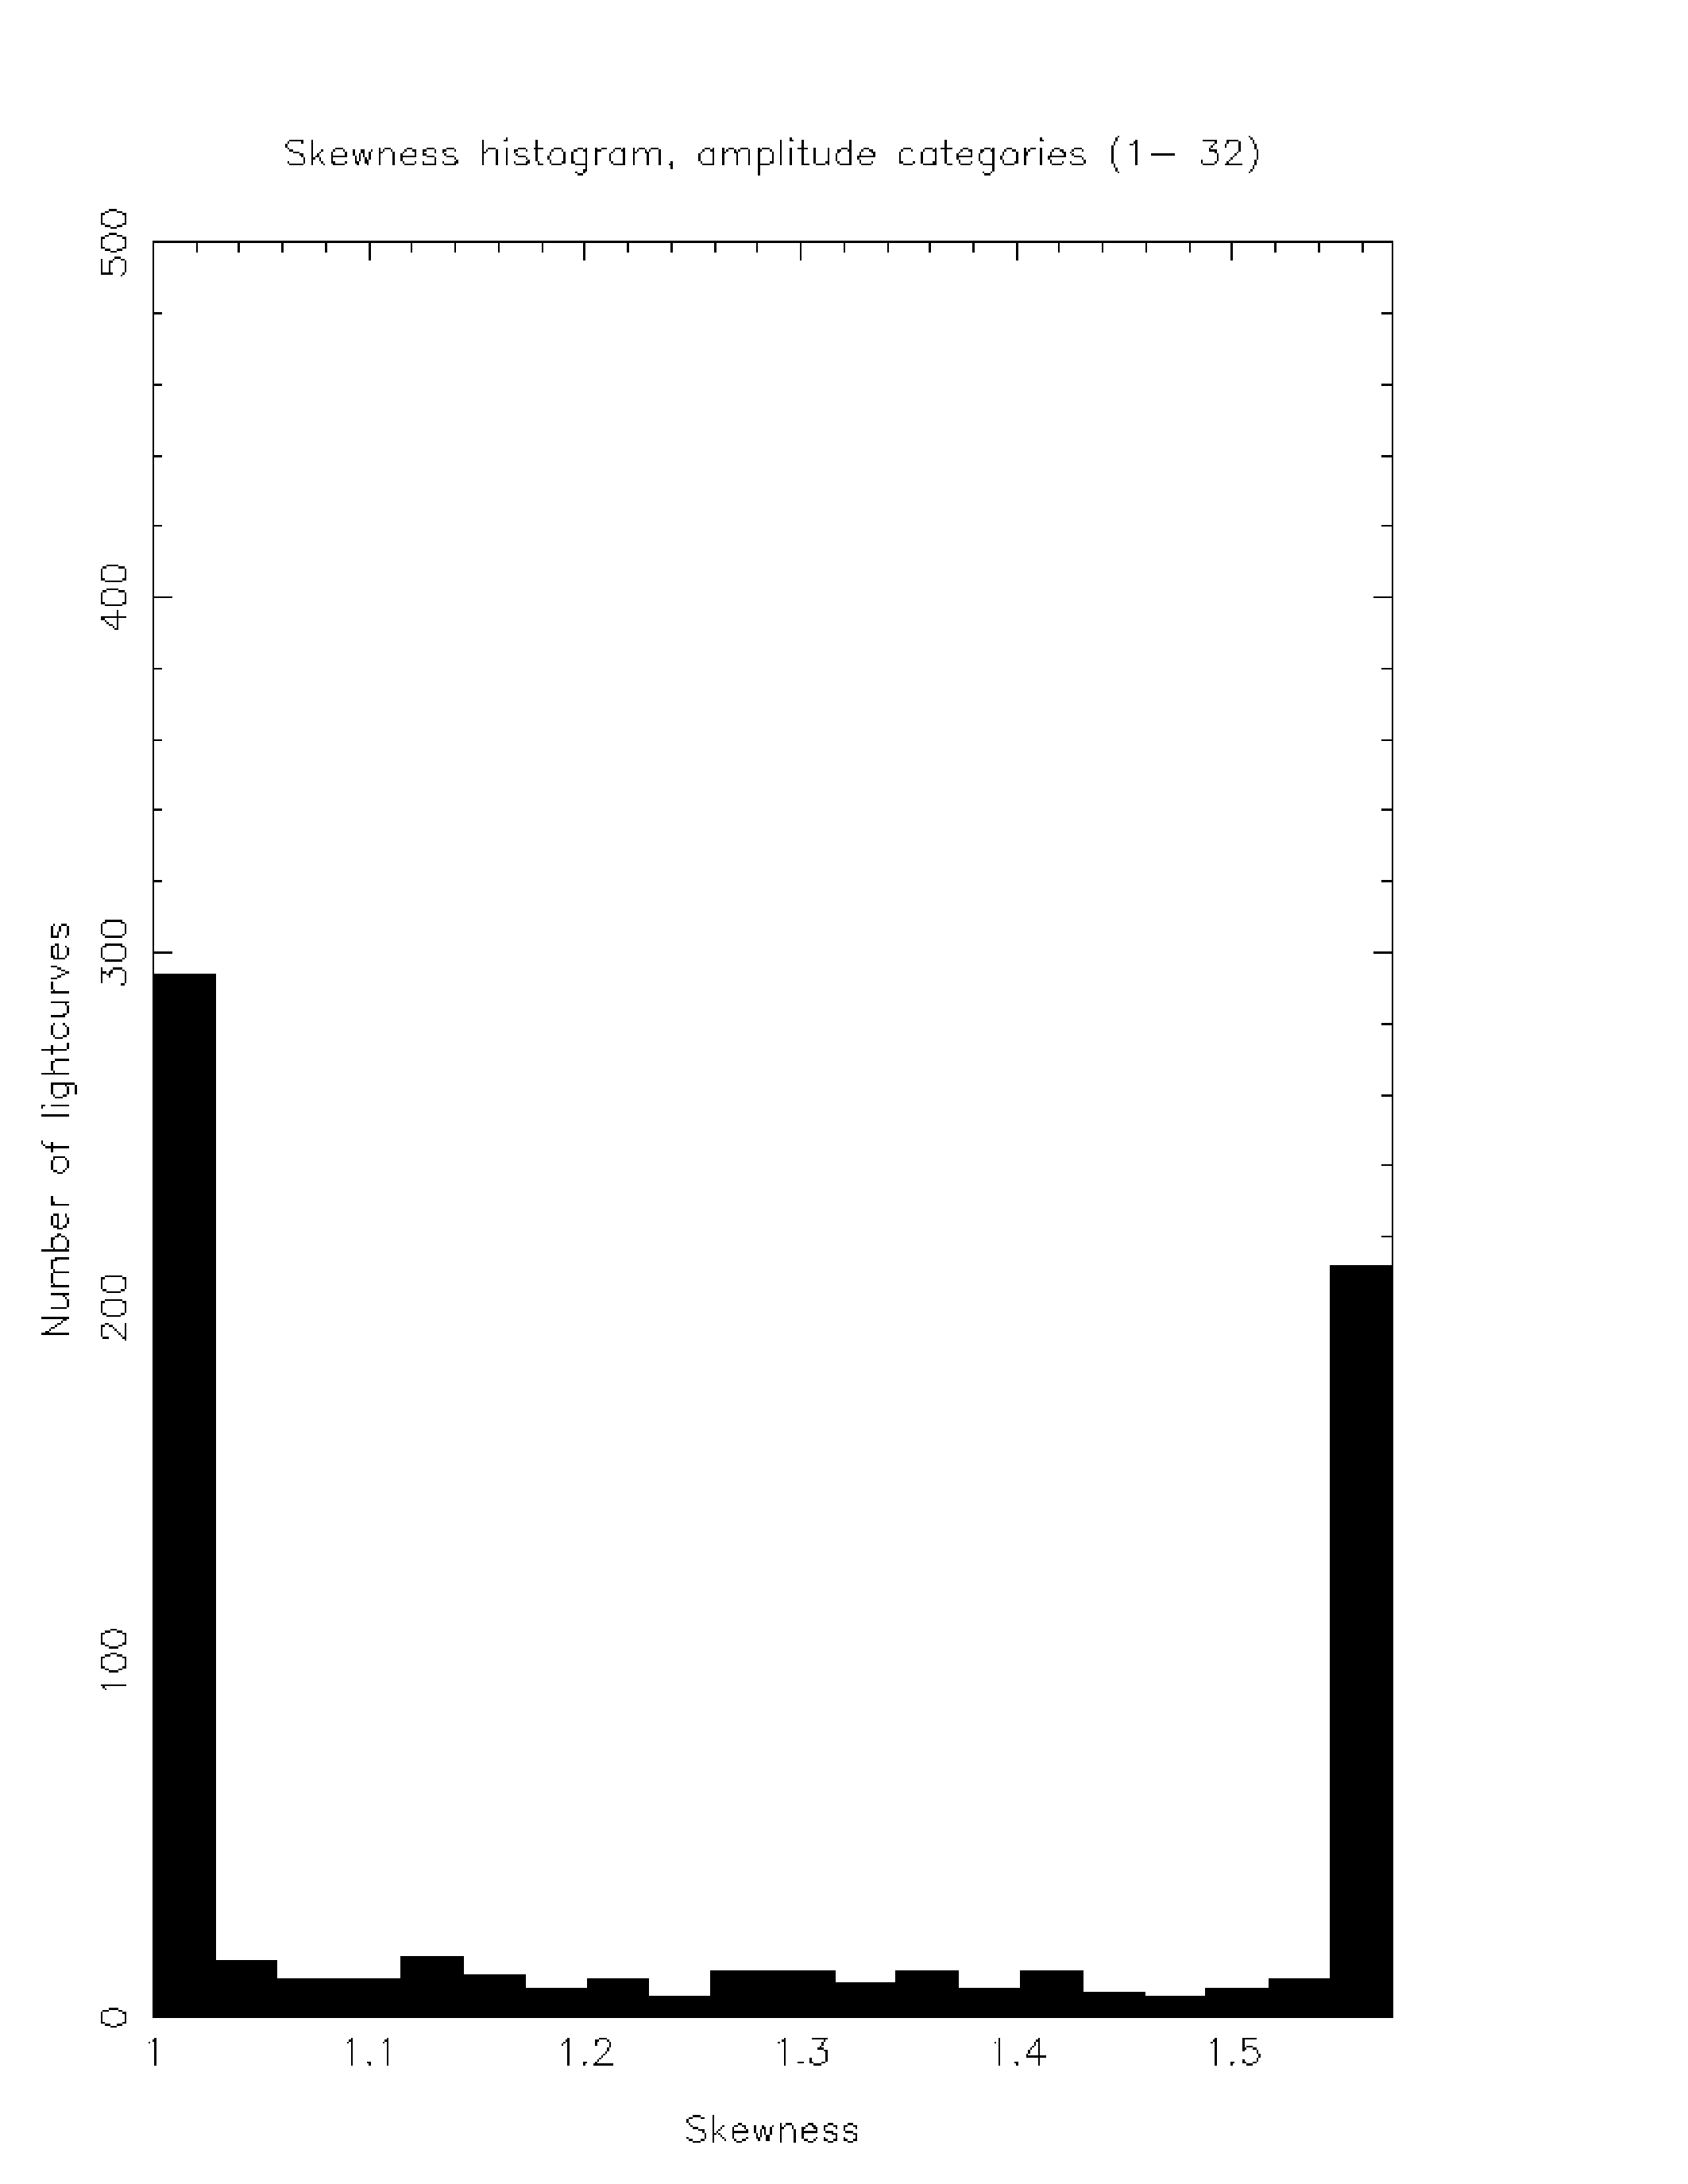} \\
\vspace*{0cm}
   \leavevmode
 \includegraphics{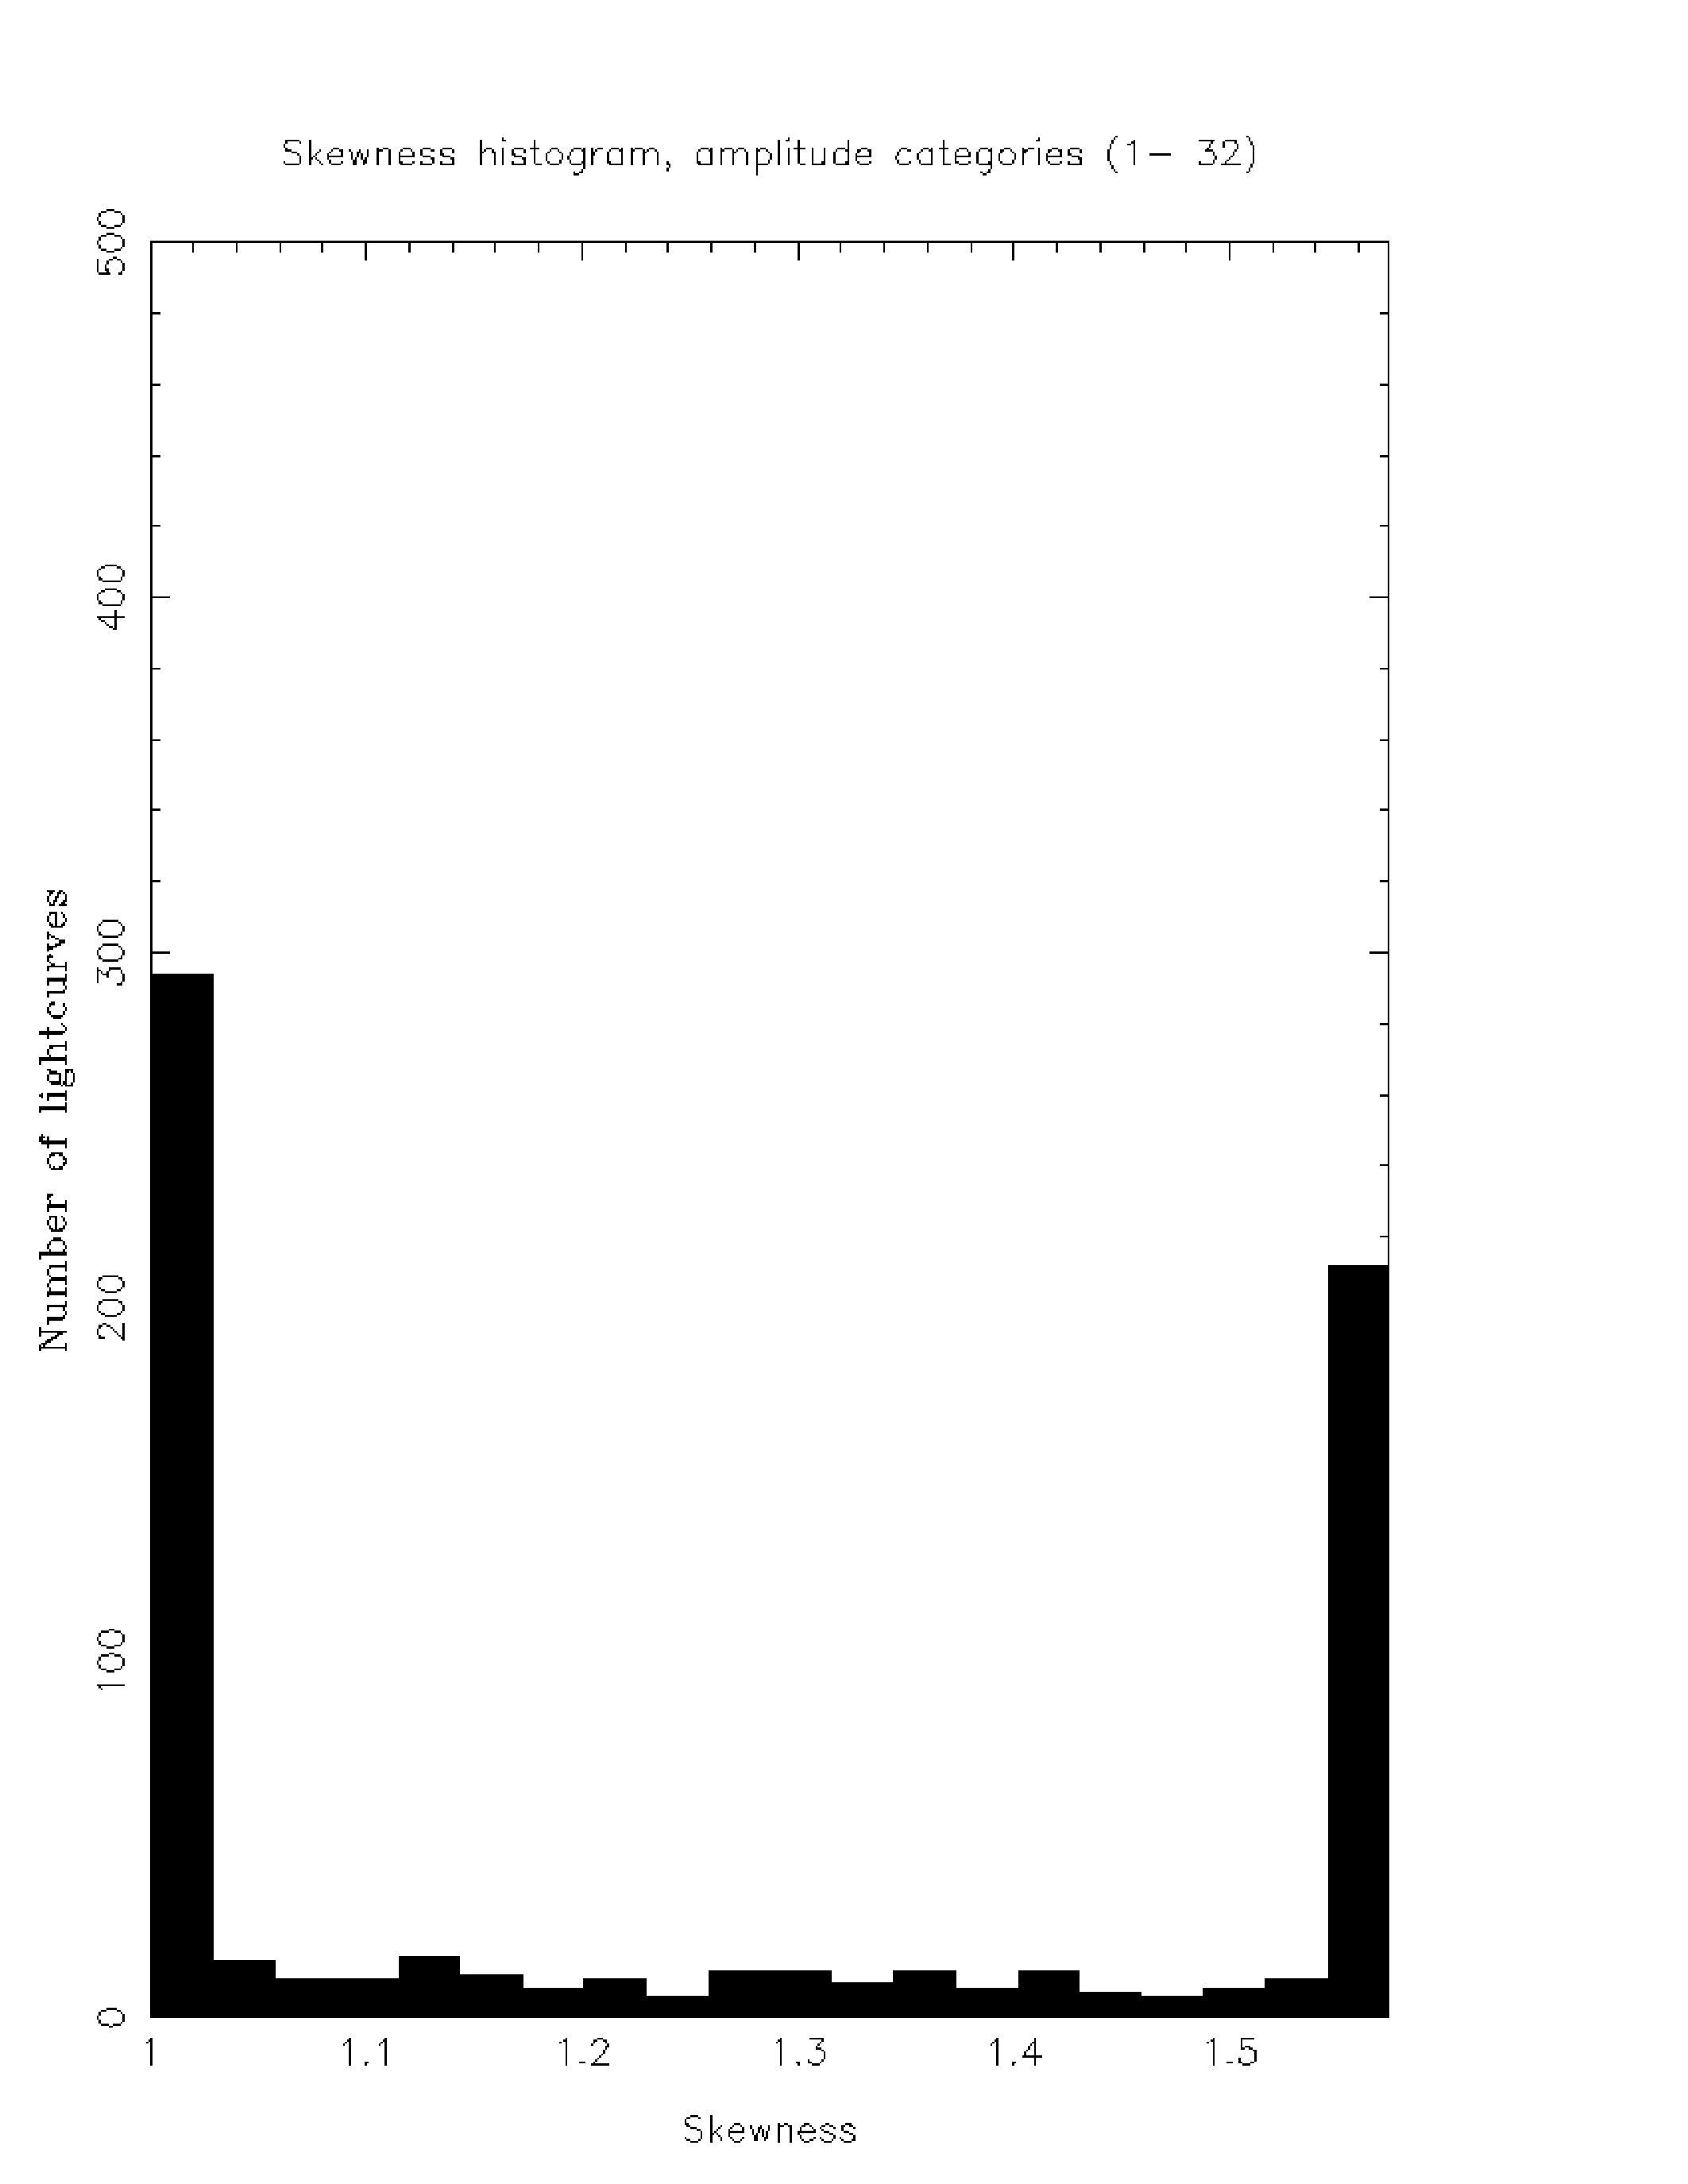} \\
  \end{tabular}
 %}
}
\caption[Histograms of variable lightcurve Skewness distributions: PA/LT flux ratio = 7.89. ]{Histograms of variable
 lightcurve Skewness distributions: PA/LT flux ratio = 7.89; Rows, top to bottom:
1)`variable' lightcurves containing (LT) or (LT + FTN) data only,
2) ``mixed'' lightcurves containing (LT) or (LT + FTN) data only,
3)`variable' lightcurves containing (PA + LT) or (PA + LT + FTN) data,
4) ``mixed'' lightcurves containing (PA + LT) or (PA + LT + FTN) data.
Columns, left to right: Flux amplitudes, 1) 0-5, 2) 5-`MAX' 3) Sum of all categories
`MAX' varies with row as: 1) 31 2) 68 3) 24 4) 32 .}
 \label{Skewness_all_categories_low_ratio}
\end{figure}

% MED RATIO

\newpage

\begin{figure}
\vspace*{4cm}
\center{
  \begin{tabular}{ccc}
% 0-5
\vspace*{5cm}
   \leavevmode
 \includegraphics{/data/thesis/thesis_document/chapter5/figures/variable_plots/med_ratio/LT/var/All_chimax_15._SNcategory_0_to_5_14_05_08_LT_chisq_log_P_histogram_030.eps} \\
\vspace*{5cm}
   \leavevmode
 \includegraphics{/data/thesis/thesis_document/chapter5/figures/variable_plots/med_ratio/LT/mixed/All_chimax_15._SNcategory_0_to_5_14_05_08_LT_mixed_chisq_log_P_histogram_030.eps} \\
\vspace*{5cm}
   \leavevmode
 \includegraphics{/data/thesis/thesis_document/chapter5/figures/variable_plots/med_ratio/PA/var/All_chimax_15._SNcategory_0_to_5_14_05_08_chisq_log_P_histogram_030.eps} \\
\vspace*{0cm}
   \leavevmode
 \includegraphics{/data/thesis/thesis_document/chapter5/figures/variable_plots/med_ratio/PA/mixed/All_chimax_15._SNcategory_0_to_5_14_05_08_mixed_chisq_log_P_histogram_030.eps} \\
  \end{tabular}
 %}
\hspace*{4cm}
  \begin{tabular}{ccc}
% 5 - whatever
\vspace*{5cm}
   \leavevmode
 \includegraphics{/data/thesis/thesis_document/chapter5/figures/variable_plots/med_ratio/LT/var/All_chimax_15._SNcategory_5_to_031_14_05_08_LT_chisq_log_P_histogram_030.eps} \\
 \vspace*{5cm}
   \leavevmode
\includegraphics{/data/thesis/thesis_document/chapter5/figures/variable_plots/med_ratio/LT/mixed/All_chimax_15._SNcategory_5_to_068_14_05_08_LT_mixed_chisq_log_P_histogram_030.eps} \\
\vspace*{5cm}
   \leavevmode
 \includegraphics{/data/thesis/thesis_document/chapter5/figures/variable_plots/med_ratio/PA/var/All_chimax_15._SNcategory_5_to_018_14_05_08_chisq_log_P_histogram_030.eps} \\
\vspace*{0cm}
   \leavevmode
 \includegraphics{/data/thesis/thesis_document/chapter5/figures/variable_plots/med_ratio/PA/mixed/All_chimax_15._SNcategory_5_to_022_14_05_08_mixed_chisq_log_P_histogram_030.eps} \\
  \end{tabular}
\hspace*{4cm}
  \begin{tabular}{ccc}
%% ALL amp categories.
\vspace*{5cm}
   \leavevmode
 \includegraphics{/data/thesis/thesis_document/chapter5/figures/variable_plots/med_ratio/LT/var/All_chimax_15._SNcategory_ALL_14_05_08_LT_chisq_log_P_histogram_030.eps} \\
\vspace*{5cm}
   \leavevmode
 \includegraphics{/data/thesis/thesis_document/chapter5/figures/variable_plots/med_ratio/LT/mixed/All_chimax_15._SNcategory_ALL_14_05_08_LT_mixed_chisq_log_P_histogram_030.eps} \\
\vspace*{5cm}
   \leavevmode
 \includegraphics{/data/thesis/thesis_document/chapter5/figures/variable_plots/med_ratio/PA/var/All_chimax_15._SNcategory_ALL_14_05_08_chisq_log_P_histogram_030.eps} \\
\vspace*{0cm}
   \leavevmode
 \includegraphics{/data/thesis/thesis_document/chapter5/figures/variable_plots/med_ratio/PA/mixed/All_chimax_15._SNcategory_ALL_14_05_08_mixed_chisq_log_P_histogram_030.eps} \\
  \end{tabular}
 %}
}
\caption[Histograms of variable lightcurve log(P) distributions: PA/LT flux ratio = 11.10 .]{Histograms of variable
 lightcurve log(P) distributions: PA/LT flux ratio = 11.10 ; Rows, top to bottom:
1)`variable' lightcurves containing (LT) or (LT + FTN) data only,
2) ``mixed'' lightcurves containing (LT) or (LT + FTN) data only,
3)`variable' lightcurves containing (PA + LT) or (PA + LT + FTN) data,
4) ``mixed'' lightcurves containing (PA + LT) or (PA + LT + FTN) data.
Columns, left to right: Flux amplitudes, 1) 0-5, 2) 5-`MAX' 3) Sum of all categories
`MAX' varies with row as: 1) 31 2) 68 3) 18 4) 22 .}
 \label{log(P)_all_categories_med_ratio}
\end{figure}

\newpage

\begin{figure}
\vspace*{4cm}
\center{
  \begin{tabular}{ccc}
% 0-5
\vspace*{5cm}
   \leavevmode
 \includegraphics{/data/thesis/thesis_document/chapter5/figures/variable_plots/med_ratio/LT/var/All_chimax_15._SNcategory_0_to_5_14_05_08_LT_chisq_skew_histogram_020.eps} \\
\vspace*{5cm}
   \leavevmode
 \includegraphics{/data/thesis/thesis_document/chapter5/figures/variable_plots/med_ratio/LT/mixed/All_chimax_15._SNcategory_0_to_5_14_05_08_LT_mixed_chisq_skew_histogram_020.eps} \\
\vspace*{5cm}
   \leavevmode
 \includegraphics{/data/thesis/thesis_document/chapter5/figures/variable_plots/med_ratio/PA/var/All_chimax_15._SNcategory_0_to_5_14_05_08_chisq_skew_histogram_020.eps} \\
\vspace*{0cm}
   \leavevmode
 \includegraphics{/data/thesis/thesis_document/chapter5/figures/variable_plots/med_ratio/PA/mixed/All_chimax_15._SNcategory_0_to_5_14_05_08_mixed_chisq_skew_histogram_020.eps} \\
  \end{tabular}
 %}
\hspace*{4cm}
  \begin{tabular}{ccc}
% 5 - whatever
\vspace*{5cm}
   \leavevmode
 \includegraphics{/data/thesis/thesis_document/chapter5/figures/variable_plots/med_ratio/LT/var/All_chimax_15._SNcategory_5_to_031_14_05_08_LT_chisq_skew_histogram_020.eps} \\
 \vspace*{5cm}
   \leavevmode
\includegraphics{/data/thesis/thesis_document/chapter5/figures/variable_plots/med_ratio/LT/mixed/All_chimax_15._SNcategory_5_to_068_14_05_08_LT_mixed_chisq_skew_histogram_020.eps} \\
\vspace*{5cm}
   \leavevmode
 \includegraphics{/data/thesis/thesis_document/chapter5/figures/variable_plots/med_ratio/PA/var/All_chimax_15._SNcategory_5_to_018_14_05_08_chisq_skew_histogram_020.eps} \\
\vspace*{0cm}
   \leavevmode
 \includegraphics{/data/thesis/thesis_document/chapter5/figures/variable_plots/med_ratio/PA/mixed/All_chimax_15._SNcategory_5_to_022_14_05_08_mixed_chisq_skew_histogram_020.eps} \\
  \end{tabular}
\hspace*{4cm}
  \begin{tabular}{ccc}
%% ALL amp categories.
\vspace*{5cm}
   \leavevmode
 \includegraphics{/data/thesis/thesis_document/chapter5/figures/variable_plots/med_ratio/LT/var/All_chimax_15._SNcategory_ALL_14_05_08_LT_chisq_skew_histogram_020.eps} \\
\vspace*{5cm}
   \leavevmode
 \includegraphics{/data/thesis/thesis_document/chapter5/figures/variable_plots/med_ratio/LT/mixed/All_chimax_15._SNcategory_ALL_14_05_08_LT_mixed_chisq_skew_histogram_020.eps} \\
\vspace*{5cm}
   \leavevmode
 \includegraphics{/data/thesis/thesis_document/chapter5/figures/variable_plots/med_ratio/PA/var/All_chimax_15._SNcategory_ALL_14_05_08_chisq_skew_histogram_020.eps} \\
\vspace*{0cm}
   \leavevmode
 \includegraphics{/data/thesis/thesis_document/chapter5/figures/variable_plots/med_ratio/PA/mixed/All_chimax_15._SNcategory_ALL_14_05_08_mixed_chisq_skew_histogram_020.eps} \\
  \end{tabular}
}
\caption[Histograms of variable lightcurve Skewness distributions: PA/LT flux ratio = 11.10 .]{Histograms of variable
 lightcurve Skewness distributions: PA/LT flux ratio = 11.10 ; Rows, top to bottom:
1)`variable' lightcurves containing (LT) or (LT + FTN) data only,
2) ``mixed'' lightcurves containing (LT) or (LT + FTN) data only,
3)`variable' lightcurves containing (PA + LT) or (PA + LT + FTN) data,
4) ``mixed'' lightcurves containing (PA + LT) or (PA + LT + FTN) data.
Columns, left to right: Flux amplitudes, 1) 0-5, 2) 5-`MAX' 3) Sum of all categories
`MAX' varies with row as: 1) 31 2) 68 3) 18 4) 22 .}
 \label{Skewness_all_categories_med_ratio}
\end{figure} 

% HIGH RATIO
\newpage

\begin{figure}
\vspace*{4cm}
\center{
  \begin{tabular}{ccc}
% 0-5
\vspace*{5cm}
   \leavevmode
 \includegraphics{/data/thesis/thesis_document/chapter5/figures/variable_plots/high_ratio/LT/var/All_chimax_15._SNcategory_0_to_5_20_05_08_LT_chisq_log_P_histogram_030.eps} \\
\vspace*{5cm}
   \leavevmode
 \includegraphics{/data/thesis/thesis_document/chapter5/figures/variable_plots/high_ratio/LT/mixed/All_chimax_15._SNcategory_0_to_5_20_05_08_LT_mixed_chisq_log_P_histogram_030.eps} \\
\vspace*{5cm}
   \leavevmode
 \includegraphics{/data/thesis/thesis_document/chapter5/figures/variable_plots/high_ratio/PA/var/All_chimax_15._SNcategory_0_to_5_20_05_08_chisq_log_P_histogram_030.eps} \\
\vspace*{0cm}
   \leavevmode
 \includegraphics{/data/thesis/thesis_document/chapter5/figures/variable_plots/high_ratio/PA/mixed/All_chimax_15._SNcategory_0_to_5_20_05_08_mixed_chisq_log_P_histogram_030.eps} \\
  \end{tabular}
\hspace*{4cm}
  \begin{tabular}{ccc}
% 5 - whatever
\vspace*{5cm}
   \leavevmode
 \includegraphics{/data/thesis/thesis_document/chapter5/figures/variable_plots/high_ratio/LT/var/All_chimax_15._SNcategory_5_to_031_20_05_08_LT_chisq_log_P_histogram_030.eps} \\
 \vspace*{5cm}
   \leavevmode
\includegraphics{/data/thesis/thesis_document/chapter5/figures/variable_plots/high_ratio/LT/mixed/All_chimax_15._SNcategory_5_to_068_20_05_08_LT_mixed_chisq_log_P_histogram_030.eps} \\
\vspace*{5cm}
   \leavevmode
 \includegraphics{/data/thesis/thesis_document/chapter5/figures/variable_plots/high_ratio/PA/var/All_chimax_15._SNcategory_5_to_024_20_05_08_chisq_log_P_histogram_030.eps} \\
\vspace*{0cm}
   \leavevmode
 \includegraphics{/data/thesis/thesis_document/chapter5/figures/variable_plots/high_ratio/PA/mixed/All_chimax_15._SNcategory_5_to_017_20_05_08_mixed_chisq_log_P_histogram_030.eps} \\
  \end{tabular}
\hspace*{4cm}
  \begin{tabular}{ccc}
%% ALL amp categories.
\vspace*{5cm}
   \leavevmode
 \includegraphics{/data/thesis/thesis_document/chapter5/figures/variable_plots/high_ratio/LT/var/All_chimax_15._SNcategory_ALL_20_05_08_LT_chisq_log_P_histogram_030.eps} \\
\vspace*{5cm}
   \leavevmode
 \includegraphics{/data/thesis/thesis_document/chapter5/figures/variable_plots/high_ratio/LT/mixed/All_chimax_15._SNcategory_ALL_20_05_08_LT_mixed_chisq_log_P_histogram_030.eps} \\
\vspace*{5cm}
   \leavevmode
 \includegraphics{/data/thesis/thesis_document/chapter5/figures/variable_plots/high_ratio/PA/var/All_chimax_15._SNcategory_ALL_20_05_08_chisq_log_P_histogram_030.eps} \\
\vspace*{0cm}
   \leavevmode
 \includegraphics{/data/thesis/thesis_document/chapter5/figures/variable_plots/high_ratio/PA/mixed/All_chimax_15._SNcategory_ALL_20_05_08_mixed_chisq_log_P_histogram_030.eps} \\
  \end{tabular}
}
\caption[Histograms of variable lightcurve log(P) distributions: PA/LT flux ratio = 14.80 .]{Histograms of variable
 lightcurve log(P) distributions: PA/LT flux ratio = 14.80; Rows, top to bottom:
1)`variable' lightcurves containing (LT) or (LT + FTN) data only,
2) ``mixed'' lightcurves containing (LT) or (LT + FTN) data only,
3)`variable' lightcurves containing (PA + LT) or (PA + LT + FTN) data,
4) ``mixed'' lightcurves containing (PA + LT) or (PA + LT + FTN) data.
Columns, left to right: Flux amplitudes, 1) 0-5, 2) 5-`MAX' 3) Sum of all categories
`MAX' varies with row as: 1) 31 2) 68 3) 24 4) 17 .}
 \label{log(P)_all_categories_high_ratio}
\end{figure} 

\newpage

\begin{figure}
\vspace*{4cm}
\center{
  \begin{tabular}{ccc}
% 0-5
\vspace*{5cm}
   \leavevmode
 \includegraphics{/data/thesis/thesis_document/chapter5/figures/variable_plots/high_ratio/LT/var/All_chimax_15._SNcategory_0_to_5_20_05_08_LT_chisq_skew_histogram_020.eps} \\
\vspace*{5cm}
   \leavevmode
 \includegraphics{/data/thesis/thesis_document/chapter5/figures/variable_plots/high_ratio/LT/mixed/All_chimax_15._SNcategory_0_to_5_20_05_08_LT_mixed_chisq_skew_histogram_020.eps} \\
\vspace*{5cm}
   \leavevmode
 \includegraphics{/data/thesis/thesis_document/chapter5/figures/variable_plots/high_ratio/PA/var/All_chimax_15._SNcategory_0_to_5_20_05_08_chisq_skew_histogram_020.eps} \\
\vspace*{0cm}
   \leavevmode
 \includegraphics{/data/thesis/thesis_document/chapter5/figures/variable_plots/high_ratio/PA/mixed/All_chimax_15._SNcategory_0_to_5_20_05_08_mixed_chisq_skew_histogram_020.eps} \\
  \end{tabular}
 %}
\hspace*{4cm}
  \begin{tabular}{ccc}
% 5 - whatever
\vspace*{5cm}
   \leavevmode
 \includegraphics{/data/thesis/thesis_document/chapter5/figures/variable_plots/high_ratio/LT/var/All_chimax_15._SNcategory_5_to_031_20_05_08_LT_chisq_skew_histogram_020.eps} \\
 \vspace*{5cm}
   \leavevmode
\includegraphics{/data/thesis/thesis_document/chapter5/figures/variable_plots/high_ratio/LT/mixed/All_chimax_15._SNcategory_5_to_068_20_05_08_LT_mixed_chisq_skew_histogram_020.eps} \\
\vspace*{5cm}
   \leavevmode
 \includegraphics{/data/thesis/thesis_document/chapter5/figures/variable_plots/high_ratio/PA/var/All_chimax_15._SNcategory_5_to_024_20_05_08_chisq_skew_histogram_020.eps} \\
\vspace*{0cm}
   \leavevmode
 \includegraphics{/data/thesis/thesis_document/chapter5/figures/variable_plots/high_ratio/PA/mixed/All_chimax_15._SNcategory_5_to_017_20_05_08_mixed_chisq_skew_histogram_020.eps} \\
  \end{tabular}
\hspace*{4cm}
  \begin{tabular}{ccc}
%% ALL amp categories.
\vspace*{5cm}
   \leavevmode
 \includegraphics{/data/thesis/thesis_document/chapter5/figures/variable_plots/high_ratio/LT/var/All_chimax_15._SNcategory_ALL_20_05_08_LT_chisq_skew_histogram_020.eps} \\
\vspace*{5cm}
   \leavevmode
 \includegraphics{/data/thesis/thesis_document/chapter5/figures/variable_plots/high_ratio/LT/mixed/All_chimax_15._SNcategory_ALL_20_05_08_LT_mixed_chisq_skew_histogram_020.eps} \\
\vspace*{5cm}
   \leavevmode
 \includegraphics{/data/thesis/thesis_document/chapter5/figures/variable_plots/high_ratio/PA/var/All_chimax_15._SNcategory_ALL_20_05_08_chisq_skew_histogram_020.eps} \\
\vspace*{0cm}
   \leavevmode
 \includegraphics{/data/thesis/thesis_document/chapter5/figures/variable_plots/high_ratio/PA/mixed/All_chimax_15._SNcategory_ALL_20_05_08_mixed_chisq_skew_histogram_020.eps} \\
  \end{tabular}
}
\caption[Histograms of variable lightcurve Skewness distributions: PA/LT flux ratio = 14.80 .]{Histograms of variable
 lightcurve Skewness distributions: PA/LT flux ratio = 14.80 ; Rows, top to bottom:
1)`variable' lightcurves containing (LT) or (LT + FTN) data only,
2) ``mixed'' lightcurves containing (LT) or (LT + FTN) data only,
3)`variable' lightcurves containing (PA + LT) or (PA + LT + FTN) data,
4) ``mixed'' lightcurves containing (PA + LT) or (PA + LT + FTN) data.
Columns, left to right: Flux amplitudes, 1) 0-5, 2) 5-`MAX' 3) Sum of all categories
`MAX' varies with row as: 1) 31 2) 68 3) 24 4) 17 .}
 \label{Skewness_all_categories_high_ratio}
\end{figure}

% NO FIXED RATIO
\newpage

\begin{figure}
\vspace*{4cm}
\center{
  \begin{tabular}{ccc}
% 0-5
\vspace*{5cm}
   \leavevmode
 \includegraphics{/data/thesis/thesis_document/chapter5/figures/variable_plots/no_ratio/LT/var/All_chimax_15._SNcategory_0_to_5_12_04_08_LT_chisq_log_P_histogram_030.eps} \\
\vspace*{5cm}
   \leavevmode
 \includegraphics{/data/thesis/thesis_document/chapter5/figures/variable_plots/no_ratio/LT/mixed/All_chimax_15._SNcategory_0_to_5_12_04_08_LT_mixed_chisq_log_P_histogram_030.eps} \\
\vspace*{5cm}
   \leavevmode
 \includegraphics{/data/thesis/thesis_document/chapter5/figures/variable_plots/no_ratio/PA/var/All_chimax_15._SNcategory_0_to_5_12_04_08_chisq_log_P_histogram_030.eps} \\
\vspace*{0cm}
   \leavevmode
 \includegraphics{/data/thesis/thesis_document/chapter5/figures/variable_plots/no_ratio/PA/mixed/All_chimax_15._SNcategory_0_to_5_12_04_08_mixed_chisq_log_P_histogram_030.eps} \\
  \end{tabular}
\hspace*{4cm}
  \begin{tabular}{ccc}
% 5 - whatever
\vspace*{5cm}
   \leavevmode
 \includegraphics{/data/thesis/thesis_document/chapter5/figures/variable_plots/no_ratio/LT/var/All_chimax_15._SNcategory_5_to_031_12_04_08_LT_chisq_log_P_histogram_030.eps} \\
 \vspace*{5cm}
   \leavevmode
\includegraphics{/data/thesis/thesis_document/chapter5/figures/variable_plots/no_ratio/LT/mixed/All_chimax_15._SNcategory_5_to_035_12_04_08_LT_mixed_chisq_log_P_histogram_030.eps} \\
\vspace*{5cm}
   \leavevmode
 \includegraphics{/data/thesis/thesis_document/chapter5/figures/variable_plots/no_ratio/PA/var/All_chimax_15._SNcategory_5_to_023_12_04_08_chisq_log_P_histogram_030.eps} \\
\vspace*{0cm}
   \leavevmode
 \includegraphics{/data/thesis/thesis_document/chapter5/figures/variable_plots/no_ratio/PA/mixed/All_chimax_15._SNcategory_5_to_078_12_04_08_mixed_chisq_log_P_histogram_030.eps} \\
  \end{tabular}
\hspace*{4cm}
  \begin{tabular}{ccc}
%% ALL amp categories.
\vspace*{5cm}
   \leavevmode
 \includegraphics{/data/thesis/thesis_document/chapter5/figures/variable_plots/no_ratio/LT/var/All_chimax_15._SNcategory_ALL_12_04_08_LT_chisq_log_P_histogram_030.eps} \\
\vspace*{5cm}
   \leavevmode
 \includegraphics{/data/thesis/thesis_document/chapter5/figures/variable_plots/no_ratio/LT/mixed/All_chimax_15._SNcategory_ALL_12_04_08_LT_mixed_chisq_log_P_histogram_030.eps} \\
\vspace*{5cm}
   \leavevmode
 \includegraphics{/data/thesis/thesis_document/chapter5/figures/variable_plots/no_ratio/PA/var/All_chimax_15._SNcategory_ALL_12_04_08_chisq_log_P_histogram_030.eps} \\
\vspace*{0cm}
   \leavevmode
 \includegraphics{/data/thesis/thesis_document/chapter5/figures/variable_plots/no_ratio/PA/mixed/All_chimax_15._SNcategory_ALL_12_04_08_mixed_chisq_log_P_histogram_030.eps} \\
  \end{tabular}
}
\caption[Histograms of variable lightcurve log(P) distributions: No fixed PA/LT flux ratio.]{Histograms of variable
 lightcurve log(P) distributions: No fixed PA/LT flux ratio ; Rows, top to bottom:
1)`variable' lightcurves containing (LT) or (LT + FTN) data only,
2) ``mixed'' lightcurves containing (LT) or (LT + FTN) data only,
3)`variable' lightcurves containing (PA + LT) or (PA + LT + FTN) data,
4) ``mixed'' lightcurves containing (PA + LT) or (PA + LT + FTN) data.
Columns, left to right: Flux amplitudes, 1) 0-5, 2) 5-`MAX' 3) Sum of all categories
`MAX' varies with row as: 1) 31 2) 35 3) 23 4) 78 .}
 \label{log(P)_all_categories_no_ratio}
\end{figure} 

%NO RATIO SKEW

\newpage

\begin{figure}
\vspace*{4cm}
\center{
  \begin{tabular}{ccc}
% 0-5
\vspace*{5cm}
   \leavevmode
 \includegraphics{/data/thesis/thesis_document/chapter5/figures/variable_plots/low_ratio/LT/var/All_chimax_15._SNcategory_0_to_5_08_06_08_LT_chisq_skew_histogram_020.eps} \\
\vspace*{5cm}
   \leavevmode
 \includegraphics{/data/thesis/thesis_document/chapter5/figures/variable_plots/low_ratio/LT/mixed/All_chimax_15._SNcategory_0_to_5_08_06_08_LT_mixed_chisq_skew_histogram_020.eps} \\
\vspace*{5cm}
   \leavevmode
 \includegraphics{/data/thesis/thesis_document/chapter5/figures/variable_plots/low_ratio/PA/var/All_chimax_15._SNcategory_0_to_5_08_06_08_chisq_skew_histogram_020.eps} \\
\vspace*{0cm}
   \leavevmode
 \includegraphics{/data/thesis/thesis_document/chapter5/figures/variable_plots/low_ratio/PA/mixed/All_chimax_15._SNcategory_0_to_5_08_06_08_mixed_chisq_skew_histogram_020.eps} \\
  \end{tabular}
\hspace*{4cm}
  \begin{tabular}{ccc}
% 5 - whatever
\vspace*{5cm}
   \leavevmode
 \includegraphics{/data/thesis/thesis_document/chapter5/figures/variable_plots/low_ratio/LT/var/All_chimax_15._SNcategory_5_to_031_08_06_08_LT_chisq_skew_histogram_020.eps} \\
 \vspace*{5cm}
   \leavevmode
\includegraphics{/data/thesis/thesis_document/chapter5/figures/variable_plots/low_ratio/LT/mixed/All_chimax_15._SNcategory_5_to_068_08_06_08_LT_mixed_chisq_skew_histogram_020.eps} \\
\vspace*{5cm}
   \leavevmode
 \includegraphics{/data/thesis/thesis_document/chapter5/figures/variable_plots/low_ratio/PA/var/All_chimax_15._SNcategory_5_to_032_08_06_08_chisq_skew_histogram_020.eps} \\
\vspace*{0cm}
   \leavevmode
 \includegraphics{/data/thesis/thesis_document/chapter5/figures/variable_plots/low_ratio/PA/mixed/All_chimax_15._SNcategory_5_to_032_08_06_08_mixed_chisq_skew_histogram_020.eps} \\
  \end{tabular}
\hspace*{4cm}
  \begin{tabular}{ccc}
%% ALL amp categories.
\vspace*{5cm}
   \leavevmode
 \includegraphics{/data/thesis/thesis_document/chapter5/figures/variable_plots/low_ratio/LT/var/All_chimax_15._SNcategory_ALL_08_06_08_LT_chisq_skew_histogram_020.eps} \\
\vspace*{5cm}
   \leavevmode
 \includegraphics{/data/thesis/thesis_document/chapter5/figures/variable_plots/low_ratio/LT/mixed/All_chimax_15._SNcategory_ALL_08_06_08_LT_mixed_chisq_skew_histogram_020.eps} \\
\vspace*{5cm}
   \leavevmode
 \includegraphics{/data/thesis/thesis_document/chapter5/figures/variable_plots/low_ratio/PA/var/All_chimax_15._SNcategory_ALL_08_06_08_chisq_skew_histogram_020.eps} \\
\vspace*{0cm}
   \leavevmode
 \includegraphics{/data/thesis/thesis_document/chapter5/figures/variable_plots/low_ratio/PA/mixed/All_chimax_15._SNcategory_ALL_08_06_08_mixed_chisq_skew_histogram_020.eps} \\
  \end{tabular}
}
\caption[Histograms of variable lightcurve Skewness distributions: No fixed PA/LT flux ratio. ]{Histograms of variable
 lightcurve Skewness distributions: No fixed PA/LT flux ratio ; Rows, top to bottom:
1)`variable' lightcurves containing (LT) or (LT + FTN) data only,
2) ``mixed'' lightcurves containing (LT) or (LT + FTN) data only,
3)`variable' lightcurves containing (PA + LT) or (PA + LT + FTN) data,
4) ``mixed'' lightcurves containing (PA + LT) or (PA + LT + FTN) data.
Columns, left to right: Flux amplitudes, 1) 0-5, 2) 5-`MAX' 3) Sum of all categories
`MAX' varies with row as: 1) 31 2) 35 3) 23 4) 78 .}
 \label{Skewness_all_categories_no_ratio}
\end{figure}
